# Supplementary material for: Automated Customized Bug-Benchmark Generation
Source: arXiv:1901.02819 source file (2019-09-06)
Supplement: Supplementary file 1 [file scion-appendix.tex]

\section{Bug Template Definitions}
\label{bug-template-definitions}

In this appendix, we provide the definitions for all the bug templates
listed in~Table 5, in the same order that they appear in the table.

\subsection*{Bug Template {\tt CLANG-BUFFER1}}
\begin{description}
\item[Definition:]~\newline
\begin{lstlisting}[language=lisp]
(define-scion clang-buffer1
    (make-instance 'clang-scion
                   :name 'clang-buffer1
                   :patches (list clang-buffer1-patch)))
\end{lstlisting}
\item[Patches:]~
\begin{itemize}
\item Definition for patch {\tt CLANG-BUFFER1-PATCH}.
\begin{lstlisting}[language=lisp]
(defparameter clang-buffer1-patch
  (make-instance 'clang-dynamic-patch
    :precondition nil
    :cwe 122
    :cwe-line 3
    :free-variables '(("s" "*char" :-const) ("c" "char" :-const))
    :code "s = \"\";
/* POTENTIAL FLAW */
c = s[1];
c++;"))
\end{lstlisting}
\end{itemize}
\end{description}

\subsection*{Bug Template {\tt CLANG-BUFFER2}}
\begin{description}
\item[Definition:]~\newline
\begin{lstlisting}[language=lisp]
(define-scion clang-buffer2
    (make-instance 'clang-scion
                   :name 'clang-buffer2
                   :patches (list clang-buffer2-patch)))
\end{lstlisting}
\item[Patches:]~
\begin{itemize}
\item Definition for patch {\tt CLANG-BUFFER2-PATCH}.
\begin{lstlisting}[language=lisp]
(defparameter clang-buffer2-patch
  (make-instance 'clang-dynamic-patch
    :cwe 121
    :cwe-line 3
    :precondition (lambda (obj location)
                    (vars-declarable-p obj
                                       (ast-at-index obj location)
                                       (list "s" "c")))
    :free-variables '()
    :code "char *s = \"\";
/* POTENTIAL FLAW */
char c = s[1];"))
\end{lstlisting}
\end{itemize}
\end{description}

\subsection*{Bug Template {\tt CLANG-BUFFER3}}
\begin{description}
\item[Definition:]~\newline
\begin{lstlisting}[language=lisp]
(define-scion clang-buffer3
    (make-instance 'clang-scion
                   :name 'clang-buffer3
                   :patches (list clang-buffer3-patch)))
\end{lstlisting}
\item[Patches:]~
\begin{itemize}
\item Definition for patch {\tt CLANG-BUFFER3-PATCH}.
\begin{lstlisting}[language=lisp]
(defparameter clang-buffer3-patch
  (make-instance 'clang-dynamic-patch
    :cwe 121
    :cwe-line 5
    :precondition (lambda (obj location)
                    (vars-declarable-p obj
                                       (ast-at-index obj location)
                                       (list "buf" "p")))
    :free-variables '()
    :code "int buf[100];
int *p = buf;
p = p + 99;
/* POTENTIAL FLAW */
p[1] = 1;"))
\end{lstlisting}
\end{itemize}
\end{description}

\subsection*{Bug Template {\tt CLANG-BUFFER4}}
\begin{description}
\item[Definition:]~\newline
\begin{lstlisting}[language=lisp]
(define-scion clang-buffer4
    (make-instance 'clang-scion
                   :name 'clang-buffer4
                   :patches (list clang-buffer4-patch)))
\end{lstlisting}
\item[Patches:]~
\begin{itemize}
\item Definition for patch {\tt CLANG-BUFFER4-PATCH}.
\begin{lstlisting}[language=lisp]
(defparameter clang-buffer4-patch
  (make-instance 'clang-dynamic-patch
    :cwe 121
    :cwe-line 5
    :precondition (lambda (obj location p)
                    (declare (ignorable p))
                    (var-declarable-p obj (ast-at-index obj location) "buf"))
    :free-variables '(("p" "*int" :-const))
    :code "int buf[100];
p = buf;
p = p + 99;
/* POTENTIAL FLAW */
p[1] = 1;"))
\end{lstlisting}
\end{itemize}
\end{description}

\subsection*{Bug Template {\tt CLANG-BUFFER5}}
\begin{description}
\item[Definition:]~\newline
\begin{lstlisting}[language=lisp]
(define-scion clang-buffer5
    (make-instance 'clang-scion
                   :name 'clang-buffer5
                   :patches (list clang-buffer5-patch)))
\end{lstlisting}
\item[Patches:]~
\begin{itemize}
\item Definition for patch {\tt CLANG-BUFFER5-PATCH}.
\begin{lstlisting}[language=lisp]
(defparameter clang-buffer5-patch
  (make-instance 'clang-dynamic-patch
    :cwe 121
    :cwe-line 3
    :precondition (lambda (obj location)
                    (var-declarable-p obj
                                      (ast-at-index obj location)
                                      "buf"))
    :free-variables '()
    :code "int buf[100][100];
/* POTENTIAL FLAW */
buf[0][-1] = 1;"))
\end{lstlisting}
\end{itemize}
\end{description}

\subsection*{Bug Template {\tt CLANG-BUFFER6}}
\begin{description}
\item[Definition:]~\newline
\begin{lstlisting}[language=lisp]
(define-scion clang-buffer6
    (make-instance 'clang-scion
                   :name 'clang-buffer6
                   :patches (list clang-buffer6-patch)))
\end{lstlisting}
\item[Patches:]~
\begin{itemize}
\item Definition for patch {\tt CLANG-BUFFER6-PATCH}.
\begin{lstlisting}[language=lisp]
(defparameter clang-buffer6-patch
  (make-instance 'clang-dynamic-patch
    :cwe 121
    :cwe-line 4
    :precondition (lambda (obj location p)
                    (declare (ignorable p))
                    (var-declarable-p obj (ast-at-index obj location) "buf"))
    :free-variables '(("p" "*int" :-const))
    :code "int buf[100][100];
p = &buf[0][-1];
/* POTENTIAL FLAW */
p[0] = 1;"))
\end{lstlisting}
\end{itemize}
\end{description}

\subsection*{Bug Template {\tt CLANG-BUFFER7}}
\begin{description}
\item[Definition:]~\newline
\begin{lstlisting}[language=lisp]
(define-scion clang-buffer7
    (make-instance 'clang-scion
                   :name 'clang-buffer7
                   :patches (list clang-buffer7-patch)))
\end{lstlisting}
\item[Patches:]~
\begin{itemize}
\item Definition for patch {\tt CLANG-BUFFER7-PATCH}.
\begin{lstlisting}[language=lisp]
(defparameter clang-buffer7-patch
  (make-instance 'clang-dynamic-patch
    :cwe 122
    :cwe-line 2
    :precondition (lambda (obj location n p)
                    (declare (ignorable obj location p))
                    (> (* (v/value n) 4) +max-int-32+))
    :free-variables '(("n" "int") ("p" "*void" :-const))
    :code "/* POTENTIAL FLAW */
p = malloc(n * sizeof(int));"))
\end{lstlisting}
\end{itemize}
\end{description}

\subsection*{Bug Template {\tt CLANG-PD1}}
\begin{description}
\item[Definition:]~\newline
\begin{lstlisting}[language=lisp]
(define-scion clang-pd1
    (make-instance 'clang-scion
                   :name 'clang-pd1
                   :patches (list clang-pd1-patch)))
\end{lstlisting}
\item[Patches:]~
\begin{itemize}
\item Definition for patch {\tt CLANG-PD1-PATCH}.
\begin{lstlisting}[language=lisp]
(defparameter clang-pd1-patch
  (make-instance 'clang-dynamic-patch
    :cwe 476
    :cwe-line 5
    :precondition (lambda (obj location p)
                    (let ((ast (ast-at-index obj location)))
                      (and (= (v/value p) 0)
                           (ast-void-ret (function-containing-ast obj ast))
                           (var-declarable-p obj ast "x"))))
    :free-variables '(("p" "*int"))
    :code "if (p) {
    return;
}
/* POTENTIAL FLAW */
int x = p[0];"))
\end{lstlisting}
\end{itemize}
\end{description}

\subsection*{Bug Template {\tt CLANG-PD2}}
\begin{description}
\item[Definition:]~\newline
\begin{lstlisting}[language=lisp]
(define-scion clang-pd2
    (make-instance 'clang-scion
                   :name 'clang-pd2
                   :patches (list clang-pd2-patch)))
\end{lstlisting}
\item[Patches:]~
\begin{itemize}
\item Definition for patch {\tt CLANG-PD2-PATCH}.
\begin{lstlisting}[language=lisp]
(defparameter clang-pd2-patch
  (make-instance 'clang-dynamic-patch
    :cwe 476
    :cwe-line 3
    :precondition (lambda (obj location p)
                    (declare (ignorable obj location))
                    (= (v/value p) 0))
    :free-variables '(("p" "*int" :-const))
    :code "if (!p) {
    /* POTENTIAL FLAW */
    *p = 0;
}"))
\end{lstlisting}
\end{itemize}
\end{description}

\subsection*{Bug Template {\tt CLANG-PD3}}
\begin{description}
\item[Definition:]~\newline
\begin{lstlisting}[language=lisp]
(define-scion clang-pd3
    (make-instance 'clang-scion
                   :name 'clang-pd3
                   :patches (list clang-pd3-patch)))
\end{lstlisting}
\item[Patches:]~
\begin{itemize}
\item Definition for patch {\tt CLANG-PD3-PATCH}.
\begin{lstlisting}[language=lisp]
(defparameter clang-pd3-patch
  (make-instance 'clang-dynamic-patch
    :cwe 476
    :cwe-line 2
    :precondition  nil
    :free-variables '()
    :includes '("<string.h>")
    :code "/* POTENTIAL FLAW */
strlen(0);"))
\end{lstlisting}
\end{itemize}
\end{description}

\subsection*{Bug Template {\tt CLANG-PD4}}
\begin{description}
\item[Definition:]~\newline
\begin{lstlisting}[language=lisp]
(define-scion clang-pd4
    (make-instance 'clang-scion
                   :name 'clang-pd4
                   :patches (list clang-pd4-patch)))
\end{lstlisting}
\item[Patches:]~
\begin{itemize}
\item Definition for patch {\tt CLANG-PD4-PATCH}.
\begin{lstlisting}[language=lisp]
(defparameter clang-pd4-patch
  (make-instance 'clang-dynamic-patch
    :cwe 476
    :cwe-line 2
    :precondition (lambda (obj location x)
                    (declare (ignorable obj location))
                    (= (v/value x) 0))
    :free-variables '(("x" "*char"))
    :includes '("<string.h>")
    :code "/* POTENTIAL FLAW */
strlen(x);"))
\end{lstlisting}
\end{itemize}
\end{description}

\subsection*{Bug Template {\tt INFER-BUFFER1}}
\begin{description}
\item[Definition:]~\newline
\begin{lstlisting}[language=lisp]
(define-scion infer-buffer1
    (make-instance 'clang-scion
                   :name 'infer-buffer1
                   :patches (list infer-buffer1-patch1
                                  infer-buffer1-patch2)))
\end{lstlisting}
\item[Patches:]~
\begin{itemize}
\item Definition for patch {\tt INFER-BUFFER1-PATCH1}.
\begin{lstlisting}[language=lisp]
(defparameter infer-buffer1-patch1
  (make-instance 'clang-static-patch
    :precondition (lambda (obj location)
                    (declare (ignorable obj))
                    (= location 0))
    :free-variables nil
    :code-top-level-p t
    :code "void set_i(int *arr, int index) {
  arr[index] = 0;
}"))
\end{lstlisting}
\item Definition for patch {\tt INFER-BUFFER1-PATCH2}.
\begin{lstlisting}[language=lisp]
(defparameter infer-buffer1-patch2
  (make-instance 'clang-dynamic-patch
    :cwe 122
    :cwe-line 7
    :precondition nil
    :free-variables '(("arr" "*int" :-const))
    :dependencies (list infer-buffer1-patch1)
    :includes (list "<stdlib.h>")
    :code "arr = (int *)malloc(9*sizeof(int));
if (arr != NULL) {
    int i;
    for (i = 0; i < 9; i+=1) {
        set_i(arr, i);
        /* POTENTIAL FLAW */
        set_i(arr, i + 1);
    }
}"))
\end{lstlisting}
\end{itemize}
\end{description}

\subsection*{Bug Template {\tt INFER-BUFFER2}}
\begin{description}
\item[Definition:]~\newline
\begin{lstlisting}[language=lisp]
(define-scion infer-buffer2
    (make-instance 'clang-scion
                   :name 'infer-buffer2
                   :patches (list infer-buffer2-patch)))
\end{lstlisting}
\item[Patches:]~
\begin{itemize}
\item Definition for patch {\tt INFER-BUFFER2-PATCH}.
\begin{lstlisting}[language=lisp]
(defparameter infer-buffer2-patch
  (make-instance 'clang-dynamic-patch
    :cwe 122
    :cwe-line 7
    :precondition nil
    :free-variables '(("arr" "*int" :-const))
    :includes '("<stdlib.h>")
    :code "arr = (int *)malloc(9*sizeof(int));
if (arr != NULL) {
    int i;
    for (i = 0; i < 9; i++) {
        arr[i] = 0;
        /* POTENTIAL FLAW */
        arr[i+1] = 0;
    }
}"))
\end{lstlisting}
\end{itemize}
\end{description}

\subsection*{Bug Template {\tt INFER-BUFFER3}}
\begin{description}
\item[Definition:]~\newline
\begin{lstlisting}[language=lisp]
(define-scion infer-buffer3
    (make-instance 'clang-scion
                   :name 'infer-buffer3
                   :patches (list infer-buffer3-patch)))
\end{lstlisting}
\item[Patches:]~
\begin{itemize}
\item Definition for patch {\tt INFER-BUFFER3-PATCH}.
\begin{lstlisting}[language=lisp]
(defparameter infer-buffer3-patch
  (make-instance 'clang-dynamic-patch
    :cwe 121
    :cwe-line 4
    :precondition (lambda (obj location global)
                    (and (< (v/value global) 10)
                            (var-declarable-p obj
                                              (ast-at-index obj location)
                                              "arr")))
    :free-variables '(("global" "int"))
    :code "char arr[10];
if (global < 10){
    /* POTENTIAL FLAW */
    arr[10] = 1;
}"))
\end{lstlisting}
\end{itemize}
\end{description}

\subsection*{Bug Template {\tt INFER-BUFFER4}}
\begin{description}
\item[Definition:]~\newline
\begin{lstlisting}[language=lisp]
(define-scion infer-buffer4
    (make-instance 'clang-scion
                   :name 'infer-buffer4
                   :patches (list infer-buffer4-patch1
                                  infer-buffer4-patch2)))
\end{lstlisting}
\item[Patches:]~
\begin{itemize}
\item Definition for patch {\tt INFER-BUFFER4-PATCH1}.
\begin{lstlisting}[language=lisp]
(defparameter infer-buffer4-patch1
  (make-instance 'clang-static-patch
    :precondition (lambda (obj location)
                    (declare (ignorable obj))
                    (= location 0))
    :free-variables '()
    :code-top-level-p t
    :code "void two_accesses(int* arr) {
    if (arr[1] < 0) {
        arr[0] = 0;
    }
}"))
\end{lstlisting}
\item Definition for patch {\tt INFER-BUFFER4-PATCH2}.
\begin{lstlisting}[language=lisp]
(defparameter infer-buffer4-patch2
  (make-instance 'clang-dynamic-patch
    :cwe 122
    :cwe-line 2
    :precondition (lambda (obj location arr)
                    (declare (ignorable obj location))
                    (and (v/size arr)
                         (<= (v/size arr) 4)))
    :free-variables '(("arr" "*int" :-const))
    :dependencies (list infer-buffer4-patch1)
    :code "/* POTENTIAL FLAW */
two_accesses(arr);"))
\end{lstlisting}
\end{itemize}
\end{description}

\subsection*{Bug Template {\tt INFER-BUFFER5}}
\begin{description}
\item[Definition:]~\newline
\begin{lstlisting}[language=lisp]
(define-scion infer-buffer5
    (make-instance 'clang-scion
                   :name 'infer-buffer5
                   :patches (list infer-buffer5-patch)))
\end{lstlisting}
\item[Patches:]~
\begin{itemize}
\item Definition for patch {\tt INFER-BUFFER5-PATCH}.
\begin{lstlisting}[language=lisp]
(defparameter infer-buffer5-patch
  (make-instance 'clang-dynamic-patch
    :cwe 121
    :cwe-line 4
    :precondition (lambda (obj location n)
                    (and (= (v/value n) 0)
                         (var-declarable-p obj
                                           (ast-at-index obj location)
                                           "arr")))
    :free-variables '(("n" "int"))
    :code "int arr[1];
arr[n] = 0;
/* POTENTIAL FLAW */
arr[n - 2] = 0;"))
\end{lstlisting}
\end{itemize}
\end{description}

\subsection*{Bug Template {\tt INFER-PD1}}
\begin{description}
\item[Definition:]~\newline
\begin{lstlisting}[language=lisp]
(define-scion infer-pd1
    (make-instance 'clang-scion
                   :name 'infer-pd1
                   :patches (list infer-pd1-patch1
                                  infer-pd1-patch2)))
\end{lstlisting}
\item[Patches:]~
\begin{itemize}
\item Definition for patch {\tt INFER-PD1-PATCH1}.
\begin{lstlisting}[language=lisp]
(defparameter infer-pd1-patch1
  (make-instance 'clang-static-patch
    :precondition (lambda (obj location)
                    (declare (ignorable obj))
                    (= location 0))
    :code-top-level-p t
    :code "void set_ptr(int* ptr, int val) {
    *ptr = val;
}
int set_ptr_param_array(int buf[]) {
    set_ptr(buf, 1);
    return buf[0];
}"))
\end{lstlisting}
\item Definition for patch {\tt INFER-PD1-PATCH2}.
\begin{lstlisting}[language=lisp]
(defparameter infer-pd1-patch2
  (make-instance 'clang-dynamic-patch
    :cwe 476
    :cwe-line 2
    :dependencies (list infer-pd1-patch1)
    :code "/* POTENTIAL FLAW */
set_ptr_param_array(0);"))
\end{lstlisting}
\end{itemize}
\end{description}
