# Supplementary material for: Automated Customized Bug-Benchmark Generation
Source: arXiv:1901.02819 source file (2019-09-06)
Supplement: Supplementary file 2 [file scion-appendix2.tex]

\subsection*{Bug Template {\tt CLANG-BUFFER5}}
\begin{description}
\item[Definition:]~\newline
\begin{lstlisting}[language=lisp]
(define-scion clang-buffer5
    (make-instance 'clang-scion
                   :name 'clang-buffer5
                   :patches (list clang-buffer5-patch1
                                  clang-buffer5-patch2)))
\end{lstlisting}
\item[Patches:]~
\begin{itemize}
\item Definition for patch {\tt CLANG-BUFFER5-PATCH1}.
\begin{lstlisting}[language=lisp]
(defparameter clang-buffer5-patch1
  (make-instance 'clang-static-patch
    :precondition (lambda (obj location)
                    (declare (ignorable obj))
                    (= location 0))
    :free-variables nil
    :code "static int A[10];"
    :code-top-level-p t))
\end{lstlisting}
\item Definition for patch {\tt CLANG-BUFFER5-PATCH2}.
\begin{lstlisting}[language=lisp]
(defparameter clang-buffer5-patch2
  (make-instance 'clang-dynamic-patch
    :cwe 122
    :cwe-line 3
    :precondition (lambda (obj location p)
                    (declare (ignorable p))
                    (when-let ((return-type
                                 (some->> (ast-at-index obj location)
                                          (function-containing-ast obj)
                                          (ast-ret)
                                          (find-type obj))))
                      (and (string= "int" (type-name return-type))
                           (type-pointer return-type))))
    :free-variables '(("p" "*int" :-const))
    :dependencies (list clang-buffer5-patch1)
    :code "p = A + 10;
/* POTENTIAL FLAW */
return p;"))
\end{lstlisting}
\end{itemize}
\end{description}

\subsection*{Bug Template {\tt CLANG-BUFFER5-TRIVIAL}}
\begin{description}
\item[Definition:]~\newline
\begin{lstlisting}[language=lisp]
(define-scion clang-buffer5-trivial
    (make-instance 'clang-scion
                   :name 'clang-buffer5-trivial
                   :patches (list clang-buffer5-patch1
                                  clang-buffer5-trivial-patch2)))
\end{lstlisting}
\item[Patches:]~
\begin{itemize}
\item Definition for patch {\tt CLANG-BUFFER5-PATCH1}.
\begin{lstlisting}[language=lisp]
(defparameter clang-buffer5-patch1
  (make-instance 'clang-static-patch
    :precondition (lambda (obj location)
                    (declare (ignorable obj))
                    (= location 0))
    :free-variables nil
    :code "static int A[10];"
    :code-top-level-p t))
\end{lstlisting}
\item Definition for patch {\tt CLANG-BUFFER5-TRIVIAL-PATCH2}.
\begin{lstlisting}[language=lisp]
(defparameter clang-buffer5-trivial-patch2
  (make-instance 'clang-dynamic-patch
    :cwe 122
    :cwe-line 3
    :precondition (lambda (obj location)
                    (when-let* ((ast (ast-at-index obj location))
                                (return-type (some->> (function-containing-ast
                                                        obj ast)
                                                      (ast-ret)
                                                      (find-type obj))))
                      (and (string= "int" (type-name return-type))
                           (type-pointer return-type)
                           (var-declarable-p obj ast "p"))))
    :free-variables '()
    :dependencies (list clang-buffer5-patch1)
    :code "int *p = A + 10;
/* POTENTIAL FLAW */
return p;"))
\end{lstlisting}
\end{itemize}
\end{description}

\subsection*{Bug Template {\tt CLANG-REGRESSION-TEST-BUFFER1}}
\begin{description}
\item[Definition:]~\newline
\begin{lstlisting}[language=lisp]
(define-scion clang-regression-test-buffer1
    (make-instance 'clang-scion
                   :name 'clang-regression-test-buffer1
                   :patches (list clang-regression-test-buffer1-patch)))
\end{lstlisting}
\item[Patches:]~
\begin{itemize}
\item Definition for patch {\tt CLANG-REGRESSION-TEST-BUFFER1-PATCH}.
\begin{lstlisting}[language=lisp]
(defparameter clang-regression-test-buffer1-patch
  (make-instance 'clang-dynamic-patch
    :cwe 122
    :cwe-line 3
    :precondition nil
    :free-variables '(("buf" "*char" :-const))
    :includes '("<stdlib.h>")
    :code "buf = (char*) malloc(2);
/* POTENTIAL FLAW */
buf[1] = 'c';"))
\end{lstlisting}
\end{itemize}
\end{description}

\subsection*{Bug Template {\tt CLANG-REGRESSION-TEST-BUFFER10}}
\begin{description}
\item[Definition:]~\newline
\begin{lstlisting}[language=lisp]
(define-scion clang-regression-test-buffer10
    (make-instance 'clang-scion
                   :name 'clang-regression-test-buffer10
                   :patches (list clang-regression-test-buffer10-patch)))
\end{lstlisting}
\item[Patches:]~
\begin{itemize}
\item Definition for patch {\tt CLANG-REGRESSION-TEST-BUFFER10-PATCH}.
\begin{lstlisting}[language=lisp]
(defparameter clang-regression-test-buffer10-patch
  (make-instance 'clang-dynamic-patch
    :cwe 121
    :cwe-line 3
    :precondition (lambda (obj location)
                    (var-declarable-p obj (ast-at-index obj location) "dest"))
    :free-variables '()
    :includes '("<string.h>")
    :code "char dest[10];
/* POTENTIAL FLAW */
strncat(dest, \"AAAAAAAAAAAAAAAAAAAAAAAAAAA\", sizeof(dest));"))
\end{lstlisting}
\end{itemize}
\end{description}

\subsection*{Bug Template {\tt CLANG-REGRESSION-TEST-BUFFER11}}
\begin{description}
\item[Definition:]~\newline
\begin{lstlisting}[language=lisp]
(define-scion clang-regression-test-buffer11
    (make-instance 'clang-scion
                   :name 'clang-regression-test-buffer11
                   :patches (list clang-regression-test-buffer11-patch)))
\end{lstlisting}
\item[Patches:]~
\begin{itemize}
\item Definition for patch {\tt CLANG-REGRESSION-TEST-BUFFER11-PATCH}.
\begin{lstlisting}[language=lisp]
(defparameter clang-regression-test-buffer11-patch
  (make-instance 'clang-dynamic-patch
    :cwe 121
    :cwe-line 3
    :precondition (lambda (obj location)
                    (var-declarable-p obj (ast-at-index obj location) "dest"))
    :free-variables '()
    :includes '("<string.h>")
    :code "char dest[10];
/* POTENTIAL FLAW */
strncat(dest, \"AAAAAAAAAAAAAAAAAAAAAAAAAAAAAAA\",
        sizeof(dest) - strlen(dest));"))
\end{lstlisting}
\end{itemize}
\end{description}

\subsection*{Bug Template {\tt CLANG-REGRESSION-TEST-BUFFER12}}
\begin{description}
\item[Definition:]~\newline
\begin{lstlisting}[language=lisp]
(define-scion clang-regression-test-buffer12
    (make-instance 'clang-scion
                   :name 'clang-regression-test-buffer12
                   :patches (list clang-regression-test-buffer12-patch)))
\end{lstlisting}
\item[Patches:]~
\begin{itemize}
\item Definition for patch {\tt CLANG-REGRESSION-TEST-BUFFER12-PATCH}.
\begin{lstlisting}[language=lisp]
(defparameter clang-regression-test-buffer12-patch
  (make-instance 'clang-dynamic-patch
    :cwe 121
    :cwe-line 3
    :precondition (lambda (obj location)
                    (let ((ast (ast-at-index obj location)))
                      (and (var-declarable-p obj ast "mystr")
                           (string= "char"
                                    (some->> (function-containing-ast obj ast)
                                             (ast-ret)
                                             (find-type obj)
                                             (type-trace-string))))))
    :free-variables '()
    :code "const char *mystr = \"mary had a little lamb\";
/* POTENTIAL FLAW */
return mystr[-1];"))
\end{lstlisting}
\end{itemize}
\end{description}

\subsection*{Bug Template {\tt CLANG-REGRESSION-TEST-BUFFER13}}
\begin{description}
\item[Definition:]~\newline
\begin{lstlisting}[language=lisp]
(define-scion clang-regression-test-buffer13
    (make-instance 'clang-scion
                   :name 'clang-regression-test-buffer13
                   :patches (list clang-regression-test-buffer13-patch)))
\end{lstlisting}
\item[Patches:]~
\begin{itemize}
\item Definition for patch {\tt CLANG-REGRESSION-TEST-BUFFER13-PATCH}.
\begin{lstlisting}[language=lisp]
(defparameter clang-regression-test-buffer13-patch
  (make-instance 'clang-dynamic-patch
    :cwe 121
    :cwe-line 3
    :precondition (lambda (obj location)
                    (let ((ast (ast-at-index obj location)))
                      (and (var-declarable-p obj ast "mystr")
                           (string= "char"
                                    (some->> (function-containing-ast obj ast)
                                             (ast-ret)
                                             (find-type obj)
                                             (type-trace-string))))))
    :free-variables '()
    :code "const char *mystr = \"mary had a little lamb\";
/* POTENTIAL FLAW */
return mystr[1000]; "))
\end{lstlisting}
\end{itemize}
\end{description}

\subsection*{Bug Template {\tt CLANG-REGRESSION-TEST-BUFFER14}}
\begin{description}
\item[Definition:]~\newline
\begin{lstlisting}[language=lisp]
(define-scion clang-regression-test-buffer14
    (make-instance 'clang-scion
                   :name 'clang-regression-test-buffer14
                   :patches (list clang-regression-test-buffer14-patch)))
\end{lstlisting}
\item[Patches:]~
\begin{itemize}
\item Definition for patch {\tt CLANG-REGRESSION-TEST-BUFFER14-PATCH}.
\begin{lstlisting}[language=lisp]
(defparameter clang-regression-test-buffer14-patch
  (make-instance 'clang-dynamic-patch
    :cwe 121
    :cwe-line 4
    :precondition (lambda (obj location)
                    (vars-declarable-p obj
                                       (ast-at-index obj location)
                                       '("buf" "p")))
    :free-variables '()
    :code "int buf[100];
int *p = buf;
/* POTENTIAL FLAW */
p[101] = 1; "))
\end{lstlisting}
\end{itemize}
\end{description}

\subsection*{Bug Template {\tt CLANG-REGRESSION-TEST-BUFFER15}}
\begin{description}
\item[Definition:]~\newline
\begin{lstlisting}[language=lisp]
(define-scion clang-regression-test-buffer15
    (make-instance 'clang-scion
                   :name 'clang-regression-test-buffer15
                   :patches (list clang-regression-test-buffer15-patch)))
\end{lstlisting}
\item[Patches:]~
\begin{itemize}
\item Definition for patch {\tt CLANG-REGRESSION-TEST-BUFFER15-PATCH}.
\begin{lstlisting}[language=lisp]
(defparameter clang-regression-test-buffer15-patch
  (make-instance 'clang-dynamic-patch
    :cwe 121
    :cwe-line 4
    :precondition (lambda (obj location)
                    (vars-declarable-p obj
                                       (ast-at-index obj location)
                                      '("buf" "p")))
    :free-variables '()
    :code "int buf[100];
int *p = buf;
/* POTENTIAL FLAW */
p[-1] = 1;"))
\end{lstlisting}
\end{itemize}
\end{description}

\subsection*{Bug Template {\tt CLANG-REGRESSION-TEST-BUFFER16}}
\begin{description}
\item[Definition:]~\newline
\begin{lstlisting}[language=lisp]
(define-scion clang-regression-test-buffer16
    (make-instance 'clang-scion
                   :name 'clang-regression-test-buffer16
                   :patches (list clang-regression-test-buffer16-patch)))
\end{lstlisting}
\item[Patches:]~
\begin{itemize}
\item Definition for patch {\tt CLANG-REGRESSION-TEST-BUFFER16-PATCH}.
\begin{lstlisting}[language=lisp]
(defparameter clang-regression-test-buffer16-patch
  (make-instance 'clang-dynamic-patch
    :cwe 121
    :cwe-line 5
    :precondition (lambda (obj location)
                    (vars-declarable-p obj
                                       (ast-at-index obj location)
                                       '("buf" "p")))
    :free-variables '()
    :code "int buf[100];
int *p = buf;
--p;
/* POTENTIAL FLAW */
p[0] = 1;"))
\end{lstlisting}
\end{itemize}
\end{description}

\subsection*{Bug Template {\tt CLANG-REGRESSION-TEST-BUFFER17}}
\begin{description}
\item[Definition:]~\newline
\begin{lstlisting}[language=lisp]
(define-scion clang-regression-test-buffer17
    (make-instance 'clang-scion
                   :name 'clang-regression-test-buffer17
                   :patches (list clang-regression-test-buffer17-patch)))
\end{lstlisting}
\item[Patches:]~
\begin{itemize}
\item Definition for patch {\tt CLANG-REGRESSION-TEST-BUFFER17-PATCH}.
\begin{lstlisting}[language=lisp]
(defparameter clang-regression-test-buffer17-patch
  (make-instance 'clang-dynamic-patch
    :cwe 121
    :cwe-line 4
    :precondition (lambda (obj location x)
                    (and (> (v/value x) 99)
                         (var-declarable-p obj
                                           (ast-at-index obj location)
                                           "buf")))
    :free-variables '(("x" "int"))
    :code "int buf[100];
if (x > 99) {
    /* POTENTIAL FLAW */
    buf[x] = 1;
}"))
\end{lstlisting}
\end{itemize}
\end{description}

\subsection*{Bug Template {\tt CLANG-REGRESSION-TEST-BUFFER18}}
\begin{description}
\item[Definition:]~\newline
\begin{lstlisting}[language=lisp]
(define-scion clang-regression-test-buffer18
    (make-instance 'clang-scion
                   :name 'clang-regression-test-buffer18
                   :patches (list clang-regression-test-buffer18-patch)))
\end{lstlisting}
\item[Patches:]~
\begin{itemize}
\item Definition for patch {\tt CLANG-REGRESSION-TEST-BUFFER18-PATCH}.
\begin{lstlisting}[language=lisp]
(defparameter clang-regression-test-buffer18-patch
  (make-instance 'clang-dynamic-patch
    :cwe 121
    :cwe-line 4
    :precondition (lambda (obj location x)
                    (and (< (v/value x) 0)
                         (var-declarable-p obj
                                           (ast-at-index obj location)
                                           "buf")))
    :free-variables '(("x" "int"))
    :code "int buf[100];
if (x < 0) {
    /* POTENTIAL FLAW */
    buf[x] = 1;
}"))
\end{lstlisting}
\end{itemize}
\end{description}

\subsection*{Bug Template {\tt CLANG-REGRESSION-TEST-BUFFER2}}
\begin{description}
\item[Definition:]~\newline
\begin{lstlisting}[language=lisp]
(define-scion clang-regression-test-buffer2
    (make-instance 'clang-scion
                   :name 'clang-regression-test-buffer2
                   :patches (list clang-regression-test-buffer2-patch)))
\end{lstlisting}
\item[Patches:]~
\begin{itemize}
\item Definition for patch {\tt CLANG-REGRESSION-TEST-BUFFER2-PATCH}.
\begin{lstlisting}[language=lisp]
(defparameter clang-regression-test-buffer2-patch
  (make-instance 'clang-dynamic-patch
    :cwe 122
    :cwe-line 3
    :precondition nil
    :free-variables '(("p" "*int" :-const))
    :includes '("<stdlib.h>")
    :code "p = (int*) malloc(12);
/* POTENTIAL FLAW */
p[3] = 4;"))
\end{lstlisting}
\end{itemize}
\end{description}

\subsection*{Bug Template {\tt CLANG-REGRESSION-TEST-BUFFER3}}
\begin{description}
\item[Definition:]~\newline
\begin{lstlisting}[language=lisp]
(define-scion clang-regression-test-buffer3
    (make-instance 'clang-scion
                   :name 'clang-regression-test-buffer3
                   :patches (list clang-regression-test-buffer3-patch)))
\end{lstlisting}
\item[Patches:]~
\begin{itemize}
\item Definition for patch {\tt CLANG-REGRESSION-TEST-BUFFER3-PATCH}.
\begin{lstlisting}[language=lisp]
(defparameter clang-regression-test-buffer3-patch
  (make-instance 'clang-dynamic-patch
    :cwe 122
    :cwe-line 4
    :precondition nil
    :free-variables '(("p" "*char" :-const))
    :includes '("<stdlib.h>")
    :code "p = (char*) calloc(2,2);
p[3] = '.';
/* POTENTIAL FLAW */
p[4] = '!';"))
\end{lstlisting}
\end{itemize}
\end{description}

\subsection*{Bug Template {\tt CLANG-REGRESSION-TEST-BUFFER4}}
\begin{description}
\item[Definition:]~\newline
\begin{lstlisting}[language=lisp]
(define-scion clang-regression-test-buffer4
    (make-instance 'clang-scion
                   :name 'clang-regression-test-buffer4
                   :patches (list clang-regression-test-buffer4-patch)))
\end{lstlisting}
\item[Patches:]~
\begin{itemize}
\item Definition for patch {\tt CLANG-REGRESSION-TEST-BUFFER4-PATCH}.
\begin{lstlisting}[language=lisp]
(defparameter clang-regression-test-buffer4-patch
  (make-instance 'clang-dynamic-patch
    :cwe 121
    :cwe-line 4
    :precondition (lambda (obj location)
                    (vars-declarable-p obj
                                       (ast-at-index obj location)
                                       '("a" "b")))
    :free-variables '()
    :code "char a[2];
int *b = (int*)a;
/* POTENTIAL FLAW */
b[1] = 3;"))
\end{lstlisting}
\end{itemize}
\end{description}

\subsection*{Bug Template {\tt CLANG-REGRESSION-TEST-BUFFER5}}
\begin{description}
\item[Definition:]~\newline
\begin{lstlisting}[language=lisp]
(define-scion clang-regression-test-buffer5
    (make-instance 'clang-scion
                   :name 'clang-regression-test-buffer5
                   :patches (list clang-regression-test-buffer5-patch)))
\end{lstlisting}
\item[Patches:]~
\begin{itemize}
\item Definition for patch {\tt CLANG-REGRESSION-TEST-BUFFER5-PATCH}.
\begin{lstlisting}[language=lisp]
(defparameter clang-regression-test-buffer5-patch
  (make-instance 'clang-dynamic-patch
    :cwe 121
    :cwe-line 5
    :precondition (lambda (obj location a)
                    (declare (ignorable obj location))
                    (= (v/value a) 5))
    :free-variables '(("a" "int"))
    :code "if (a == 5) {
    int x[a];
    x[4] = 4;
    /* POTENTIAL FLAW */
    x[5] = 5;
}"))
\end{lstlisting}
\end{itemize}
\end{description}

\subsection*{Bug Template {\tt CLANG-REGRESSION-TEST-BUFFER6}}
\begin{description}
\item[Definition:]~\newline
\begin{lstlisting}[language=lisp]
(define-scion clang-regression-test-buffer6
    (make-instance 'clang-scion
                   :name 'clang-regression-test-buffer6
                   :patches (list clang-regression-test-buffer6-patch)))
\end{lstlisting}
\item[Patches:]~
\begin{itemize}
\item Definition for patch {\tt CLANG-REGRESSION-TEST-BUFFER6-PATCH}.
\begin{lstlisting}[language=lisp]
(defparameter clang-regression-test-buffer6-patch
  (make-instance 'clang-dynamic-patch
    :cwe 121
    :cwe-line 4
    :precondition (lambda (obj location a)
                    (let ((ast (ast-at-index obj location)))
                      (and (= (v/value a) 2)
                           (equal "int"
                                  (some->> (function-containing-ast obj ast)
                                           (ast-ret)
                                           (find-type obj)
                                           (type-trace-string)))
                           (var-declarable-p obj ast "x"))))
    :free-variables '(("a" "int"))
    :code "int x[2];
if (a == 2) {
    /* POTENTIAL FLAW */
    return x[a];
}"))
\end{lstlisting}
\end{itemize}
\end{description}

\subsection*{Bug Template {\tt CLANG-REGRESSION-TEST-BUFFER7}}
\begin{description}
\item[Definition:]~\newline
\begin{lstlisting}[language=lisp]
(define-scion clang-regression-test-buffer7
    (make-instance 'clang-scion
                   :name 'clang-regression-test-buffer7
                   :patches (list clang-regression-test-buffer7-patch)))
\end{lstlisting}
\item[Patches:]~
\begin{itemize}
\item Definition for patch {\tt CLANG-REGRESSION-TEST-BUFFER7-PATCH}.
\begin{lstlisting}[language=lisp]
(defparameter clang-regression-test-buffer7-patch
  (make-instance 'clang-dynamic-patch
    :cwe 121
    :cwe-line 4
    :precondition (lambda (obj location a)
                    (let ((ast (ast-at-index obj location)))
                      (and (< (v/value a) 0)
                           (equal "int"
                                  (some->> (function-containing-ast obj ast)
                                           (ast-ret)
                                           (find-type obj)
                                           (type-trace-string)))
                           (var-declarable-p obj ast "x"))))
    :free-variables '(("a" "int"))
    :code "int x[2];
if (a < 0) {
    /* POTENTIAL FLAW */
    return x[a];
}"))
\end{lstlisting}
\end{itemize}
\end{description}

\subsection*{Bug Template {\tt CLANG-REGRESSION-TEST-BUFFER8}}
\begin{description}
\item[Definition:]~\newline
\begin{lstlisting}[language=lisp]
(define-scion clang-regression-test-buffer8
    (make-instance 'clang-scion
                   :name 'clang-regression-test-buffer8
                   :patches (list clang-regression-test-buffer8-patch)))
\end{lstlisting}
\item[Patches:]~
\begin{itemize}
\item Definition for patch {\tt CLANG-REGRESSION-TEST-BUFFER8-PATCH}.
\begin{lstlisting}[language=lisp]
(defparameter clang-regression-test-buffer8-patch
  (make-instance 'clang-dynamic-patch
    :cwe 121
    :cwe-line 30
    :precondition (lambda (obj location in)
                     (and (> (v/value in) 1E-8)
                          (< (v/value in) 1E+23)
                          (var-declarable-p obj
                                            (ast-at-index obj location)
                                            "eee")))
    :free-variables '(("in" "double"))
    :code "int eee = 16;
  if (in < 1e-8 || in > 1e23) {
    return 0;
  } else {
    static const double ins[] = {1e-8, 1e-7, 1e-6, 1e-5, 1e-4, 1e-3, 1e-2,
                                 1e-1, 1e0, 1e1, 1e2, 1e3, 1e4, 1e5, 1e6, 1e7,
                                 1e8, 1e9, 1e10, 1e11, 1e12, 1e13, 1e14, 1e15,
                                 1e16, 1e17, 1e18, 1e19, 1e20, 1e21, 1e22};
    if (in < ins[eee]) {
      eee -= 8;
    } else {
      eee += 8;
    }
    if (in < ins[eee]) {
      eee -= 4;
    } else {
      eee += 4;
    }
    if (in < ins[eee]) {
      eee -= 2;
    } else {
      eee += 2;
    }
    if (in < ins[eee]) {
      eee -= 1;
    } else {
      eee += 1;
    }
    /* POTENTIAL FLAW */
    if (in < ins[eee]) { //Access out-of-bound array element (buffer overflow)
      eee -= 1;
    }
  }
  return eee;"))
\end{lstlisting}
\end{itemize}
\end{description}

\subsection*{Bug Template {\tt CLANG-REGRESSION-TEST-BUFFER9}}
\begin{description}
\item[Definition:]~\newline
\begin{lstlisting}[language=lisp]
(define-scion clang-regression-test-buffer9
    (make-instance 'clang-scion
                   :name 'clang-regression-test-buffer9
                   :patches (list clang-regression-test-buffer9-patch)))
\end{lstlisting}
\item[Patches:]~
\begin{itemize}
\item Definition for patch {\tt CLANG-REGRESSION-TEST-BUFFER9-PATCH}.
\begin{lstlisting}[language=lisp]
(defparameter clang-regression-test-buffer9-patch
  (make-instance 'clang-dynamic-patch
    :cwe 121
    :cwe-line 3
    :precondition (lambda (obj location)
                    (var-declarable-p obj (ast-at-index obj location) "dest"))
    :free-variables '()
    :includes '("<string.h>")
    :code "char dest[10];
/* POTENTIAL FLAW */
strncat(dest, \"AAAAAAAAAAAAAAAAAAAAAAAAAAAAA\", sizeof(dest) - 1);"))
\end{lstlisting}
\end{itemize}
\end{description}

\subsection*{Bug Template {\tt CLANG-REGRESSION-TEST-POINTER-DEREFERENCE1}}
\begin{description}
\item[Definition:]~\newline
\begin{lstlisting}[language=lisp]
(define-scion clang-regression-test-pointer-dereference1
    (make-instance 'clang-scion
                   :name 'clang-regression-test-pointer-dereference1
                   :patches (list clang-regression-test-pointer-dereference1-patch)))
\end{lstlisting}
\item[Patches:]~
\begin{itemize}
\item Definition for patch {\tt CLANG-REGRESSION-TEST-POINTER-DEREFERENCE1-PATCH}.
\begin{lstlisting}[language=lisp]
(defparameter clang-regression-test-pointer-dereference1-patch
  (make-instance 'clang-dynamic-patch
    :cwe 476
    :cwe-line 2
    :precondition (lambda (obj location a)
                    (declare (ignorable obj location))
                    (= (v/value a) 0))
    :free-variables '(("a" "*int"))
    :code "/* POTENTIAL FLAW */
(a + 0)[0];"))
\end{lstlisting}
\end{itemize}
\end{description}

\subsection*{Bug Template {\tt CLANG-REGRESSION-TEST-POINTER-DEREFERENCE10}}
\begin{description}
\item[Definition:]~\newline
\begin{lstlisting}[language=lisp]
(define-scion clang-regression-test-pointer-dereference10
    (make-instance 'clang-scion
                   :name 'clang-regression-test-pointer-dereference10
                   :patches (list clang-regression-test-pointer-dereference10-patch1
                                  clang-regression-test-pointer-dereference10-patch2)))
\end{lstlisting}
\item[Patches:]~
\begin{itemize}
\item Definition for patch {\tt CLANG-REGRESSION-TEST-POINTER-DEREFERENCE10-PATCH1}.
\begin{lstlisting}[language=lisp]
(defparameter clang-regression-test-pointer-dereference10-patch1
  (make-instance 'clang-static-patch
    :precondition (lambda (obj location)
                    (declare (ignorable obj))
                    (= location 0))
    :free-variables nil
    :code-top-level-p t
    :code "void use2(int *ptr, int val) {
    *ptr = val;
}
int compute() {
    return 2 + 3 + 4 + 5 + 6;
}
void passThrough(int *p) {
  use2(p, compute());
}"))
\end{lstlisting}
\item Definition for patch {\tt CLANG-REGRESSION-TEST-POINTER-DEREFERENCE10-PATCH2}.
\begin{lstlisting}[language=lisp]
(defparameter clang-regression-test-pointer-dereference10-patch2
  (make-instance 'clang-dynamic-patch
    :cwe 476
    :cwe-line 2
    :precondition (lambda (obj location ptr)
                    (declare (ignorable obj location))
                    (= (v/value ptr) 0))
    :free-variables '(("ptr" "*int" :-const))
    :dependencies (list clang-regression-test-pointer-dereference10-patch1)
    :code "/* POTENTIAL FLAW */
passThrough(ptr);"))
\end{lstlisting}
\end{itemize}
\end{description}

\subsection*{Bug Template {\tt CLANG-REGRESSION-TEST-POINTER-DEREFERENCE11}}
\begin{description}
\item[Definition:]~\newline
\begin{lstlisting}[language=lisp]
(define-scion clang-regression-test-pointer-dereference11
    (make-instance 'clang-scion
                   :name 'clang-regression-test-pointer-dereference11
                   :patches (list clang-regression-test-pointer-dereference11-patch1
                                  clang-regression-test-pointer-dereference11-patch2)))
\end{lstlisting}
\item[Patches:]~
\begin{itemize}
\item Definition for patch {\tt CLANG-REGRESSION-TEST-POINTER-DEREFERENCE11-PATCH1}.
\begin{lstlisting}[language=lisp]
(defparameter clang-regression-test-pointer-dereference11-patch1
  (make-instance 'clang-static-patch
    :precondition (lambda (obj location)
                    (declare (ignorable obj))
                    (= location 0))
    :free-variables nil
    :code-top-level-p t
    :code "static void bug(int *p) {
    *p = 0xDEADBEEF;
}"))
\end{lstlisting}
\item Definition for patch {\tt CLANG-REGRESSION-TEST-POINTER-DEREFERENCE11-PATCH2}.
\begin{lstlisting}[language=lisp]
(defparameter clang-regression-test-pointer-dereference11-patch2
  (make-instance 'clang-dynamic-patch
    :cwe 476
    :cwe-line 2
    :precondition (lambda (obj location ptr)
                    (declare (ignorable obj location))
                    (= (v/value ptr) 0))
    :free-variables '(("p" "*int" :-const))
    :dependencies (list clang-regression-test-pointer-dereference11-patch1)
    :code "/* POTENTIAL FLAW */
bug(p);"))
\end{lstlisting}
\end{itemize}
\end{description}

\subsection*{Bug Template {\tt CLANG-REGRESSION-TEST-POINTER-DEREFERENCE12}}
\begin{description}
\item[Definition:]~\newline
\begin{lstlisting}[language=lisp]
(define-scion clang-regression-test-pointer-dereference12
    (make-instance 'clang-scion
                   :name 'clang-regression-test-pointer-dereference12
                   :patches (list clang-regression-test-pointer-dereference12-patch1
                                  clang-regression-test-pointer-dereference12-patch2)))
\end{lstlisting}
\item[Patches:]~
\begin{itemize}
\item Definition for patch {\tt CLANG-REGRESSION-TEST-POINTER-DEREFERENCE12-PATCH1}.
\begin{lstlisting}[language=lisp]
(defparameter clang-regression-test-pointer-dereference12-patch1
  (make-instance 'clang-static-patch
    :precondition (lambda (obj location)
                    (declare (ignorable obj))
                    (= location 0))
    :free-variables nil
    :code-top-level-p t
    :code "int test1_f1() {
    int y = 1;
    y++;
    return y;
}"))
\end{lstlisting}
\item Definition for patch {\tt CLANG-REGRESSION-TEST-POINTER-DEREFERENCE12-PATCH2}.
\begin{lstlisting}[language=lisp]
(defparameter clang-regression-test-pointer-dereference12-patch2
  (make-instance 'clang-dynamic-patch
    :cwe 476
    :cwe-line 10
    :precondition nil
    :free-variables '(("x" "int" :-const))
    :dependencies (list clang-regression-test-pointer-dereference12-patch1)
    :code "x = 1;
x = test1_f1();
if (x == 1) {
    int *p = 0;
    *p = 3;
}
if (x == 2) {
    int *p = 0;
    /* POTENTIAL FLAW */
    *p = 3;
}"))
\end{lstlisting}
\end{itemize}
\end{description}

\subsection*{Bug Template {\tt CLANG-REGRESSION-TEST-POINTER-DEREFERENCE13}}
\begin{description}
\item[Definition:]~\newline
\begin{lstlisting}[language=lisp]
(define-scion clang-regression-test-pointer-dereference13
    (make-instance 'clang-scion
                   :name 'clang-regression-test-pointer-dereference13
                   :patches (list clang-regression-test-pointer-dereference13-patch1
                                  clang-regression-test-pointer-dereference13-patch2)))
\end{lstlisting}
\item[Patches:]~
\begin{itemize}
\item Definition for patch {\tt CLANG-REGRESSION-TEST-POINTER-DEREFERENCE13-PATCH1}.
\begin{lstlisting}[language=lisp]
(defparameter clang-regression-test-pointer-dereference13-patch1
  (make-instance 'clang-static-patch
    :precondition (lambda (obj location)
                    (declare (ignorable obj))
                    (= location 0))
    :free-variables nil
    :code-top-level-p t
    :code "unsigned factorial(unsigned x) {
    if (x <= 1)
        return 1;
    return x * factorial(x - 1);
}"))
\end{lstlisting}
\item Definition for patch {\tt CLANG-REGRESSION-TEST-POINTER-DEREFERENCE13-PATCH2}.
\begin{lstlisting}[language=lisp]
(defparameter clang-regression-test-pointer-dereference13-patch2
  (make-instance 'clang-dynamic-patch
    :cwe 476
    :cwe-line 3
    :precondition (lambda (obj location p)
                    (declare (ignorable obj location))
                    (= (v/value p) 0))
    :free-variables '(("p" "*int" :-const))
    :dependencies (list clang-regression-test-pointer-dereference13-patch1)
    :code "if (factorial(3) == 6) {
    /* POTENTIAL FLAW */
    *p = 0xDEADBEEF;
}"))
\end{lstlisting}
\end{itemize}
\end{description}

\subsection*{Bug Template {\tt CLANG-REGRESSION-TEST-POINTER-DEREFERENCE14}}
\begin{description}
\item[Definition:]~\newline
\begin{lstlisting}[language=lisp]
(define-scion clang-regression-test-pointer-dereference14
    (make-instance 'clang-scion
                   :name 'clang-regression-test-pointer-dereference14
                   :patches (list clang-regression-test-pointer-dereference14-patch)))
\end{lstlisting}
\item[Patches:]~
\begin{itemize}
\item Definition for patch {\tt CLANG-REGRESSION-TEST-POINTER-DEREFERENCE14-PATCH}.
\begin{lstlisting}[language=lisp]
(defparameter clang-regression-test-pointer-dereference14-patch
  (make-instance 'clang-dynamic-patch
    :cwe 476
    :cwe-line 4
    :precondition (lambda (obj location coin)
                    (declare (ignorable obj location))
                    (and (= (v/value coin) 0)
                         (equal "int"
                                (some->> (ast-at-index obj location)
                                         (function-containing-ast obj)
                                         (ast-ret)
                                         (find-type obj)
                                         (type-trace-string)))))
    :free-variables '(("coin" "int"))
    :code "if (coin) {
    int *x = 0;
    /* POTENTIAL FLAW */
    return *x;
} else {
    return 0;
}"))
\end{lstlisting}
\end{itemize}
\end{description}

\subsection*{Bug Template {\tt CLANG-REGRESSION-TEST-POINTER-DEREFERENCE15}}
\begin{description}
\item[Definition:]~\newline
\begin{lstlisting}[language=lisp]
(define-scion clang-regression-test-pointer-dereference15
    (make-instance 'clang-scion
                   :name 'clang-regression-test-pointer-dereference15
                   :patches (list clang-regression-test-pointer-dereference15-patch)))
\end{lstlisting}
\item[Patches:]~
\begin{itemize}
\item Definition for patch {\tt CLANG-REGRESSION-TEST-POINTER-DEREFERENCE15-PATCH}.
\begin{lstlisting}[language=lisp]
(defparameter clang-regression-test-pointer-dereference15-patch
  (make-instance 'clang-dynamic-patch
    :cwe 476
    :cwe-line 2
    :precondition (lambda (obj location x)
                    (and (= (v/value x) 0)
                         (equal "int"
                                (some->> (ast-at-index obj location)
                                         (function-containing-ast obj)
                                         (ast-ret)
                                         (find-type obj)
                                         (type-trace-string)))))
    :free-variables '(("x" "*int"))
    :code "/* POTENTIAL FLAW */
return *x;"))
\end{lstlisting}
\end{itemize}
\end{description}

\subsection*{Bug Template {\tt CLANG-REGRESSION-TEST-POINTER-DEREFERENCE16}}
\begin{description}
\item[Definition:]~\newline
\begin{lstlisting}[language=lisp]
(define-scion clang-regression-test-pointer-dereference16
    (make-instance 'clang-scion
                   :name 'clang-regression-test-pointer-dereference16
                   :patches (list clang-regression-test-pointer-dereference16-patch)))
\end{lstlisting}
\item[Patches:]~
\begin{itemize}
\item Definition for patch {\tt CLANG-REGRESSION-TEST-POINTER-DEREFERENCE16-PATCH}.
\begin{lstlisting}[language=lisp]
(defparameter clang-regression-test-pointer-dereference16-patch
  (make-instance 'clang-dynamic-patch
    :cwe 476
    :cwe-line 4
    :precondition (lambda (obj location param)
                    (let ((ast (ast-at-index obj location)))
                      (and (= (v/value param) 0)
                           (var-declarable-p obj ast "buf")
                           (equal "int"
                                  (some->> (function-containing-ast obj ast)
                                           (ast-ret)
                                           (find-type obj)
                                           (type-trace-string))))))
    :free-variables '(("param" "*int"))
    :macros (list (make-clang-macro :name "DYN_CAST"
                                    :body "DYN_CAST(X) (X ? (char*)X : 0)"
                                    :hash 0))
    :code "char *param2;
param2 = DYN_CAST(param);
/* POTENTIAL FLAW */
return *param2;"))
\end{lstlisting}
\end{itemize}
\end{description}

\subsection*{Bug Template {\tt CLANG-REGRESSION-TEST-POINTER-DEREFERENCE17}}
\begin{description}
\item[Definition:]~\newline
\begin{lstlisting}[language=lisp]
(define-scion clang-regression-test-pointer-dereference17
    (make-instance 'clang-scion
                   :name 'clang-regression-test-pointer-dereference17
                   :patches (list clang-regression-test-pointer-dereference17-patch)))
\end{lstlisting}
\item[Patches:]~
\begin{itemize}
\item Definition for patch {\tt CLANG-REGRESSION-TEST-POINTER-DEREFERENCE17-PATCH}.
\begin{lstlisting}[language=lisp]
(defparameter clang-regression-test-pointer-dereference17-patch
  (make-instance 'clang-dynamic-patch
    :cwe 476
    :cwe-line 3
    :precondition (lambda (obj location p)
                    (and (= (v/value p) 0)
                         (var-declarable-p obj
                                           (ast-at-index obj location)
                                           "x")))
    :free-variables '(("p" "*int"))
    :code "int *x = p ? p : p;
/* POTENTIAL FLAW */
*x = 1;"))
\end{lstlisting}
\end{itemize}
\end{description}

\subsection*{Bug Template {\tt CLANG-REGRESSION-TEST-POINTER-DEREFERENCE18}}
\begin{description}
\item[Definition:]~\newline
\begin{lstlisting}[language=lisp]
(define-scion clang-regression-test-pointer-dereference18
    (make-instance 'clang-scion
                   :name 'clang-regression-test-pointer-dereference18
                   :patches (list clang-regression-test-pointer-dereference18-patch)))
\end{lstlisting}
\item[Patches:]~
\begin{itemize}
\item Definition for patch {\tt CLANG-REGRESSION-TEST-POINTER-DEREFERENCE18-PATCH}.
\begin{lstlisting}[language=lisp]
(defparameter clang-regression-test-pointer-dereference18-patch
  (make-instance 'clang-dynamic-patch
    :cwe 476
    :cwe-line 5
    :precondition (lambda (obj location p)
                    (and (= (v/value p) 0)
                         (some->> (ast-at-index obj location)
                                  (function-containing-ast obj)
                                  (ast-void-ret))))
    :free-variables '(("p" "*int"))
    :code "if (p) {
    return;
}
/* POTENTIAL FLAW */
int x = *p ? 0 : 1;"))
\end{lstlisting}
\end{itemize}
\end{description}

\subsection*{Bug Template {\tt CLANG-REGRESSION-TEST-POINTER-DEREFERENCE19}}
\begin{description}
\item[Definition:]~\newline
\begin{lstlisting}[language=lisp]
(define-scion clang-regression-test-pointer-dereference19
    (make-instance 'clang-scion
                   :name 'clang-regression-test-pointer-dereference19
                   :patches (list clang-regression-test-pointer-dereference19-patch)))
\end{lstlisting}
\item[Patches:]~
\begin{itemize}
\item Definition for patch {\tt CLANG-REGRESSION-TEST-POINTER-DEREFERENCE19-PATCH}.
\begin{lstlisting}[language=lisp]
(defparameter clang-regression-test-pointer-dereference19-patch
  (make-instance 'clang-dynamic-patch
    :cwe 476
    :cwe-line 2
    :precondition (lambda (obj location p)
                    (and (= (v/value p) 0)
                         (var-declarable-p obj
                                           (ast-at-index obj location)
                                           "x")))
    :free-variables '(("p" "*int"))
    :code "/* POTENTIAL FLAW */
int x = !p ? *p : 1;"))
\end{lstlisting}
\end{itemize}
\end{description}

\subsection*{Bug Template {\tt CLANG-REGRESSION-TEST-POINTER-DEREFERENCE2}}
\begin{description}
\item[Definition:]~\newline
\begin{lstlisting}[language=lisp]
(define-scion clang-regression-test-pointer-dereference2
    (make-instance 'clang-scion
                   :name 'clang-regression-test-pointer-dereference2
                   :patches (list clang-regression-test-pointer-dereference2-patch)))
\end{lstlisting}
\item[Patches:]~
\begin{itemize}
\item Definition for patch {\tt CLANG-REGRESSION-TEST-POINTER-DEREFERENCE2-PATCH}.
\begin{lstlisting}[language=lisp]
(defparameter clang-regression-test-pointer-dereference2-patch
  (make-instance 'clang-dynamic-patch
    :cwe 476
    :cwe-line 2
    :precondition (lambda (obj location destination source)
                    (declare (ignorable obj location source))
                    (= (v/value destination) 0))
    :free-variables '(("destination" "*char" :-const) ("source" "*char"))
    :includes '("<string.h>")
    :code "/* POTENTIAL FLAW */
memcpy(destination + 0, source, 10);"))
\end{lstlisting}
\end{itemize}
\end{description}

\subsection*{Bug Template {\tt CLANG-REGRESSION-TEST-POINTER-DEREFERENCE20}}
\begin{description}
\item[Definition:]~\newline
\begin{lstlisting}[language=lisp]
(define-scion clang-regression-test-pointer-dereference20
    (make-instance 'clang-scion
                   :name 'clang-regression-test-pointer-dereference20
                   :patches (list clang-regression-test-pointer-dereference20-patch)))
\end{lstlisting}
\item[Patches:]~
\begin{itemize}
\item Definition for patch {\tt CLANG-REGRESSION-TEST-POINTER-DEREFERENCE20-PATCH}.
\begin{lstlisting}[language=lisp]
(defparameter clang-regression-test-pointer-dereference20-patch
  (make-instance 'clang-dynamic-patch
    :cwe 476
    :cwe-line 2
    :precondition (lambda (obj location p)
                    (and (= (v/value p) 0)
                         (var-declarable-p obj
                                           (ast-at-index obj location)
                                           "x")))
    :free-variables '(("p" "*int"))
    :code "/* POTENTIAL FLAW */
int x = p ? 1 : *p;"))
\end{lstlisting}
\end{itemize}
\end{description}

\subsection*{Bug Template {\tt CLANG-REGRESSION-TEST-POINTER-DEREFERENCE21}}
\begin{description}
\item[Definition:]~\newline
\begin{lstlisting}[language=lisp]
(define-scion clang-regression-test-pointer-dereference21
    (make-instance 'clang-scion
                   :name 'clang-regression-test-pointer-dereference21
                   :patches (list clang-regression-test-pointer-dereference21-patch)))
\end{lstlisting}
\item[Patches:]~
\begin{itemize}
\item Definition for patch {\tt CLANG-REGRESSION-TEST-POINTER-DEREFERENCE21-PATCH}.
\begin{lstlisting}[language=lisp]
(defparameter clang-regression-test-pointer-dereference21-patch
  (make-instance 'clang-dynamic-patch
    :cwe 476
    :cwe-line 1
    :precondition nil
    :free-variables '()
    :code "*(volatile int *)0 = 1;"))
\end{lstlisting}
\end{itemize}
\end{description}

\subsection*{Bug Template {\tt CLANG-REGRESSION-TEST-POINTER-DEREFERENCE22}}
\begin{description}
\item[Definition:]~\newline
\begin{lstlisting}[language=lisp]
(define-scion clang-regression-test-pointer-dereference22
    (make-instance 'clang-scion
                   :name 'clang-regression-test-pointer-dereference22
                   :patches (list clang-regression-test-pointer-dereference22-patch)))
\end{lstlisting}
\item[Patches:]~
\begin{itemize}
\item Definition for patch {\tt CLANG-REGRESSION-TEST-POINTER-DEREFERENCE22-PATCH}.
\begin{lstlisting}[language=lisp]
(defparameter clang-regression-test-pointer-dereference22-patch
  (make-instance 'clang-dynamic-patch
    :cwe 476
    :cwe-line 7
    :precondition nil
    :precondition (lambda (obj location input)
                    (let ((ast (ast-at-index obj location)))
                      (and (not (= (v/value input) 0))
                           (var-declarable-p obj ast "p")
                           (equal "int"
                                  (some->> (function-containing-ast obj ast)
                                           (ast-ret)
                                           (find-type obj)
                                           (type-trace-string))))))
    :free-variables '(("input" "int"))
    :code "int *p = 0;
if (input)
    goto mylabel;
return 0;
mylabel:
    /* POTENTIAL FLAW */
    return *p;"))
\end{lstlisting}
\end{itemize}
\end{description}

\subsection*{Bug Template {\tt CLANG-REGRESSION-TEST-POINTER-DEREFERENCE23}}
\begin{description}
\item[Definition:]~\newline
\begin{lstlisting}[language=lisp]
(define-scion clang-regression-test-pointer-dereference23
    (make-instance 'clang-scion
                   :name 'clang-regression-test-pointer-dereference23
                   :patches (list clang-regression-test-pointer-dereference23-patch1
                                  clang-regression-test-pointer-dereference23-patch2)))
\end{lstlisting}
\item[Patches:]~
\begin{itemize}
\item Definition for patch {\tt CLANG-REGRESSION-TEST-POINTER-DEREFERENCE23-PATCH1}.
\begin{lstlisting}[language=lisp]
(defparameter clang-regression-test-pointer-dereference23-patch1
  (make-instance 'clang-static-patch
    :precondition (lambda (obj location)
                    (declare (ignorable obj))
                    (= 0 location))
    :code-top-level-p t
    :code "void zero(int **p) {
    *p = 0;
}"))
\end{lstlisting}
\item Definition for patch {\tt CLANG-REGRESSION-TEST-POINTER-DEREFERENCE23-PATCH2}.
\begin{lstlisting}[language=lisp]
(defparameter clang-regression-test-pointer-dereference23-patch2
  (make-instance 'clang-dynamic-patch
    :cwe 476
    :cwe-line 3
    :precondition nil
    :free-variables '(("a" "*int" :-const))
    :dependencies (list clang-regression-test-pointer-dereference23-patch1)
    :code "zero(&a);
/* POTENTIAL FLAW */
*a = 1;"))
\end{lstlisting}
\end{itemize}
\end{description}

\subsection*{Bug Template {\tt CLANG-REGRESSION-TEST-POINTER-DEREFERENCE24}}
\begin{description}
\item[Definition:]~\newline
\begin{lstlisting}[language=lisp]
(define-scion clang-regression-test-pointer-dereference24
    (make-instance 'clang-scion
                   :name 'clang-regression-test-pointer-dereference24
                   :patches (list clang-regression-test-pointer-dereference24-patch)))
\end{lstlisting}
\item[Patches:]~
\begin{itemize}
\item Definition for patch {\tt CLANG-REGRESSION-TEST-POINTER-DEREFERENCE24-PATCH}.
\begin{lstlisting}[language=lisp]
(defparameter clang-regression-test-pointer-dereference24-patch
  (make-instance 'clang-dynamic-patch
    :cwe 476
    :cwe-line 5
    :precondition (lambda (obj location p)
                    (and (= (v/value p) 0)
                         (some->> (ast-at-index obj location)
                                  (function-containing-ast obj)
                                  (ast-void-ret))))
    :free-variables '(("p" "*int*" :-const))
    :code "if (*p) {
    return;
}
/* POTENTIAL FLAW */
**p = 1;"))
\end{lstlisting}
\end{itemize}
\end{description}

\subsection*{Bug Template {\tt CLANG-REGRESSION-TEST-POINTER-DEREFERENCE25}}
\begin{description}
\item[Definition:]~\newline
\begin{lstlisting}[language=lisp]
(define-scion clang-regression-test-pointer-dereference25
    (make-instance 'clang-scion
                   :name 'clang-regression-test-pointer-dereference25
                   :patches (list clang-regression-test-pointer-dereference25-patch)))
\end{lstlisting}
\item[Patches:]~
\begin{itemize}
\item Definition for patch {\tt CLANG-REGRESSION-TEST-POINTER-DEREFERENCE25-PATCH}.
\begin{lstlisting}[language=lisp]
(defparameter clang-regression-test-pointer-dereference25-patch
  (make-instance 'clang-dynamic-patch
    :cwe 476
    :cwe-line 3
    :precondition (lambda (obj location x)
                    (and (= (v/value x) 0)
                         (equal "int" (some->> (ast-at-index obj location)
                                               (function-containing-ast obj)
                                               (ast-ret)
                                               (find-type obj)
                                               (type-trace-string)))))
    :free-variables '(("x" "*int*"))
    :code "if (!x) {
    /* POTENTIAL FLAW */
    return **x;
}
return 1;"))
\end{lstlisting}
\end{itemize}
\end{description}

\subsection*{Bug Template {\tt CLANG-REGRESSION-TEST-POINTER-DEREFERENCE26}}
\begin{description}
\item[Definition:]~\newline
\begin{lstlisting}[language=lisp]
(define-scion clang-regression-test-pointer-dereference26
    (make-instance 'clang-scion
                   :name 'clang-regression-test-pointer-dereference26
                   :patches (list clang-regression-test-pointer-dereference26-patch1
                                  clang-regression-test-pointer-dereference26-patch2)))
\end{lstlisting}
\item[Patches:]~
\begin{itemize}
\item Definition for patch {\tt CLANG-REGRESSION-TEST-POINTER-DEREFERENCE26-PATCH1}.
\begin{lstlisting}[language=lisp]
(defparameter clang-regression-test-pointer-dereference26-patch1
  (make-instance 'clang-static-patch
    :precondition (lambda (obj location)
                    (declare (ignorable obj))
                    (= location 0))
    :free-variables nil
    :code-top-level-p t
    :code "void init_in_func(int **x) {
  *x = 0;
}"))
\end{lstlisting}
\item Definition for patch {\tt CLANG-REGRESSION-TEST-POINTER-DEREFERENCE26-PATCH2}.
\begin{lstlisting}[language=lisp]
(defparameter clang-regression-test-pointer-dereference26-patch2
  (make-instance 'clang-dynamic-patch
    :cwe 476
    :cwe-line 4
    :precondition (lambda (obj location x)
                    (declare (ignorable x))
                    (let ((ast (ast-at-index obj location)))
                      (and (var-declarable-p obj ast "y")
                           (equal "int" (some->> (function-containing-ast
                                                   obj ast)
                                                 (ast-ret)
                                                 (find-type obj)
                                                 (type-trace-string))))))
    :dependencies (list clang-regression-test-pointer-dereference26-patch1)
    :free-variables '(("x" "int" :-const))
    :code "int *y = &x;
init_in_func(&y);
/* POTENTIAL FLAW */
return *y;"))
\end{lstlisting}
\end{itemize}
\end{description}

\subsection*{Bug Template {\tt CLANG-REGRESSION-TEST-POINTER-DEREFERENCE27}}
\begin{description}
\item[Definition:]~\newline
\begin{lstlisting}[language=lisp]
(define-scion clang-regression-test-pointer-dereference27
    (make-instance 'clang-scion
                   :name 'clang-regression-test-pointer-dereference27
                   :patches (list clang-regression-test-pointer-dereference27-patch)))
\end{lstlisting}
\item[Patches:]~
\begin{itemize}
\item Definition for patch {\tt CLANG-REGRESSION-TEST-POINTER-DEREFERENCE27-PATCH}.
\begin{lstlisting}[language=lisp]
(defparameter clang-regression-test-pointer-dereference27-patch
  (make-instance 'clang-dynamic-patch
    :cwe 476
    :cwe-line 4
    :precondition (lambda (obj location p)
                    (and (= (v/value p) 0)
                         (equal "int" (some->> (ast-at-index obj location)
                                               (function-containing-ast obj)
                                               (ast-ret)
                                               (find-type obj)
                                               (type-trace-string)))))
    :free-variables '(("p" "*int"))
    :macros (list (make-clang-macro :name "macroWithArg"
                                    :body "macroWithArg(mp) mp==0"
                                    :hash 0))
    :code "if (macroWithArg(p))
    ;
/* POTENTIAL FLAW */
return *p;"))
\end{lstlisting}
\end{itemize}
\end{description}

\subsection*{Bug Template {\tt CLANG-REGRESSION-TEST-POINTER-DEREFERENCE28}}
\begin{description}
\item[Definition:]~\newline
\begin{lstlisting}[language=lisp]
(define-scion clang-regression-test-pointer-dereference28
    (make-instance 'clang-scion
                   :name 'clang-regression-test-pointer-dereference28
                   :patches (list clang-regression-test-pointer-dereference28-patch)))
\end{lstlisting}
\item[Patches:]~
\begin{itemize}
\item Definition for patch {\tt CLANG-REGRESSION-TEST-POINTER-DEREFERENCE28-PATCH}.
\begin{lstlisting}[language=lisp]
(defparameter clang-regression-test-pointer-dereference28-patch
  (make-instance 'clang-dynamic-patch
    :cwe 122
    :cwe-line 4
    :precondition (lambda (obj location p)
                    (declare (ignorable p))
                    (equal "int" (some->> (ast-at-index obj location)
                                          (function-containing-ast obj)
                                          (ast-ret)
                                          (find-type obj)
                                          (type-trace-string))))
    :free-variables '(("p" "*int" :-const))
    :includes '("<stdlib.h>")
    :code "p = (int *) malloc(sizeof(int));
p -= 1;
/* POTENTIAL FLAW */
return *p;"))
\end{lstlisting}
\end{itemize}
\end{description}

\subsection*{Bug Template {\tt CLANG-REGRESSION-TEST-POINTER-DEREFERENCE29}}
\begin{description}
\item[Definition:]~\newline
\begin{lstlisting}[language=lisp]
(define-scion clang-regression-test-pointer-dereference29
    (make-instance 'clang-scion
                   :name 'clang-regression-test-pointer-dereference29
                   :patches (list clang-regression-test-pointer-dereference29-patch)))
\end{lstlisting}
\item[Patches:]~
\begin{itemize}
\item Definition for patch {\tt CLANG-REGRESSION-TEST-POINTER-DEREFERENCE29-PATCH}.
\begin{lstlisting}[language=lisp]
(defparameter clang-regression-test-pointer-dereference29-patch
  (make-instance 'clang-dynamic-patch
    :cwe 122
    :cwe-line 5
    :precondition (lambda (obj location p)
                    (declare (ignorable p))
                    (equal "int" (some->> (ast-at-index obj location)
                                          (function-containing-ast obj)
                                          (ast-ret)
                                          (find-type obj)
                                          (type-trace-string))))
    :free-variables '(("p" "*int" :-const))
    :includes '("<stdlib.h>")
    :code "p = (int *) malloc(sizeof(int));
p -= 2;
p += 1;
/* POTENTIAL FLAW */
return *p;"))
\end{lstlisting}
\end{itemize}
\end{description}

\subsection*{Bug Template {\tt CLANG-REGRESSION-TEST-POINTER-DEREFERENCE3}}
\begin{description}
\item[Definition:]~\newline
\begin{lstlisting}[language=lisp]
(define-scion clang-regression-test-pointer-dereference3
    (make-instance 'clang-scion
                   :name 'clang-regression-test-pointer-dereference3
                   :patches (list clang-regression-test-pointer-dereference3-patch)))
\end{lstlisting}
\item[Patches:]~
\begin{itemize}
\item Definition for patch {\tt CLANG-REGRESSION-TEST-POINTER-DEREFERENCE3-PATCH}.
\begin{lstlisting}[language=lisp]
(defparameter clang-regression-test-pointer-dereference3-patch
  (make-instance 'clang-dynamic-patch
    :cwe 476
    :cwe-line 2
    :precondition (lambda (obj location destination source)
                    (declare (ignorable obj location source))
                    (= (v/value destination) 0))
    :free-variables '(("destination" "*char" :-const) ("source" "*char"))
    :includes '("<string.h>")
    :code "/* POTENTIAL FLAW */
memcpy(destination - 0, source, 10);"))
\end{lstlisting}
\end{itemize}
\end{description}

\subsection*{Bug Template {\tt CLANG-REGRESSION-TEST-POINTER-DEREFERENCE30}}
\begin{description}
\item[Definition:]~\newline
\begin{lstlisting}[language=lisp]
(define-scion clang-regression-test-pointer-dereference30
    (make-instance 'clang-scion
                   :name 'clang-regression-test-pointer-dereference30
                   :patches (list clang-regression-test-pointer-dereference30-patch)))
\end{lstlisting}
\item[Patches:]~
\begin{itemize}
\item Definition for patch {\tt CLANG-REGRESSION-TEST-POINTER-DEREFERENCE30-PATCH}.
\begin{lstlisting}[language=lisp]
(defparameter clang-regression-test-pointer-dereference30-patch
  (make-instance 'clang-dynamic-patch
    :cwe 122
    :cwe-line 6
    :precondition (lambda (obj location p)
                    (declare (ignorable p))
                    (equal "int" (some->> (ast-at-index obj location)
                                          (function-containing-ast obj)
                                          (ast-ret)
                                          (find-type obj)
                                          (type-trace-string))))
    :free-variables '(("p" "*int" :-const))
    :includes '("<stdlib.h>")
    :code "p = (int *) malloc(sizeof(int));
p++;
p--;
p--;
/* POTENTIAL FLAW */
return *p;"))
\end{lstlisting}
\end{itemize}
\end{description}

\subsection*{Bug Template {\tt CLANG-REGRESSION-TEST-POINTER-DEREFERENCE31}}
\begin{description}
\item[Definition:]~\newline
\begin{lstlisting}[language=lisp]
(define-scion clang-regression-test-pointer-dereference31
    (make-instance 'clang-scion
                   :name 'clang-regression-test-pointer-dereference31
                   :patches (list clang-regression-test-pointer-dereference31-patch)))
\end{lstlisting}
\item[Patches:]~
\begin{itemize}
\item Definition for patch {\tt CLANG-REGRESSION-TEST-POINTER-DEREFERENCE31-PATCH}.
\begin{lstlisting}[language=lisp]
(defparameter clang-regression-test-pointer-dereference31-patch
  (make-instance 'clang-dynamic-patch
    :cwe 476
    :cwe-line 4
    :precondition (lambda (obj location p)
                    (and (= (v/value p) 0)
                         (var-declarable-p obj (ast-at-index obj location) "i")))
    :free-variables '(("p" "*int" :-const))
    :macros (list (make-clang-macro
                    :name "MACRO_WITH_CHECK"
                    :body "MACRO_WITH_CHECK(a) ( ((a) != 0) ? *a : 17 )"
                    :hash 0))
    :code "int i = MACRO_WITH_CHECK(p);
(void)i;
/* POTENTIAL FLAW */
*p = 1;"))
\end{lstlisting}
\end{itemize}
\end{description}

\subsection*{Bug Template {\tt CLANG-REGRESSION-TEST-POINTER-DEREFERENCE32}}
\begin{description}
\item[Definition:]~\newline
\begin{lstlisting}[language=lisp]
(define-scion clang-regression-test-pointer-dereference32
    (make-instance 'clang-scion
                   :name 'clang-regression-test-pointer-dereference32
                   :patches (list clang-regression-test-pointer-dereference32-patch)))
\end{lstlisting}
\item[Patches:]~
\begin{itemize}
\item Definition for patch {\tt CLANG-REGRESSION-TEST-POINTER-DEREFERENCE32-PATCH}.
\begin{lstlisting}[language=lisp]
(defparameter clang-regression-test-pointer-dereference32-patch
  (make-instance 'clang-dynamic-patch
    :cwe 476
    :cwe-line 3
    :precondition (lambda (obj location p)
                    (declare (ignorable obj location))
                    (= (v/value p) 0))
    :free-variables '(("p" "*int" :-const))
    :macros (list (make-clang-macro
                    :name "MACRO_WITH_NESTED_CHECK"
                    :body "MACRO_WITH_NESTED_CHECK(a) ( { int j = MACRO_WITH_CHECK(a); j; } )"
                    :hash 1)
                  (make-clang-macro
                    :name "MACRO_WITH_CHECK"
                    :body "MACRO_WITH_CHECK(a) ( ((a) != 0) ? *a : 17)"
                    :hash 0))
    :code "MACRO_WITH_NESTED_CHECK(p);
/* POTENTIAL FLAW */
*p = 1;"))
\end{lstlisting}
\end{itemize}
\end{description}

\subsection*{Bug Template {\tt CLANG-REGRESSION-TEST-POINTER-DEREFERENCE33}}
\begin{description}
\item[Definition:]~\newline
\begin{lstlisting}[language=lisp]
(define-scion clang-regression-test-pointer-dereference33
    (make-instance 'clang-scion
                   :name 'clang-regression-test-pointer-dereference33
                   :patches (list clang-regression-test-pointer-dereference33-patch)))
\end{lstlisting}
\item[Patches:]~
\begin{itemize}
\item Definition for patch {\tt CLANG-REGRESSION-TEST-POINTER-DEREFERENCE33-PATCH}.
\begin{lstlisting}[language=lisp]
(defparameter clang-regression-test-pointer-dereference33-patch
  (make-instance 'clang-dynamic-patch
    :cwe 476
    :cwe-line 2
    :precondition (lambda (obj location p)
                    (and (= (v/value p) 0)
                            (var-declarable-p obj
                                              (ast-at-index obj location)
                                              "i")))
    :free-variables '(("p" "*int"))
    :macros (list (make-clang-macro
                    :name "MACRO_WITH_ERROR"
                    :body "MACRO_WITH_ERROR(a) ( ((a) != 0) ? 0 : *a)"
                    :hash 0))
    :code "/* POTENTIAL FLAW */
int i = MACRO_WITH_ERROR(p);"))
\end{lstlisting}
\end{itemize}
\end{description}

\subsection*{Bug Template {\tt CLANG-REGRESSION-TEST-POINTER-DEREFERENCE34}}
\begin{description}
\item[Definition:]~\newline
\begin{lstlisting}[language=lisp]
(define-scion clang-regression-test-pointer-dereference34
    (make-instance 'clang-scion
                   :name 'clang-regression-test-pointer-dereference34
                   :patches (list clang-regression-test-pointer-dereference34-patch)))
\end{lstlisting}
\item[Patches:]~
\begin{itemize}
\item Definition for patch {\tt CLANG-REGRESSION-TEST-POINTER-DEREFERENCE34-PATCH}.
\begin{lstlisting}[language=lisp]
(defparameter clang-regression-test-pointer-dereference34-patch
  (make-instance 'clang-dynamic-patch
    :cwe 476
    :cwe-line 2
    :precondition (lambda (obj location p)
                    (and (= (v/value p) 0)
                            (var-declarable-p obj
                                              (ast-at-index obj location)
                                              "i")))
    :free-variables '(("p" "*int"))
    :macros (list (make-clang-macro
                    :name "MACRO_DO_IT"
                    :body "MACRO_DO_IT(a) (a)"
                    :hash 0))
    :code "/* POTENTIAL FLAW */
int i = MACRO_DO_IT((p ? 0 : *p));"))
\end{lstlisting}
\end{itemize}
\end{description}

\subsection*{Bug Template {\tt CLANG-REGRESSION-TEST-POINTER-DEREFERENCE35}}
\begin{description}
\item[Definition:]~\newline
\begin{lstlisting}[language=lisp]
(define-scion clang-regression-test-pointer-dereference35
    (make-instance 'clang-scion
                   :name 'clang-regression-test-pointer-dereference35
                   :patches (list clang-regression-test-pointer-dereference35-patch)))
\end{lstlisting}
\item[Patches:]~
\begin{itemize}
\item Definition for patch {\tt CLANG-REGRESSION-TEST-POINTER-DEREFERENCE35-PATCH}.
\begin{lstlisting}[language=lisp]
(defparameter clang-regression-test-pointer-dereference35-patch
  (make-instance 'clang-dynamic-patch
    :cwe 476
    :cwe-line 2
    :precondition (lambda (obj location x)
                    (and (= (v/value x) 0)
                         (equal "int"
                                (some->> (ast-at-index obj location)
                                         (function-containing-ast obj)
                                         (ast-ret)
                                         (find-type obj)
                                         (type-trace-string)))))
    :free-variables '(("x" "int"))
    :includes '("<stdlib.h>")
    :code "/* POTENTIAL FLAW */
return *(x ? 0 : ((int*) malloc(sizeof(int))));"))
\end{lstlisting}
\end{itemize}
\end{description}

\subsection*{Bug Template {\tt CLANG-REGRESSION-TEST-POINTER-DEREFERENCE36}}
\begin{description}
\item[Definition:]~\newline
\begin{lstlisting}[language=lisp]
(define-scion clang-regression-test-pointer-dereference36
    (make-instance 'clang-scion
                   :name 'clang-regression-test-pointer-dereference36
                   :patches (list clang-regression-test-pointer-dereference36-patch)))
\end{lstlisting}
\item[Patches:]~
\begin{itemize}
\item Definition for patch {\tt CLANG-REGRESSION-TEST-POINTER-DEREFERENCE36-PATCH}.
\begin{lstlisting}[language=lisp]
(defparameter clang-regression-test-pointer-dereference36-patch
  (make-instance 'clang-dynamic-patch
    :cwe 476
    :cwe-line 2
    :precondition (lambda (obj location x)
                    (and (= (v/value x) 0)
                         (equal "int"
                                (some->> (ast-at-index obj location)
                                         (function-containing-ast obj)
                                         (ast-ret)
                                         (find-type obj)
                                         (type-trace-string)))))
    :free-variables '(("x" "int"))
    :includes '("<stdlib.h>")
    :code "/* POTENTIAL FLAW */
return *(x ? 0 : ((int*) malloc(sizeof(int))));"))
\end{lstlisting}
\end{itemize}
\end{description}

\subsection*{Bug Template {\tt CLANG-REGRESSION-TEST-POINTER-DEREFERENCE37}}
\begin{description}
\item[Definition:]~\newline
\begin{lstlisting}[language=lisp]
(define-scion clang-regression-test-pointer-dereference37
    (make-instance 'clang-scion
                   :name 'clang-regression-test-pointer-dereference37
                   :patches (list clang-regression-test-pointer-dereference37-patch)))
\end{lstlisting}
\item[Patches:]~
\begin{itemize}
\item Definition for patch {\tt CLANG-REGRESSION-TEST-POINTER-DEREFERENCE37-PATCH}.
\begin{lstlisting}[language=lisp]
(defparameter clang-regression-test-pointer-dereference37-patch
  (make-instance 'clang-dynamic-patch
    :cwe 476
    :cwe-line 2
    :precondition (lambda (obj location p)
                    (declare (ignorable obj location))
                    (= (v/value p) 0))
    :free-variables '(("p" "*int"))
    :macros (list (make-clang-macro :name "DEREF"
                                    :body "DEREF(p) *p = 0xDEADBEEF"
                                    :hash 0))
    :code "/* POTENTIAL FLAW */
DEREF(p);"))
\end{lstlisting}
\end{itemize}
\end{description}

\subsection*{Bug Template {\tt CLANG-REGRESSION-TEST-POINTER-DEREFERENCE4}}
\begin{description}
\item[Definition:]~\newline
\begin{lstlisting}[language=lisp]
(define-scion clang-regression-test-pointer-dereference4
    (make-instance 'clang-scion
                   :name 'clang-regression-test-pointer-dereference4
                   :patches (list clang-regression-test-pointer-dereference4-patch)))
\end{lstlisting}
\item[Patches:]~
\begin{itemize}
\item Definition for patch {\tt CLANG-REGRESSION-TEST-POINTER-DEREFERENCE4-PATCH}.
\begin{lstlisting}[language=lisp]
(defparameter clang-regression-test-pointer-dereference4-patch
  (make-instance 'clang-dynamic-patch
    :cwe 476
    :cwe-line 3
    :precondition (lambda (obj location destination source)
                    (declare (ignorable obj location source))
                    (= (v/value destination) 0))
    :free-variables '(("destination" "*char" :-const) ("source" "*char"))
    :includes '("<string.h>")
    :code "destination = destination + 0;
/* POTENTIAL FLAW */
memcpy(destination, source, 10);"))
\end{lstlisting}
\end{itemize}
\end{description}

\subsection*{Bug Template {\tt CLANG-REGRESSION-TEST-POINTER-DEREFERENCE5}}
\begin{description}
\item[Definition:]~\newline
\begin{lstlisting}[language=lisp]
(define-scion clang-regression-test-pointer-dereference5
    (make-instance 'clang-scion
                   :name 'clang-regression-test-pointer-dereference5
                   :patches (list clang-regression-test-pointer-dereference5-patch)))
\end{lstlisting}
\item[Patches:]~
\begin{itemize}
\item Definition for patch {\tt CLANG-REGRESSION-TEST-POINTER-DEREFERENCE5-PATCH}.
\begin{lstlisting}[language=lisp]
(defparameter clang-regression-test-pointer-dereference5-patch
  (make-instance 'clang-dynamic-patch
    :cwe 476
    :cwe-line 3
    :precondition (lambda (obj location dest1 dest2 src)
                    (declare (ignorable obj location dest2 src))
                    (= (v/value dest1) 0))
    :free-variables '(("dest1" "*char") ("dest2" "*char" :-const) ("src" "*char"))
    :includes '("<string.h>")
    :code "dest2 = dest1 - 0;
/* POTENTIAL FLAW */
memcpy(dest2, src, 10);"))
\end{lstlisting}
\end{itemize}
\end{description}

\subsection*{Bug Template {\tt CLANG-REGRESSION-TEST-POINTER-DEREFERENCE6}}
\begin{description}
\item[Definition:]~\newline
\begin{lstlisting}[language=lisp]
(define-scion clang-regression-test-pointer-dereference6
    (make-instance 'clang-scion
                   :name 'clang-regression-test-pointer-dereference6
                   :patches (list clang-regression-test-pointer-dereference6-patch)))
\end{lstlisting}
\item[Patches:]~
\begin{itemize}
\item Definition for patch {\tt CLANG-REGRESSION-TEST-POINTER-DEREFERENCE6-PATCH}.
\begin{lstlisting}[language=lisp]
(defparameter clang-regression-test-pointer-dereference6-patch
  (make-instance 'clang-dynamic-patch
    :cwe 476
    :cwe-line 2
    :precondition (lambda (obj location p)
                    (declare (ignorable obj location))
                    (= (v/value p) 0))
    :free-variables '(("p" "*int" :-const))
    :code "/* POTENTIAL FLAW */
*p = 1;"))
\end{lstlisting}
\end{itemize}
\end{description}

\subsection*{Bug Template {\tt CLANG-REGRESSION-TEST-POINTER-DEREFERENCE7}}
\begin{description}
\item[Definition:]~\newline
\begin{lstlisting}[language=lisp]
(define-scion clang-regression-test-pointer-dereference7
    (make-instance 'clang-scion
                   :name 'clang-regression-test-pointer-dereference7
                   :patches (list clang-regression-test-pointer-dereference7-patch)))
\end{lstlisting}
\item[Patches:]~
\begin{itemize}
\item Definition for patch {\tt CLANG-REGRESSION-TEST-POINTER-DEREFERENCE7-PATCH}.
\begin{lstlisting}[language=lisp]
(defparameter clang-regression-test-pointer-dereference7-patch
  (make-instance 'clang-dynamic-patch
    :cwe 476
    :cwe-line 5
    :precondition (lambda (obj location q)
                    (and (= (v/value q) 0)
                         (some->> (ast-at-index obj location)
                                  (function-containing-ast obj)
                                  (ast-void-ret))))
    :free-variables '(("q" "*int" :-const))
    :code "if (q) {
    return;
}
/* POTENTIAL FLAW */
*q = 1;"))
\end{lstlisting}
\end{itemize}
\end{description}

\subsection*{Bug Template {\tt CLANG-REGRESSION-TEST-POINTER-DEREFERENCE8}}
\begin{description}
\item[Definition:]~\newline
\begin{lstlisting}[language=lisp]
(define-scion clang-regression-test-pointer-dereference8
    (make-instance 'clang-scion
                   :name 'clang-regression-test-pointer-dereference8
                   :patches (list clang-regression-test-pointer-dereference8-patch)))
\end{lstlisting}
\item[Patches:]~
\begin{itemize}
\item Definition for patch {\tt CLANG-REGRESSION-TEST-POINTER-DEREFERENCE8-PATCH}.
\begin{lstlisting}[language=lisp]
(defparameter clang-regression-test-pointer-dereference8-patch
  (make-instance 'clang-dynamic-patch
    :cwe 476
    :cwe-line 4
    :precondition (lambda (obj location coin)
                    (and (not (= (v/value coin) 0))
                         (equal "int"
                                (some->> (ast-at-index obj location)
                                         (function-containing-ast obj)
                                         (ast-ret)
                                         (find-type obj)
                                         (type-trace-string)))))
    :free-variables '(("coin" "int"))
    :macros (list (make-clang-macro :name "deref"
                                    :body "deref(X) (*X)"
                                    :hash 0))
    :code "if (coin) {
    int *x = 0;
    /* POTENTIAL FLAW */
    return deref(x);
} else {
    return 0;
}"))
\end{lstlisting}
\end{itemize}
\end{description}

\subsection*{Bug Template {\tt CLANG-REGRESSION-TEST-POINTER-DEREFERENCE9}}
\begin{description}
\item[Definition:]~\newline
\begin{lstlisting}[language=lisp]
(define-scion clang-regression-test-pointer-dereference9
    (make-instance 'clang-scion
                   :name 'clang-regression-test-pointer-dereference9
                   :patches (list clang-regression-test-pointer-dereference9-patch1
                                  clang-regression-test-pointer-dereference9-patch2)))
\end{lstlisting}
\item[Patches:]~
\begin{itemize}
\item Definition for patch {\tt CLANG-REGRESSION-TEST-POINTER-DEREFERENCE9-PATCH1}.
\begin{lstlisting}[language=lisp]
(defparameter clang-regression-test-pointer-dereference9-patch1
  (make-instance 'clang-static-patch
    :precondition (lambda (obj location)
                    (declare (ignorable obj))
                    (= location 0))
    :free-variables nil
    :code-top-level-p t
    :code "void use(int *ptr, int val) {
    *ptr = val;
}
int compute() {
    return 2 + 3 + 4 + 5 + 6;
}"))
\end{lstlisting}
\item Definition for patch {\tt CLANG-REGRESSION-TEST-POINTER-DEREFERENCE9-PATCH2}.
\begin{lstlisting}[language=lisp]
(defparameter clang-regression-test-pointer-dereference9-patch2
  (make-instance 'clang-dynamic-patch
    :cwe 476
    :cwe-line 2
    :precondition (lambda (obj location p)
                    (declare (ignorable obj location))
                    (= (v/value p) 0))
    :free-variables '(("p" "*int" :-const))
    :dependencies (list clang-regression-test-pointer-dereference9-patch1)
    :code "/* POTENTIAL FLAW */
use(p, compute());"))
\end{lstlisting}
\end{itemize}
\end{description}

\subsection*{Bug Template {\tt CWE121\_STACK\_BASED\_BUFFER\_OVERFLOW\_\_CWE193\_CHAR\_ALLOCA\_CPY\_01\_BAD\_INLINE}}
\begin{description}
\item[Definition:]~\newline
\begin{lstlisting}[language=lisp]
(define-scion CWE121_Stack_Based_Buffer_Overflow__CWE193_char_alloca_cpy_01_bad_inline
  (make-instance 'clang-scion
    :name 'CWE121_Stack_Based_Buffer_Overflow__CWE193_char_alloca_cpy_01_bad_inline
    :patches (list printLine_patch CWE121_Stack_Based_Buffer_Overflow__CWE193_char_alloca_cpy_01_bad_inline_patch)))
\end{lstlisting}
\item[Patches:]~
\begin{itemize}
\item Definition for patch {\tt PRINTLINE\_PATCH}.
\begin{lstlisting}[language=lisp]
(defvar printLine_patch
  (make-instance 'clang-static-patch
    :precondition (lambda (obj location)
  (and (= location 0)
       (not (member "printLine" (asts obj)
                    :test #'string=
                    :key [#'first #'ast-declares]))))
    :free-variables 'NIL
    :includes '("<stddef.h>" "<stdio.h>")
    :types '((CLANG-TYPE
                :HASH 3615142211888308905
                :POINTER T
                :NAME "void"
                :SIZE 8)
             (CLANG-TYPE
                :HASH -1944158543856436560
                :POINTER T
                :CONST T
                :NAME "char"
                :SIZE 8))
    :macros 'NIL
    :code "void printLine (const char * line)
{
    if(line != NULL) {
        printf(\"%s\\n\", line);
    }
}"))
\end{lstlisting}
\item Definition for patch\newline{\tt CWE121\_STACK\_BASED\_BUFFER\_OVERFLOW\_\_CWE193\_CHAR\_ALLOCA\_CPY\_01\_BAD\_INLINE\_PATCH}.
\begin{lstlisting}[language=lisp]
(defvar CWE121_Stack_Based_Buffer_Overflow__CWE193_char_alloca_cpy_01_bad_inline_patch
  (make-instance 'clang-dynamic-patch
    :precondition NIL
    :cwe 121
    :conditional-code '()
    :free-variables '(("data" "*char" :-CONST :-REGISTER)
                      ("dataBadBuffer" "*char" :-CONST :-REGISTER)
                      ("dataGoodBuffer" "*char" :-CONST :-REGISTER)
                      ("source" "[11]char" :-CONST :-REGISTER))
    :includes '("<alloca.h>" "<string.h>")
    :types '((CLANG-TYPE
                :ARRAY "[11]"
                :HASH 2944235125889796353
                :POINTER NIL
                :NAME "char"
                :SIZE 11)
             (CLANG-TYPE
                :HASH -2054504279541534951
                :POINTER NIL
                :NAME "char"
                :SIZE 1)
             (CLANG-TYPE
                :HASH 5790451697626571727
                :POINTER T
                :NAME "char"
                :SIZE 8))
    :macros '((CLANG-MACRO :HASH -4911426765191714778 :NAME "SRC_STRING" :BODY "SRC_STRING \"AAAAAAAAAA\"")
              (CLANG-MACRO :HASH -342517378131665086 :NAME "ALLOCA" :BODY "ALLOCA alloca"))
    :code "dataBadBuffer = (char *)ALLOCA((10)*sizeof(char));
           dataGoodBuffer = (char *)ALLOCA((10+1)*sizeof(char));
           data = dataBadBufferdata[0] = '\\0'
   {
        source = SRC_STRING;
        /* POTENTIAL FLAW: data may not have enough space to hold source */
        strcpy(data, source);
        printLine(data);
    }"))
\end{lstlisting}
\end{itemize}
\end{description}

\subsection*{Bug Template {\tt CWE122\_HEAP\_BASED\_BUFFER\_OVERFLOW\_\_C\_CWE193\_CHAR\_CPY\_01\_BAD\_INLINE}}
\begin{description}
\item[Definition:]~\newline
\begin{lstlisting}[language=lisp]
(define-scion CWE122_Heap_Based_Buffer_Overflow__c_CWE193_char_cpy_01_bad_inline
  (make-instance 'clang-scion
    :name 'CWE122_Heap_Based_Buffer_Overflow__c_CWE193_char_cpy_01_bad_inline
    :patches (list printLine_patch CWE122_Heap_Based_Buffer_Overflow__c_CWE193_char_cpy_01_bad_inline_patch)))
\end{lstlisting}
\item[Patches:]~
\begin{itemize}
\item Definition for patch {\tt PRINTLINE\_PATCH}.
\begin{lstlisting}[language=lisp]
(defvar printLine_patch
  (make-instance 'clang-static-patch
    :precondition (lambda (obj location)
  (and (= location 0)
       (not (member "printLine" (asts obj)
                    :test #'string=
                    :key [#'first #'ast-declares]))))
    :free-variables 'NIL
    :includes '("<stddef.h>" "<stdio.h>")
    :types '((CLANG-TYPE
                :HASH 3615142211888308905
                :POINTER T
                :NAME "void"
                :SIZE 8)
             (CLANG-TYPE
                :HASH -1944158543856436560
                :POINTER T
                :CONST T
                :NAME "char"
                :SIZE 8))
    :macros 'NIL
    :code "void printLine (const char * line)
{
    if(line != NULL) {
        printf(\"%s\\n\", line);
    }
}"))
\end{lstlisting}
\item Definition for patch\newline{\tt CWE122\_HEAP\_BASED\_BUFFER\_OVERFLOW\_\_C\_CWE193\_CHAR\_CPY\_01\_BAD\_INLINE\_PATCH}.
\begin{lstlisting}[language=lisp]
(defvar CWE122_Heap_Based_Buffer_Overflow__c_CWE193_char_cpy_01_bad_inline_patch
  (make-instance 'clang-dynamic-patch
    :precondition NIL
    :cwe 122
    :conditional-code '(((((:CLASS . "BINARYOPERATOR") (:COUNTER . 5) (:FULL-STMT . T)
   (:INCLUDES "<stddef.h>") (:OPCODE . "=") (:SYN-CTX . "FULLSTMT")
  )
  "\"\""
  (((:CLASS . "DECLREFEXPR") (:COUNTER . 6) (:FULL-STMT) (:INCLUDES)
    (:OPCODE) (:SYN-CTX . "GENERIC")
   )
   "\"data\"")
  "\" = \""
  (((:CLASS . "MACROEXPANSION") (:COUNTER . 7) (:FULL-STMT) (:IN-MACRO-EXPANSION . T)
    (:INCLUDES "<stddef.h>") (:OPCODE) (:SYN-CTX . "GENERIC") (:TYPES 3615142211888308905)
   )
   "\"NULL\"")
  "\"\"") . T))
    :free-variables '(("data" "*char" :-CONST :-REGISTER) ("source" "[11]char" :-CONST :-REGISTER))
    :includes '("<stddef.h>" "<stdlib.h>" "<string.h>")
    :types '((CLANG-TYPE
                :ARRAY "[11]"
                :HASH 2944235125889796353
                :POINTER NIL
                :NAME "char"
                :SIZE 11)
             (CLANG-TYPE
                :HASH 3615142211888308905
                :POINTER T
                :NAME "void"
                :SIZE 8)
             (CLANG-TYPE
                :HASH -2054504279541534951
                :POINTER NIL
                :NAME "char"
                :SIZE 1)
             (CLANG-TYPE
                :HASH 5790451697626571727
                :POINTER T
                :NAME "char"
                :SIZE 8))
    :macros '((CLANG-MACRO :HASH -4911426765191714778 :NAME "SRC_STRING" :BODY "SRC_STRING \"AAAAAAAAAA\""))
    :code "data = NULL;
    data = (char *)malloc(10*sizeof(char));
    if (data == NULL) {
        exit(-1);
    }{
        source = SRC_STRING;
        /* POTENTIAL FLAW: data may not have enough space to hold source */
        strcpy(data, source);
        printLine(data);
        free(data);
    }"))
\end{lstlisting}
\end{itemize}
\end{description}

\subsection*{Bug Template {\tt CWE124\_BUFFER\_UNDERWRITE\_\_CHAR\_ALLOCA\_CPY\_01\_BAD\_INLINE}}
\begin{description}
\item[Definition:]~\newline
\begin{lstlisting}[language=lisp]
(define-scion CWE124_Buffer_Underwrite__char_alloca_cpy_01_bad_inline
  (make-instance 'clang-scion
    :name 'CWE124_Buffer_Underwrite__char_alloca_cpy_01_bad_inline
    :patches (list printLine_patch CWE124_Buffer_Underwrite__char_alloca_cpy_01_bad_inline_patch)))
\end{lstlisting}
\item[Patches:]~
\begin{itemize}
\item Definition for patch {\tt PRINTLINE\_PATCH}.
\begin{lstlisting}[language=lisp]
(defvar printLine_patch
  (make-instance 'clang-static-patch
    :precondition (lambda (obj location)
  (and (= location 0)
       (not (member "printLine" (asts obj)
                    :test #'string=
                    :key [#'first #'ast-declares]))))
    :free-variables 'NIL
    :includes '("<stddef.h>" "<stdio.h>")
    :types '((CLANG-TYPE
                :HASH 3615142211888308905
                :POINTER T
                :NAME "void"
                :SIZE 8)
             (CLANG-TYPE
                :HASH -1944158543856436560
                :POINTER T
                :CONST T
                :NAME "char"
                :SIZE 8))
    :macros 'NIL
    :code "void printLine (const char * line)
{
    if(line != NULL) {
        printf(\"%s\\n\", line);
    }
}"))
\end{lstlisting}
\item Definition for patch {\tt CWE124\_BUFFER\_UNDERWRITE\_\_CHAR\_ALLOCA\_CPY\_01\_BAD\_INLINE\_PATCH}.
\begin{lstlisting}[language=lisp]
(defvar CWE124_Buffer_Underwrite__char_alloca_cpy_01_bad_inline_patch
  (make-instance 'clang-dynamic-patch
    :precondition NIL
    :cwe 124
    :conditional-code '()
    :free-variables '(("data" "*char" :-CONST :-REGISTER)
                      ("dataBuffer" "*char" :-CONST :-REGISTER)
                      ("source" "[100]char" :-CONST :-REGISTER))
    :includes '("<alloca.h>" "<string.h>")
    :types '((CLANG-TYPE
                :ARRAY "[100]"
                :HASH 6253389274476629705
                :POINTER NIL
                :NAME "char"
                :SIZE 100)
             (CLANG-TYPE
                :HASH -2054504279541534951
                :POINTER NIL
                :NAME "char"
                :SIZE 1)
             (CLANG-TYPE
                :HASH 5790451697626571727
                :POINTER T
                :NAME "char"
                :SIZE 8))
    :macros '((CLANG-MACRO :HASH -342517378131665086 :NAME "ALLOCA" :BODY "ALLOCA alloca"))
    :code "dataBuffer = (char *)ALLOCA(100*sizeof(char));
           memset(dataBuffer, 'A', 100-1);
           dataBuffer[100-1] = '\\0';
           data = dataBuffer - 8;
   {
        
        memset(source, 'C', 100-1); /* fill with 'C's */
        source[100-1] = '\\0'; /* null terminate */
        /* POTENTIAL FLAW: Possibly copying data to memory before the destination buffer */
        strcpy(data, source);
        printLine(data);
    }"))
\end{lstlisting}
\end{itemize}
\end{description}

\subsection*{Bug Template {\tt CWE126\_BUFFER\_OVERREAD\_\_CHAR\_ALLOCA\_LOOP\_01\_BAD\_INLINE}}
\begin{description}
\item[Definition:]~\newline
\begin{lstlisting}[language=lisp]
(define-scion CWE126_Buffer_Overread__char_alloca_loop_01_bad_inline
  (make-instance 'clang-scion
    :name 'CWE126_Buffer_Overread__char_alloca_loop_01_bad_inline
    :patches (list printLine_patch CWE126_Buffer_Overread__char_alloca_loop_01_bad_inline_patch)))
\end{lstlisting}
\item[Patches:]~
\begin{itemize}
\item Definition for patch {\tt PRINTLINE\_PATCH}.
\begin{lstlisting}[language=lisp]
(defvar printLine_patch
  (make-instance 'clang-static-patch
    :precondition (lambda (obj location)
  (and (= location 0)
       (not (member "printLine" (asts obj)
                    :test #'string=
                    :key [#'first #'ast-declares]))))
    :free-variables 'NIL
    :includes '("<stddef.h>" "<stdio.h>")
    :types '((CLANG-TYPE
                :HASH 3615142211888308905
                :POINTER T
                :NAME "void"
                :SIZE 8)
             (CLANG-TYPE
                :HASH -1944158543856436560
                :POINTER T
                :CONST T
                :NAME "char"
                :SIZE 8))
    :macros 'NIL
    :code "void printLine (const char * line)
{
    if(line != NULL) {
        printf(\"%s\\n\", line);
    }
}"))
\end{lstlisting}
\item Definition for patch {\tt CWE126\_BUFFER\_OVERREAD\_\_CHAR\_ALLOCA\_LOOP\_01\_BAD\_INLINE\_PATCH}.
\begin{lstlisting}[language=lisp]
(defvar CWE126_Buffer_Overread__char_alloca_loop_01_bad_inline_patch
  (make-instance 'clang-dynamic-patch
    :precondition NIL
    :cwe 126
    :conditional-code '()
    :free-variables '(("data" "*char" :-CONST :-REGISTER)
                      ("dataBadBuffer" "*char" :-CONST :-REGISTER)
                      ("dataGoodBuffer" "*char" :-CONST :-REGISTER)
                      ("i" "size_t" :-CONST :-REGISTER)
                      ("destLen" "size_t" :-CONST :-REGISTER)
                      ("dest" "[100]char" :-CONST :-REGISTER))
    :includes '("<alloca.h>" "<string.h>")
    :types '((CLANG-TYPE
                :ARRAY "[100]"
                :HASH 6253389274476629705
                :POINTER NIL
                :NAME "char"
                :SIZE 100)
             (CLANG-TYPE
                :COL 1
                :DECL NIL
                :FILE "/usr/bin/../lib/clang/6.0.1/include/stddef.h"
                :LINE 62
                :HASH 764611252874068922
                :I-FILE "<stddef.h>"
                :POINTER NIL
                :NAME "size_t"
                :SIZE 8)
             (CLANG-TYPE
                :HASH -2054504279541534951
                :POINTER NIL
                :NAME "char"
                :SIZE 1)
             (CLANG-TYPE
                :HASH 5790451697626571727
                :POINTER T
                :NAME "char"
                :SIZE 8))
    :macros '((CLANG-MACRO :HASH -342517378131665086 :NAME "ALLOCA" :BODY "ALLOCA alloca"))
    :code "dataBadBuffer = (char *)ALLOCA(50*sizeof(char));
        dataGoodBuffer = (char *)ALLOCA(100*sizeof(char));
        memset(dataBadBuffer, 'A', 50-1);
        dataBadBuffer[50-1] = '\\0';
        memset(dataGoodBuffer, 'A', 100-1);
        dataGoodBuffer[100-1] = '\\0';
        data = dataBadBuffer
   {
        
        
        memset(dest, 'C', 100-1);
        dest[100-1] = '\\0'; /* null terminate */
        destLen = strlen(dest);
        /* POTENTIAL FLAW: using length of the dest where data
         * could be smaller than dest causing buffer overread */
        for (i = 0; i < destLen; i++) {
            dest[i] = data[i];
        }
        dest[100-1] = '\\0';
        printLine(dest);
    }"))
\end{lstlisting}
\end{itemize}
\end{description}

\subsection*{Bug Template {\tt CWE127\_BUFFER\_UNDERREAD\_\_CHAR\_ALLOCA\_CPY\_01\_BAD\_INLINE}}
\begin{description}
\item[Definition:]~\newline
\begin{lstlisting}[language=lisp]
(define-scion CWE127_Buffer_Underread__char_alloca_cpy_01_bad_inline
  (make-instance 'clang-scion
    :name 'CWE127_Buffer_Underread__char_alloca_cpy_01_bad_inline
    :patches (list printLine_patch CWE127_Buffer_Underread__char_alloca_cpy_01_bad_inline_patch)))
\end{lstlisting}
\item[Patches:]~
\begin{itemize}
\item Definition for patch {\tt PRINTLINE\_PATCH}.
\begin{lstlisting}[language=lisp]
(defvar printLine_patch
  (make-instance 'clang-static-patch
    :precondition (lambda (obj location)
  (and (= location 0)
       (not (member "printLine" (asts obj)
                    :test #'string=
                    :key [#'first #'ast-declares]))))
    :free-variables 'NIL
    :includes '("<stddef.h>" "<stdio.h>")
    :types '((CLANG-TYPE
                :HASH 3615142211888308905
                :POINTER T
                :NAME "void"
                :SIZE 8)
             (CLANG-TYPE
                :HASH -1944158543856436560
                :POINTER T
                :CONST T
                :NAME "char"
                :SIZE 8))
    :macros 'NIL
    :code "void printLine (const char * line)
{
    if(line != NULL) {
        printf(\"%s\\n\", line);
    }
}"))
\end{lstlisting}
\item Definition for patch {\tt CWE127\_BUFFER\_UNDERREAD\_\_CHAR\_ALLOCA\_CPY\_01\_BAD\_INLINE\_PATCH}.
\begin{lstlisting}[language=lisp]
(defvar CWE127_Buffer_Underread__char_alloca_cpy_01_bad_inline_patch
  (make-instance 'clang-dynamic-patch
    :precondition NIL
    :cwe 127
    :conditional-code '()
    :free-variables '(("data" "*char" :-CONST :-REGISTER)
                      ("dataBuffer" "*char" :-CONST :-REGISTER)
                      ("dest" "[200]char" :-CONST :-REGISTER))
    :includes '("<alloca.h>" "<string.h>")
    :types '((CLANG-TYPE
                :ARRAY "[200]"
                :HASH 349279012212144110
                :POINTER NIL
                :NAME "char"
                :SIZE 200)
             (CLANG-TYPE
                :HASH -2054504279541534951
                :POINTER NIL
                :NAME "char"
                :SIZE 1)
             (CLANG-TYPE
                :HASH 5790451697626571727
                :POINTER T
                :NAME "char"
                :SIZE 8))
    :macros '((CLANG-MACRO :HASH -342517378131665086 :NAME "ALLOCA" :BODY "ALLOCA alloca"))
    :code "dataBuffer = (char *)ALLOCA(100*sizeof(char));
           memset(dataBuffer, 'A', 100-1);
           dataBuffer[100-1] = '\\0';
           data = dataBuffer - 8;
   {
        
        memset(dest, 'C', 100*2-1); /* fill with 'C's */
        dest[100*2-1] = '\\0'; /* null terminate */
        /* POTENTIAL FLAW: Possibly copy from a memory location located before the source buffer */
        strcpy(dest, data);
        printLine(dest);
    }"))
\end{lstlisting}
\end{itemize}
\end{description}

\subsection*{Bug Template {\tt CWE190\_INTEGER\_OVERFLOW\_\_INT\_RAND\_ADD\_01\_BAD\_INLINE}}
\begin{description}
\item[Definition:]~\newline
\begin{lstlisting}[language=lisp]
(define-scion CWE190_Integer_Overflow__int_rand_add_01_bad_inline
  (make-instance 'clang-scion
    :name 'CWE190_Integer_Overflow__int_rand_add_01_bad_inline
    :patches (list printIntLine_patch CWE190_Integer_Overflow__int_rand_add_01_bad_inline_patch)))
\end{lstlisting}
\item[Patches:]~
\begin{itemize}
\item Definition for patch {\tt PRINTINTLINE\_PATCH}.
\begin{lstlisting}[language=lisp]
(defvar printIntLine_patch
  (make-instance 'clang-static-patch
    :precondition (lambda (obj location)
  (and (= location 0)
       (not (member "printIntLine" (asts obj)
                    :test #'string=
                    :key [#'first #'ast-declares]))))
    :free-variables 'NIL
    :includes '("<stdio.h>")
    :types '((CLANG-TYPE
                :HASH -1958391046879680490
                :POINTER NIL
                :NAME "int"
                :SIZE 4))
    :macros 'NIL
    :code "void printIntLine (int intNumber)
{
    printf(\"%d\\n\", intNumber);
}"))
\end{lstlisting}
\item Definition for patch {\tt CWE190\_INTEGER\_OVERFLOW\_\_INT\_RAND\_ADD\_01\_BAD\_INLINE\_PATCH}.
\begin{lstlisting}[language=lisp]
(defvar CWE190_Integer_Overflow__int_rand_add_01_bad_inline_patch
  (make-instance 'clang-dynamic-patch
    :precondition NIL
    :cwe 190
    :conditional-code '(((((:CLASS . "BINARYOPERATOR") (:COUNTER . 5) (:FULL-STMT . T) (:INCLUDES)
   (:OPCODE . "=") (:SYN-CTX . "FULLSTMT")
  )
  "\"\""
  (((:CLASS . "DECLREFEXPR") (:COUNTER . 6) (:FULL-STMT) (:INCLUDES)
    (:OPCODE) (:SYN-CTX . "GENERIC")
   )
   "\"data\"")
  "\" = \""
  (((:CLASS . "INTEGERLITERAL") (:COUNTER . 7) (:FULL-STMT) (:INCLUDES)
    (:OPCODE) (:SYN-CTX . "GENERIC")
   )
   "\"0\"")
  "\"\"") . T))
    :free-variables '(("data" "int" :-CONST :-REGISTER) ("result" "int" :-CONST :-REGISTER))
    :includes '("<stdlib.h>")
    :types '((CLANG-TYPE
                :HASH -1958391046879680490
                :POINTER NIL
                :NAME "int"
                :SIZE 4)
             (CLANG-TYPE
                :HASH -760642589583846522
                :POINTER NIL
                :NAME "unsigned int"
                :SIZE 4))
    :macros '((CLANG-MACRO :HASH 2308996158549424241 :NAME "URAND31"
                           :BODY "URAND31() (((unsigned)rand()<<30) ^ ((unsigned)rand()<<15) ^ rand())")
              (CLANG-MACRO :HASH 1124813122759813294 :NAME "RAND32"
                           :BODY "RAND32() ((int)(rand() & 1 ? URAND31() : -URAND31() - 1))"))
    :code "data = 0;
    data = RAND32();
    {
        /* POTENTIAL FLAW: Adding 1 to data could cause an overflow */
        result = data + 1;
        printIntLine(result);
    }"))
\end{lstlisting}
\end{itemize}
\end{description}

\subsection*{Bug Template {\tt CWE191\_INTEGER\_UNDERFLOW\_\_INT\_RAND\_MULTIPLY\_01\_BAD\_INLINE}}
\begin{description}
\item[Definition:]~\newline
\begin{lstlisting}[language=lisp]
(define-scion CWE191_Integer_Underflow__int_rand_multiply_01_bad_inline
  (make-instance 'clang-scion
    :name 'CWE191_Integer_Underflow__int_rand_multiply_01_bad_inline
    :patches (list printIntLine_patch CWE191_Integer_Underflow__int_rand_multiply_01_bad_inline_patch)))
\end{lstlisting}
\item[Patches:]~
\begin{itemize}
\item Definition for patch {\tt PRINTINTLINE\_PATCH}.
\begin{lstlisting}[language=lisp]
(defvar printIntLine_patch
  (make-instance 'clang-static-patch
    :precondition (lambda (obj location)
  (and (= location 0)
       (not (member "printIntLine" (asts obj)
                    :test #'string=
                    :key [#'first #'ast-declares]))))
    :free-variables 'NIL
    :includes '("<stdio.h>")
    :types '((CLANG-TYPE
                :HASH -1958391046879680490
                :POINTER NIL
                :NAME "int"
                :SIZE 4))
    :macros 'NIL
    :code "void printIntLine (int intNumber)
{
    printf(\"%d\\n\", intNumber);
}"))
\end{lstlisting}
\item Definition for patch {\tt CWE191\_INTEGER\_UNDERFLOW\_\_INT\_RAND\_MULTIPLY\_01\_BAD\_INLINE\_PATCH}.
\begin{lstlisting}[language=lisp]
(defvar CWE191_Integer_Underflow__int_rand_multiply_01_bad_inline_patch
  (make-instance 'clang-dynamic-patch
    :precondition NIL
    :cwe 191
    :conditional-code '(((((:CLASS . "BINARYOPERATOR") (:COUNTER . 5) (:FULL-STMT . T) (:INCLUDES)
   (:OPCODE . "=") (:SYN-CTX . "FULLSTMT")
  )
  "\"\""
  (((:CLASS . "DECLREFEXPR") (:COUNTER . 6) (:FULL-STMT) (:INCLUDES)
    (:OPCODE) (:SYN-CTX . "GENERIC")
   )
   "\"data\"")
  "\" = \""
  (((:CLASS . "INTEGERLITERAL") (:COUNTER . 7) (:FULL-STMT) (:INCLUDES)
    (:OPCODE) (:SYN-CTX . "GENERIC")
   )
   "\"0\"")
  "\"\"") . T))
    :free-variables '(("data" "int" :-CONST :-REGISTER) ("result" "int" :-CONST :-REGISTER))
    :includes '("<stdlib.h>")
    :types '((CLANG-TYPE
                :HASH -1958391046879680490
                :POINTER NIL
                :NAME "int"
                :SIZE 4)
             (CLANG-TYPE
                :HASH -760642589583846522
                :POINTER NIL
                :NAME "unsigned int"
                :SIZE 4))
    :macros '((CLANG-MACRO :HASH 2308996158549424241 :NAME "URAND31"
                           :BODY "URAND31() (((unsigned)rand()<<30) ^ ((unsigned)rand()<<15) ^ rand())")
              (CLANG-MACRO :HASH 1124813122759813294 :NAME "RAND32"
                           :BODY "RAND32() ((int)(rand() & 1 ? URAND31() : -URAND31() - 1))"))
    :code "data = 0;
    data = RAND32();
    if(data < 0) { /* ensure we won't have an overflow */
        /* POTENTIAL FLAW: if (data * 2) < INT_MIN, this will underflow */
        result = data * 2;
        printIntLine(result);
    }"))
\end{lstlisting}
\end{itemize}
\end{description}

\subsection*{Bug Template {\tt CWE195\_SIGNED\_TO\_UNSIGNED\_CONVERSION\_ERROR\_\_RAND\_MALLOC\_01\_BAD\_INLINE}}
\begin{description}
\item[Definition:]~\newline
\begin{lstlisting}[language=lisp]
(define-scion CWE195_Signed_to_Unsigned_Conversion_Error__rand_malloc_01_bad_inline
  (make-instance 'clang-scion
    :name 'CWE195_Signed_to_Unsigned_Conversion_Error__rand_malloc_01_bad_inline
    :patches (list printLine_patch CWE195_Signed_to_Unsigned_Conversion_Error__rand_malloc_01_bad_inline_patch)))
\end{lstlisting}
\item[Patches:]~
\begin{itemize}
\item Definition for patch {\tt PRINTLINE\_PATCH}.
\begin{lstlisting}[language=lisp]
(defvar printLine_patch
  (make-instance 'clang-static-patch
    :precondition (lambda (obj location)
  (and (= location 0)
       (not (member "printLine" (asts obj)
                    :test #'string=
                    :key [#'first #'ast-declares]))))
    :free-variables 'NIL
    :includes '("<stddef.h>" "<stdio.h>")
    :types '((CLANG-TYPE
                :HASH 3615142211888308905
                :POINTER T
                :NAME "void"
                :SIZE 8)
             (CLANG-TYPE
                :HASH -1944158543856436560
                :POINTER T
                :CONST T
                :NAME "char"
                :SIZE 8))
    :macros 'NIL
    :code "void printLine (const char * line)
{
    if(line != NULL) {
        printf(\"%s\\n\", line);
    }
}"))
\end{lstlisting}
\item Definition for patch\newline{\tt CWE195\_SIGNED\_TO\_UNSIGNED\_CONVERSION\_ERROR\_\_RAND\_MALLOC\_01\_BAD\_INLINE\_PATCH}.
\begin{lstlisting}[language=lisp]
(defvar CWE195_Signed_to_Unsigned_Conversion_Error__rand_malloc_01_bad_inline_patch
  (make-instance 'clang-dynamic-patch
    :precondition NIL
    :cwe 195
    :conditional-code '(((((:CLASS . "BINARYOPERATOR") (:COUNTER . 5) (:FULL-STMT . T) (:INCLUDES)
   (:OPCODE . "=") (:SYN-CTX . "FULLSTMT")
  )
  "\"\""
  (((:CLASS . "DECLREFEXPR") (:COUNTER . 6) (:FULL-STMT) (:INCLUDES)
    (:OPCODE) (:SYN-CTX . "GENERIC")
   )
   "\"data\"")
  "\" = \""
  (((:CLASS . "UNARYOPERATOR") (:COUNTER . 7) (:FULL-STMT) (:INCLUDES)
    (:OPCODE . "-") (:SYN-CTX . "GENERIC")
   )
   "\"-\""
   (((:CLASS . "INTEGERLITERAL") (:COUNTER . 8) (:FULL-STMT) (:INCLUDES)
     (:OPCODE) (:SYN-CTX . "GENERIC")
    )
    "\"1\"")
   "\"\"")
  "\"\"") . T))
    :free-variables '(("data" "int" :-CONST :-REGISTER) ("dataBuffer" "*char" :-CONST :-REGISTER))
    :includes '("<stddef.h>" "<stdlib.h>" "<string.h>")
    :types '((CLANG-TYPE
                :HASH 3615142211888308905
                :POINTER T
                :NAME "void"
                :SIZE 8)
             (CLANG-TYPE
                :HASH 5790451697626571727
                :POINTER T
                :NAME "char"
                :SIZE 8)
             (CLANG-TYPE
                :HASH -760642589583846522
                :POINTER NIL
                :NAME "unsigned int"
                :SIZE 4)
             (CLANG-TYPE
                :HASH -1958391046879680490
                :POINTER NIL
                :NAME "int"
                :SIZE 4))
    :macros '((CLANG-MACRO :HASH 2308996158549424241 :NAME "URAND31"
                           :BODY "URAND31() (((unsigned)rand()<<30) ^ ((unsigned)rand()<<15) ^ rand())")
              (CLANG-MACRO :HASH 1124813122759813294 :NAME "RAND32"
                           :BODY "RAND32() ((int)(rand() & 1 ? URAND31() : -URAND31() - 1))"))
    :code "data = -1;
    data = RAND32();
    if (data < 100) {
        /* POTENTIAL FLAW: malloc() takes a size_t (unsigned int) as input and therefore if it is negative,
         * the conversion will cause malloc() to allocate a very large amount of data or fail */
        dataBuffer = (char *)malloc(data);
        if (dataBuffer == NULL) {
            exit(-1);
        }
        /* Do something with dataBuffer */
        memset(dataBuffer, 'A', data-1);
        dataBuffer[data-1] = '\\0';
        printLine(dataBuffer);
        free(dataBuffer);
    }"))
\end{lstlisting}
\end{itemize}
\end{description}

\subsection*{Bug Template {\tt CWE196\_UNSIGNED\_TO\_SIGNED\_CONVERSION\_ERROR\_\_BASIC\_01\_BAD\_INLINE}}
\begin{description}
\item[Definition:]~\newline
\begin{lstlisting}[language=lisp]
(define-scion CWE196_Unsigned_to_Signed_Conversion_Error__basic_01_bad_inline
  (make-instance 'clang-scion
    :name 'CWE196_Unsigned_to_Signed_Conversion_Error__basic_01_bad_inline
    :patches (list printIntLine_patch CWE196_Unsigned_to_Signed_Conversion_Error__basic_01_bad_inline_patch)))
\end{lstlisting}
\item[Patches:]~
\begin{itemize}
\item Definition for patch {\tt PRINTINTLINE\_PATCH}.
\begin{lstlisting}[language=lisp]
(defvar printIntLine_patch
  (make-instance 'clang-static-patch
    :precondition (lambda (obj location)
  (and (= location 0)
       (not (member "printIntLine" (asts obj)
                    :test #'string=
                    :key [#'first #'ast-declares]))))
    :free-variables 'NIL
    :includes '("<stdio.h>")
    :types '((CLANG-TYPE
                :HASH -1958391046879680490
                :POINTER NIL
                :NAME "int"
                :SIZE 4))
    :macros 'NIL
    :code "void printIntLine (int intNumber)
{
    printf(\"%d\\n\", intNumber);
}"))
\end{lstlisting}
\item Definition for patch {\tt CWE196\_UNSIGNED\_TO\_SIGNED\_CONVERSION\_ERROR\_\_BASIC\_01\_BAD\_INLINE\_PATCH}.
\begin{lstlisting}[language=lisp]
(defvar CWE196_Unsigned_to_Signed_Conversion_Error__basic_01_bad_inline_patch
  (make-instance 'clang-dynamic-patch
    :precondition NIL
    :cwe 196
    :conditional-code '()
    :free-variables '(("intUnsigned" "unsigned int" :-CONST :-REGISTER) ("intSigned" "int" :-CONST :-REGISTER))
    :includes '("<limits.h>" "<stdlib.h>")
    :types '((CLANG-TYPE
                :HASH -1958391046879680490
                :POINTER NIL
                :NAME "int"
                :SIZE 4)
             (CLANG-TYPE
                :HASH -760642589583846522
                :POINTER NIL
                :NAME "unsigned int"
                :SIZE 4))
    :macros 'NIL
    :code "{
        
        
        intUnsigned = rand();
        if (rand() % 2 == 0) {
            intUnsigned = UINT_MAX - intUnsigned;
        }
        /* FLAW: intUnsigned could be very large, in which case intSigned will be negative */
        intSigned = intUnsigned;
        printIntLine(intSigned);
    }"))
\end{lstlisting}
\end{itemize}
\end{description}

\subsection*{Bug Template {\tt CWE197\_NUMERIC\_TRUNCATION\_ERROR\_\_INT\_RAND\_TO\_CHAR\_01\_BAD\_INLINE}}
\begin{description}
\item[Definition:]~\newline
\begin{lstlisting}[language=lisp]
(define-scion CWE197_Numeric_Truncation_Error__int_rand_to_char_01_bad_inline
  (make-instance 'clang-scion
    :name 'CWE197_Numeric_Truncation_Error__int_rand_to_char_01_bad_inline
    :patches (list printHexCharLine_patch CWE197_Numeric_Truncation_Error__int_rand_to_char_01_bad_inline_patch)))
\end{lstlisting}
\item[Patches:]~
\begin{itemize}
\item Definition for patch {\tt PRINTHEXCHARLINE\_PATCH}.
\begin{lstlisting}[language=lisp]
(defvar printHexCharLine_patch
  (make-instance 'clang-static-patch
    :precondition (lambda (obj location)
  (and (= location 0)
       (not (member "printHexCharLine" (asts obj)
                    :test #'string=
                    :key [#'first #'ast-declares]))))
    :free-variables 'NIL
    :includes '("<stdio.h>")
    :types '((CLANG-TYPE
                :HASH -2054504279541534951
                :POINTER NIL
                :NAME "char"
                :SIZE 1))
    :macros 'NIL
    :code "void printHexCharLine (char charHex)
{
    printf(\"%02x\\n\", charHex);
}"))
\end{lstlisting}
\item Definition for patch {\tt CWE197\_NUMERIC\_TRUNCATION\_ERROR\_\_INT\_RAND\_TO\_CHAR\_01\_BAD\_INLINE\_PATCH}.
\begin{lstlisting}[language=lisp]
(defvar CWE197_Numeric_Truncation_Error__int_rand_to_char_01_bad_inline_patch
  (make-instance 'clang-dynamic-patch
    :precondition NIL
    :cwe 197
    :conditional-code '(((((:CLASS . "BINARYOPERATOR") (:COUNTER . 5) (:FULL-STMT . T) (:INCLUDES)
   (:OPCODE . "=") (:SYN-CTX . "FULLSTMT")
  )
  "\"\""
  (((:CLASS . "DECLREFEXPR") (:COUNTER . 6) (:FULL-STMT) (:INCLUDES)
    (:OPCODE) (:SYN-CTX . "GENERIC")
   )
   "\"data\"")
  "\" = \""
  (((:CLASS . "UNARYOPERATOR") (:COUNTER . 7) (:FULL-STMT) (:INCLUDES)
    (:OPCODE . "-") (:SYN-CTX . "GENERIC")
   )
   "\"-\""
   (((:CLASS . "INTEGERLITERAL") (:COUNTER . 8) (:FULL-STMT) (:INCLUDES)
     (:OPCODE) (:SYN-CTX . "GENERIC")
    )
    "\"1\"")
   "\"\"")
  "\"\"") . T))
    :free-variables '(("data" "int" :-CONST :-REGISTER) ("charData" "char" :-CONST :-REGISTER))
    :includes '("<stdlib.h>")
    :types '((CLANG-TYPE
                :HASH -2054504279541534951
                :POINTER NIL
                :NAME "char"
                :SIZE 1)
             (CLANG-TYPE
                :HASH -760642589583846522
                :POINTER NIL
                :NAME "unsigned int"
                :SIZE 4)
             (CLANG-TYPE
                :HASH -1958391046879680490
                :POINTER NIL
                :NAME "int"
                :SIZE 4))
    :macros '((CLANG-MACRO :HASH 2308996158549424241 :NAME "URAND31"
                           :BODY "URAND31() (((unsigned)rand()<<30) ^ ((unsigned)rand()<<15) ^ rand())")
              (CLANG-MACRO :HASH 1124813122759813294 :NAME "RAND32"
                           :BODY "RAND32() ((int)(rand() & 1 ? URAND31() : -URAND31() - 1))"))
    :code "data = -1;
    data = RAND32();
    {
        /* POTENTIAL FLAW: Convert data to a char, possibly causing a truncation error */
        charData = (char)data;
        printHexCharLine(charData);
    }"))
\end{lstlisting}
\end{itemize}
\end{description}

\subsection*{Bug Template {\tt CWE252\_UNCHECKED\_RETURN\_VALUE\_\_CHAR\_FPRINTF\_01\_BAD\_INLINE}}
\begin{description}
\item[Definition:]~\newline
\begin{lstlisting}[language=lisp]
(define-scion CWE252_Unchecked_Return_Value__char_fprintf_01_bad_inline
  (make-instance 'clang-scion
    :name 'CWE252_Unchecked_Return_Value__char_fprintf_01_bad_inline
    :patches (list CWE252_Unchecked_Return_Value__char_fprintf_01_bad_inline_patch)))
\end{lstlisting}
\item[Patches:]~
\begin{itemize}
\item Definition for patch {\tt CWE252\_UNCHECKED\_RETURN\_VALUE\_\_CHAR\_FPRINTF\_01\_BAD\_INLINE\_PATCH}.
\begin{lstlisting}[language=lisp]
(defvar CWE252_Unchecked_Return_Value__char_fprintf_01_bad_inline_patch
  (make-instance 'clang-dynamic-patch
    :precondition NIL
    :cwe 252
    :conditional-code '()
    :free-variables 'NIL
    :includes '("<stdio.h>")
    :types 'NIL
    :macros 'NIL
    :code "fprintf(stdout, \"%s\\n\", \"string\")"))
\end{lstlisting}
\end{itemize}
\end{description}

\subsection*{Bug Template {\tt CWE253\_INCORRECT\_CHECK\_OF\_FUNCTION\_RETURN\_VALUE\_\_CHAR\_FPRINTF\_01\_BAD\_INLINE}}
\begin{description}
\item[Definition:]~\newline
\begin{lstlisting}[language=lisp]
(define-scion CWE253_Incorrect_Check_of_Function_Return_Value__char_fprintf_01_bad_inline
  (make-instance 'clang-scion
    :name 'CWE253_Incorrect_Check_of_Function_Return_Value__char_fprintf_01_bad_inline
    :patches (list printLine_patch CWE253_Incorrect_Check_of_Function_Return_Value__char_fprintf_01_bad_inline_patch)))
\end{lstlisting}
\item[Patches:]~
\begin{itemize}
\item Definition for patch {\tt PRINTLINE\_PATCH}.
\begin{lstlisting}[language=lisp]
(defvar printLine_patch
  (make-instance 'clang-static-patch
    :precondition (lambda (obj location)
  (and (= location 0)
       (not (member "printLine" (asts obj)
                    :test #'string=
                    :key [#'first #'ast-declares]))))
    :free-variables 'NIL
    :includes '("<stddef.h>" "<stdio.h>")
    :types '((CLANG-TYPE
                :HASH 3615142211888308905
                :POINTER T
                :NAME "void"
                :SIZE 8)
             (CLANG-TYPE
                :HASH -1944158543856436560
                :POINTER T
                :CONST T
                :NAME "char"
                :SIZE 8))
    :macros 'NIL
    :code "void printLine (const char * line)
{
    if(line != NULL) {
        printf(\"%s\\n\", line);
    }
}"))
\end{lstlisting}
\item Definition for patch\newline{\tt CWE253\_INCORRECT\_CHECK\_OF\_FUNCTION\_RETURN\_VALUE\_\_CHAR\_FPRINTF\_01\_BAD\_INLINE\_PATCH}.
\begin{lstlisting}[language=lisp]
(defvar CWE253_Incorrect_Check_of_Function_Return_Value__char_fprintf_01_bad_inline_patch
  (make-instance 'clang-dynamic-patch
    :precondition NIL
    :cwe 253
    :conditional-code '()
    :free-variables 'NIL
    :includes '("<stdio.h>")
    :types 'NIL
    :macros 'NIL
    :code "if (fprintf(stdout, \"%s\\n\", \"string\") == 0) {
        printLine(\"fprintf failed!\");
    }"))
\end{lstlisting}
\end{itemize}
\end{description}

\subsection*{Bug Template {\tt CWE367\_TOC\_TOU\_\_ACCESS\_01\_BAD\_INLINE}}
\begin{description}
\item[Definition:]~\newline
\begin{lstlisting}[language=lisp]
(define-scion CWE367_TOC_TOU__access_01_bad_inline
  (make-instance 'clang-scion
    :name 'CWE367_TOC_TOU__access_01_bad_inline
    :patches (list printLine_patch CWE367_TOC_TOU__access_01_bad_inline_patch)))
\end{lstlisting}
\item[Patches:]~
\begin{itemize}
\item Definition for patch {\tt PRINTLINE\_PATCH}.
\begin{lstlisting}[language=lisp]
(defvar printLine_patch
  (make-instance 'clang-static-patch
    :precondition (lambda (obj location)
  (and (= location 0)
       (not (member "printLine" (asts obj)
                    :test #'string=
                    :key [#'first #'ast-declares]))))
    :free-variables 'NIL
    :includes '("<stddef.h>" "<stdio.h>")
    :types '((CLANG-TYPE
                :HASH 3615142211888308905
                :POINTER T
                :NAME "void"
                :SIZE 8)
             (CLANG-TYPE
                :HASH -1944158543856436560
                :POINTER T
                :CONST T
                :NAME "char"
                :SIZE 8))
    :macros 'NIL
    :code "void printLine (const char * line)
{
    if(line != NULL) {
        printf(\"%s\\n\", line);
    }
}"))
\end{lstlisting}
\item Definition for patch {\tt CWE367\_TOC\_TOU\_\_ACCESS\_01\_BAD\_INLINE\_PATCH}.
\begin{lstlisting}[language=lisp]
(defvar CWE367_TOC_TOU__access_01_bad_inline_patch
  (make-instance 'clang-dynamic-patch
    :precondition NIL
    :cwe 367
    :conditional-code '()
    :free-variables '(("filename" "[100]char" :-CONST :-REGISTER) ("fileDesc" "int" :-CONST :-REGISTER))
    :includes '("<fcntl.h>" "<stddef.h>" "<stdio.h>" "<stdlib.h>" "<string.h>" "<unistd.h>")
    :types '((CLANG-TYPE
                :HASH 3615142211888308905
                :POINTER T
                :NAME "void"
                :SIZE 8)
             (CLANG-TYPE
                :HASH -1958391046879680490
                :POINTER NIL
                :NAME "int"
                :SIZE 4)
             (CLANG-TYPE
                :ARRAY "[100]"
                :HASH 6253389274476629705
                :POINTER NIL
                :NAME "char"
                :SIZE 100))
    :macros '((CLANG-MACRO :HASH -7379358396012845812 :NAME "CLOSE" :BODY "CLOSE close")
              (CLANG-MACRO :HASH -2251689809414035892 :NAME "BAD_SINK_STRING" :BODY "BAD_SINK_STRING \"Bad Sink...\"")
              (CLANG-MACRO :HASH 7993643387143623974 :NAME "WRITE" :BODY "WRITE write")
              (CLANG-MACRO :HASH 1558538643793173296 :NAME "OPEN" :BODY "OPEN open")
              (CLANG-MACRO :HASH -3165941349971436421 :NAME "ACCESS" :BODY "ACCESS access")
              (CLANG-MACRO :HASH 3525616155471961188 :NAME "GOOD_SINK_STRING" :BODY "GOOD_SINK_STRING \"Good Sink...\"")
              (CLANG-MACRO :HASH 4723192209568994710 :NAME "STAT" :BODY "STAT stat"))
    :code "{
        filename = \"\";
        fileDesc = -1;
        if (fgets(filename, 100, stdin) == NULL) {
            printLine(\"fgets() failed\");
            /* Restore NUL terminator if fgets fails */
            filename[0] = '\\0';
        }
        if (strlen(filename) > 0) {
            filename[strlen(filename)-1] = '\\0'; /* remove newline */
        }
        /* FLAW: Open and write to the file after checking the status information */
        if (ACCESS(filename, W_OK) == -1) {
            exit(1);
        }
        fileDesc  = OPEN(filename, O_RDWR);
        if (fileDesc == -1) {
            exit(1);
        }
        if (WRITE(fileDesc, BAD_SINK_STRING, strlen(BAD_SINK_STRING)) == -1) {
            exit(1);
        }
        if (fileDesc != -1) {
            CLOSE(fileDesc);
        }
    }"))
\end{lstlisting}
\end{itemize}
\end{description}

\subsection*{Bug Template {\tt CWE369\_DIVIDE\_BY\_ZERO\_\_INT\_RAND\_DIVIDE\_01\_BAD\_INLINE}}
\begin{description}
\item[Definition:]~\newline
\begin{lstlisting}[language=lisp]
(define-scion CWE369_Divide_by_Zero__int_rand_divide_01_bad_inline
  (make-instance 'clang-scion
    :name 'CWE369_Divide_by_Zero__int_rand_divide_01_bad_inline
    :patches (list printIntLine_patch CWE369_Divide_by_Zero__int_rand_divide_01_bad_inline_patch)))
\end{lstlisting}
\item[Patches:]~
\begin{itemize}
\item Definition for patch {\tt PRINTINTLINE\_PATCH}.
\begin{lstlisting}[language=lisp]
(defvar printIntLine_patch
  (make-instance 'clang-static-patch
    :precondition (lambda (obj location)
  (and (= location 0)
       (not (member "printIntLine" (asts obj)
                    :test #'string=
                    :key [#'first #'ast-declares]))))
    :free-variables 'NIL
    :includes '("<stdio.h>")
    :types '((CLANG-TYPE
                :HASH -1958391046879680490
                :POINTER NIL
                :NAME "int"
                :SIZE 4))
    :macros 'NIL
    :code "void printIntLine (int intNumber)
{
    printf(\"%d\\n\", intNumber);
}"))
\end{lstlisting}
\item Definition for patch {\tt CWE369\_DIVIDE\_BY\_ZERO\_\_INT\_RAND\_DIVIDE\_01\_BAD\_INLINE\_PATCH}.
\begin{lstlisting}[language=lisp]
(defvar CWE369_Divide_by_Zero__int_rand_divide_01_bad_inline_patch
  (make-instance 'clang-dynamic-patch
    :precondition NIL
    :cwe 369
    :conditional-code '(((((:CLASS . "BINARYOPERATOR") (:COUNTER . 5) (:FULL-STMT . T) (:INCLUDES)
   (:OPCODE . "=") (:SYN-CTX . "FULLSTMT")
  )
  "\"\""
  (((:CLASS . "DECLREFEXPR") (:COUNTER . 6) (:FULL-STMT) (:INCLUDES)
    (:OPCODE) (:SYN-CTX . "GENERIC")
   )
   "\"data\"")
  "\" = \""
  (((:CLASS . "UNARYOPERATOR") (:COUNTER . 7) (:FULL-STMT) (:INCLUDES)
    (:OPCODE . "-") (:SYN-CTX . "GENERIC")
   )
   "\"-\""
   (((:CLASS . "INTEGERLITERAL") (:COUNTER . 8) (:FULL-STMT) (:INCLUDES)
     (:OPCODE) (:SYN-CTX . "GENERIC")
    )
    "\"1\"")
   "\"\"")
  "\"\"") . T))
    :free-variables '(("data" "int" :-CONST :-REGISTER))
    :includes '("<stdlib.h>")
    :types '((CLANG-TYPE
                :HASH -760642589583846522
                :POINTER NIL
                :NAME "unsigned int"
                :SIZE 4)
             (CLANG-TYPE
                :HASH -1958391046879680490
                :POINTER NIL
                :NAME "int"
                :SIZE 4))
    :macros '((CLANG-MACRO :HASH 2308996158549424241 :NAME "URAND31"
                           :BODY "URAND31() (((unsigned)rand()<<30) ^ ((unsigned)rand()<<15) ^ rand())")
              (CLANG-MACRO :HASH 1124813122759813294 :NAME "RAND32"
                           :BODY "RAND32() ((int)(rand() & 1 ? URAND31() : -URAND31() - 1))"))
    :code "data = -1;
    data = RAND32();
    printIntLine(100 / data);"))
\end{lstlisting}
\end{itemize}
\end{description}

\subsection*{Bug Template {\tt CWE377\_INSECURE\_TEMPORARY\_FILE\_\_CHAR\_TEMPNAM\_01\_BAD\_INLINE}}
\begin{description}
\item[Definition:]~\newline
\begin{lstlisting}[language=lisp]
(define-scion CWE377_Insecure_Temporary_File__char_tempnam_01_bad_inline
  (make-instance 'clang-scion
    :name 'CWE377_Insecure_Temporary_File__char_tempnam_01_bad_inline
    :patches (list printLine_patch CWE377_Insecure_Temporary_File__char_tempnam_01_bad_inline_patch)))
\end{lstlisting}
\item[Patches:]~
\begin{itemize}
\item Definition for patch {\tt PRINTLINE\_PATCH}.
\begin{lstlisting}[language=lisp]
(defvar printLine_patch
  (make-instance 'clang-static-patch
    :precondition (lambda (obj location)
  (and (= location 0)
       (not (member "printLine" (asts obj)
                    :test #'string=
                    :key [#'first #'ast-declares]))))
    :free-variables 'NIL
    :includes '("<stddef.h>" "<stdio.h>")
    :types '((CLANG-TYPE
                :HASH 3615142211888308905
                :POINTER T
                :NAME "void"
                :SIZE 8)
             (CLANG-TYPE
                :HASH -1944158543856436560
                :POINTER T
                :CONST T
                :NAME "char"
                :SIZE 8))
    :macros 'NIL
    :code "void printLine (const char * line)
{
    if(line != NULL) {
        printf(\"%s\\n\", line);
    }
}"))
\end{lstlisting}
\item Definition for patch {\tt CWE377\_INSECURE\_TEMPORARY\_FILE\_\_CHAR\_TEMPNAM\_01\_BAD\_INLINE\_PATCH}.
\begin{lstlisting}[language=lisp]
(defvar CWE377_Insecure_Temporary_File__char_tempnam_01_bad_inline_patch
  (make-instance 'clang-dynamic-patch
    :precondition NIL
    :cwe 377
    :conditional-code '()
    :free-variables '(("filename" "*char" :-CONST :-REGISTER) ("fileDesc" "int" :-CONST :-REGISTER))
    :includes '("<fcntl.h>" "<stddef.h>" "<stdio.h>" "<stdlib.h>" "<sys/stat.h>" "<unistd.h>")
    :types '((CLANG-TYPE
                :HASH 3615142211888308905
                :POINTER T
                :NAME "void"
                :SIZE 8)
             (CLANG-TYPE
                :HASH -1958391046879680490
                :POINTER NIL
                :NAME "int"
                :SIZE 4)
             (CLANG-TYPE
                :HASH 5790451697626571727
                :POINTER T
                :NAME "char"
                :SIZE 8))
    :macros '((CLANG-MACRO :HASH -7379358396012845812 :NAME "CLOSE" :BODY "CLOSE close")
              (CLANG-MACRO :HASH 1558538643793173296 :NAME "OPEN" :BODY "OPEN open")
              (CLANG-MACRO :HASH 7044633915514794449 :NAME "TEMPNAM" :BODY "TEMPNAM tempnam")
              (CLANG-MACRO :HASH -1506273811393726077 :NAME "MKSTEMP" :BODY "MKSTEMP mkstemp"))
    :code "{
        
        
        filename = TEMPNAM(NULL, NULL);
        if (filename == NULL) {
            exit(1);
        }
        printLine(filename);
        /* FLAW: Open a temporary file using open() and flags that do not prevent a race condition */
        fileDesc = OPEN(filename, O_RDWR|O_CREAT, S_IREAD|S_IWRITE);
        if (fileDesc != -1) {
            printLine(\"Temporary file was opened...now closing file\");
            CLOSE(fileDesc);
        }
        free(filename);
    }"))
\end{lstlisting}
\end{itemize}
\end{description}

\subsection*{Bug Template {\tt CWE398\_POOR\_CODE\_QUALITY\_\_ADDITION\_01\_BAD\_INLINE}}
\begin{description}
\item[Definition:]~\newline
\begin{lstlisting}[language=lisp]
(define-scion CWE398_Poor_Code_Quality__addition_01_bad_inline
  (make-instance 'clang-scion
    :name 'CWE398_Poor_Code_Quality__addition_01_bad_inline
    :patches (list printIntLine_patch CWE398_Poor_Code_Quality__addition_01_bad_inline_patch)))
\end{lstlisting}
\item[Patches:]~
\begin{itemize}
\item Definition for patch {\tt PRINTINTLINE\_PATCH}.
\begin{lstlisting}[language=lisp]
(defvar printIntLine_patch
  (make-instance 'clang-static-patch
    :precondition (lambda (obj location)
  (and (= location 0)
       (not (member "printIntLine" (asts obj)
                    :test #'string=
                    :key [#'first #'ast-declares]))))
    :free-variables 'NIL
    :includes '("<stdio.h>")
    :types '((CLANG-TYPE
                :HASH -1958391046879680490
                :POINTER NIL
                :NAME "int"
                :SIZE 4))
    :macros 'NIL
    :code "void printIntLine (int intNumber)
{
    printf(\"%d\\n\", intNumber);
}"))
\end{lstlisting}
\item Definition for patch {\tt CWE398\_POOR\_CODE\_QUALITY\_\_ADDITION\_01\_BAD\_INLINE\_PATCH}.
\begin{lstlisting}[language=lisp]
(defvar CWE398_Poor_Code_Quality__addition_01_bad_inline_patch
  (make-instance 'clang-dynamic-patch
    :precondition NIL
    :cwe 398
    :conditional-code '()
    :free-variables '(("intOne" "int" :-CONST :-REGISTER)
                      ("intTwo" "int" :-CONST :-REGISTER)
                      ("intSum" "int" :-CONST :-REGISTER))
    :includes 'NIL
    :types '((CLANG-TYPE
                :HASH -1958391046879680490
                :POINTER NIL
                :NAME "int"
                :SIZE 4))
    :macros 'NIL
    :code "{
        intOne = 1;
        printIntLine(intSum);
        /* FLAW: the statement has no effect */
        intOne + intTwo; /* This generates a compiler warning, but we expect it to */
        printIntLine(intSum);
    }"))
\end{lstlisting}
\end{itemize}
\end{description}

\subsection*{Bug Template {\tt CWE400\_RESOURCE\_EXHAUSTION\_\_RAND\_FOR\_LOOP\_01\_BAD\_INLINE}}
\begin{description}
\item[Definition:]~\newline
\begin{lstlisting}[language=lisp]
(define-scion CWE400_Resource_Exhaustion__rand_for_loop_01_bad_inline
  (make-instance 'clang-scion
    :name 'CWE400_Resource_Exhaustion__rand_for_loop_01_bad_inline
    :patches (list printLine_patch CWE400_Resource_Exhaustion__rand_for_loop_01_bad_inline_patch)))
\end{lstlisting}
\item[Patches:]~
\begin{itemize}
\item Definition for patch {\tt PRINTLINE\_PATCH}.
\begin{lstlisting}[language=lisp]
(defvar printLine_patch
  (make-instance 'clang-static-patch
    :precondition (lambda (obj location)
  (and (= location 0)
       (not (member "printLine" (asts obj)
                    :test #'string=
                    :key [#'first #'ast-declares]))))
    :free-variables 'NIL
    :includes '("<stddef.h>" "<stdio.h>")
    :types '((CLANG-TYPE
                :HASH 3615142211888308905
                :POINTER T
                :NAME "void"
                :SIZE 8)
             (CLANG-TYPE
                :HASH -1944158543856436560
                :POINTER T
                :CONST T
                :NAME "char"
                :SIZE 8))
    :macros 'NIL
    :code "void printLine (const char * line)
{
    if(line != NULL) {
        printf(\"%s\\n\", line);
    }
}"))
\end{lstlisting}
\item Definition for patch {\tt CWE400\_RESOURCE\_EXHAUSTION\_\_RAND\_FOR\_LOOP\_01\_BAD\_INLINE\_PATCH}.
\begin{lstlisting}[language=lisp]
(defvar CWE400_Resource_Exhaustion__rand_for_loop_01_bad_inline_patch
  (make-instance 'clang-dynamic-patch
    :precondition NIL
    :cwe 400
    :conditional-code '(((((:CLASS . "BINARYOPERATOR") (:COUNTER . 5) (:FULL-STMT . T) (:INCLUDES)
   (:OPCODE . "=") (:SYN-CTX . "FULLSTMT")
  )
  "\"\""
  (((:CLASS . "DECLREFEXPR") (:COUNTER . 6) (:FULL-STMT) (:INCLUDES)
    (:OPCODE) (:SYN-CTX . "GENERIC")
   )
   "\"count\"")
  "\" = \""
  (((:CLASS . "UNARYOPERATOR") (:COUNTER . 7) (:FULL-STMT) (:INCLUDES)
    (:OPCODE . "-") (:SYN-CTX . "GENERIC")
   )
   "\"-\""
   (((:CLASS . "INTEGERLITERAL") (:COUNTER . 8) (:FULL-STMT) (:INCLUDES)
     (:OPCODE) (:SYN-CTX . "GENERIC")
    )
    "\"1\"")
   "\"\"")
  "\"\"") . T))
    :free-variables '(("count" "int" :-CONST :-REGISTER) ("i" "size_t" :-CONST :-REGISTER))
    :includes '("<stdlib.h>")
    :types '((CLANG-TYPE
                :COL 1
                :DECL NIL
                :FILE "/usr/bin/../lib/clang/6.0.1/include/stddef.h"
                :LINE 62
                :HASH 764611252874068922
                :I-FILE "<stddef.h>"
                :POINTER NIL
                :NAME "size_t"
                :SIZE 8)
             (CLANG-TYPE
                :HASH -760642589583846522
                :POINTER NIL
                :NAME "unsigned int"
                :SIZE 4)
             (CLANG-TYPE
                :HASH -1958391046879680490
                :POINTER NIL
                :NAME "int"
                :SIZE 4))
    :macros '((CLANG-MACRO :HASH 2308996158549424241 :NAME "URAND31"
                           :BODY "URAND31() (((unsigned)rand()<<30) ^ ((unsigned)rand()<<15) ^ rand())")
              (CLANG-MACRO :HASH 1124813122759813294 :NAME "RAND32"
                           :BODY "RAND32() ((int)(rand() & 1 ? URAND31() : -URAND31() - 1))"))
    :code "count = -1;
    count = RAND32();
    {
        i = 0;
        /* POTENTIAL FLAW: For loop using count as the loop variant and no validation */
        for (i = 0; i < (size_t)count; i++) {
            printLine(\"Hello\");
        }
    }"))
\end{lstlisting}
\end{itemize}
\end{description}

\subsection*{Bug Template {\tt CWE401\_MEMORY\_LEAK\_\_INT\_MALLOC\_01\_BAD\_INLINE}}
\begin{description}
\item[Definition:]~\newline
\begin{lstlisting}[language=lisp]
(define-scion CWE401_Memory_Leak__int_malloc_01_bad_inline
  (make-instance 'clang-scion
    :name 'CWE401_Memory_Leak__int_malloc_01_bad_inline
    :patches (list printIntLine_patch CWE401_Memory_Leak__int_malloc_01_bad_inline_patch)))
\end{lstlisting}
\item[Patches:]~
\begin{itemize}
\item Definition for patch {\tt PRINTINTLINE\_PATCH}.
\begin{lstlisting}[language=lisp]
(defvar printIntLine_patch
  (make-instance 'clang-static-patch
    :precondition (lambda (obj location)
  (and (= location 0)
       (not (member "printIntLine" (asts obj)
                    :test #'string=
                    :key [#'first #'ast-declares]))))
    :free-variables 'NIL
    :includes '("<stdio.h>")
    :types '((CLANG-TYPE
                :HASH -1958391046879680490
                :POINTER NIL
                :NAME "int"
                :SIZE 4))
    :macros 'NIL
    :code "void printIntLine (int intNumber)
{
    printf(\"%d\\n\", intNumber);
}"))
\end{lstlisting}
\item Definition for patch {\tt CWE401\_MEMORY\_LEAK\_\_INT\_MALLOC\_01\_BAD\_INLINE\_PATCH}.
\begin{lstlisting}[language=lisp]
(defvar CWE401_Memory_Leak__int_malloc_01_bad_inline_patch
  (make-instance 'clang-dynamic-patch
    :precondition NIL
    :cwe 401
    :conditional-code '(((((:CLASS . "BINARYOPERATOR") (:COUNTER . 5) (:FULL-STMT . T)
   (:INCLUDES "<stddef.h>") (:OPCODE . "=") (:SYN-CTX . "FULLSTMT")
  )
  "\"\""
  (((:CLASS . "DECLREFEXPR") (:COUNTER . 6) (:FULL-STMT) (:INCLUDES)
    (:OPCODE) (:SYN-CTX . "GENERIC")
   )
   "\"data\"")
  "\" = \""
  (((:CLASS . "MACROEXPANSION") (:COUNTER . 7) (:FULL-STMT) (:IN-MACRO-EXPANSION . T)
    (:INCLUDES "<stddef.h>") (:OPCODE) (:SYN-CTX . "GENERIC") (:TYPES 3615142211888308905)
   )
   "\"NULL\"")
  "\"\"") . T))
    :free-variables '(("data" "*int" :-CONST :-REGISTER))
    :includes '("<stddef.h>" "<stdlib.h>")
    :types '((CLANG-TYPE
                :HASH 3615142211888308905
                :POINTER T
                :NAME "void"
                :SIZE 8)
             (CLANG-TYPE
                :HASH -1958391046879680490
                :POINTER NIL
                :NAME "int"
                :SIZE 4)
             (CLANG-TYPE
                :HASH -2241398076656181049
                :POINTER T
                :NAME "int"
                :SIZE 8))
    :macros 'NIL
    :code "data = NULL;
    data = (int *)malloc(100*sizeof(int));
    if (data == NULL) {
        exit(-1);
    }data[0] = 5printIntLine(data[0]);"))
\end{lstlisting}
\end{itemize}
\end{description}

\subsection*{Bug Template {\tt CWE404\_IMPROPER\_RESOURCE\_SHUTDOWN\_\_OPEN\_FCLOSE\_01\_BAD\_INLINE}}
\begin{description}
\item[Definition:]~\newline
\begin{lstlisting}[language=lisp]
(define-scion CWE404_Improper_Resource_Shutdown__open_fclose_01_bad_inline
  (make-instance 'clang-scion
    :name 'CWE404_Improper_Resource_Shutdown__open_fclose_01_bad_inline
    :patches (list CWE404_Improper_Resource_Shutdown__open_fclose_01_bad_inline_patch)))
\end{lstlisting}
\item[Patches:]~
\begin{itemize}
\item Definition for patch {\tt CWE404\_IMPROPER\_RESOURCE\_SHUTDOWN\_\_OPEN\_FCLOSE\_01\_BAD\_INLINE\_PATCH}.
\begin{lstlisting}[language=lisp]
(defvar CWE404_Improper_Resource_Shutdown__open_fclose_01_bad_inline_patch
  (make-instance 'clang-dynamic-patch
    :precondition NIL
    :cwe 404
    :conditional-code '(((((:CLASS . "BINARYOPERATOR") (:COUNTER . 5) (:FULL-STMT . T) (:INCLUDES)
   (:OPCODE . "=") (:SYN-CTX . "FULLSTMT")
  )
  "\"\""
  (((:CLASS . "DECLREFEXPR") (:COUNTER . 6) (:FULL-STMT) (:INCLUDES)
    (:OPCODE) (:SYN-CTX . "GENERIC")
   )
   "\"data\"")
  "\" = \""
  (((:CLASS . "UNARYOPERATOR") (:COUNTER . 7) (:FULL-STMT) (:INCLUDES)
    (:OPCODE . "-") (:SYN-CTX . "GENERIC")
   )
   "\"-\""
   (((:CLASS . "INTEGERLITERAL") (:COUNTER . 8) (:FULL-STMT) (:INCLUDES)
     (:OPCODE) (:SYN-CTX . "GENERIC")
    )
    "\"1\"")
   "\"\"")
  "\"\"") . T))
    :free-variables '(("data" "int" :-CONST :-REGISTER))
    :includes '("<fcntl.h>" "<stdio.h>" "<sys/stat.h>")
    :types '((CLANG-TYPE
                :COL 1
                :DECL NIL
                :FILE "/usr/include/bits/types/FILE.h"
                :LINE 7
                :HASH 3647496794580001440
                :I-FILE "<stdio.h>"
                :POINTER T
                :NAME "FILE"
                :SIZE 8)
             (CLANG-TYPE
                :HASH -1958391046879680490
                :POINTER NIL
                :NAME "int"
                :SIZE 4))
    :macros '((CLANG-MACRO :HASH 1558538643793173296 :NAME "OPEN" :BODY "OPEN open")
              (CLANG-MACRO :HASH -7379358396012845812 :NAME "CLOSE" :BODY "CLOSE close"))
    :code "data = -1;
    data = OPEN(\"BadSource_open.txt\", O_RDWR|O_CREAT, S_IREAD|S_IWRITE);
    if (data != -1) {
        /* FLAW: Attempt to close the file using fclose() instead of close() */
        fclose((FILE *)data);
    }"))
\end{lstlisting}
\end{itemize}
\end{description}

\subsection*{Bug Template {\tt CWE415\_DOUBLE\_FREE\_\_MALLOC\_FREE\_INT\_31\_BAD\_INLINE}}
\begin{description}
\item[Definition:]~\newline
\begin{lstlisting}[language=lisp]
(define-scion CWE415_Double_Free__malloc_free_int_31_bad_inline
  (make-instance 'clang-scion
    :name 'CWE415_Double_Free__malloc_free_int_31_bad_inline
    :patches (list CWE415_Double_Free__malloc_free_int_31_bad_inline_patch)))
\end{lstlisting}
\item[Patches:]~
\begin{itemize}
\item Definition for patch {\tt CWE415\_DOUBLE\_FREE\_\_MALLOC\_FREE\_INT\_31\_BAD\_INLINE\_PATCH}.
\begin{lstlisting}[language=lisp]
(defvar CWE415_Double_Free__malloc_free_int_31_bad_inline_patch
  (make-instance 'clang-dynamic-patch
    :precondition NIL
    :cwe 415
    :conditional-code '(((((:CLASS . "BINARYOPERATOR") (:COUNTER . 5) (:FULL-STMT . T)
   (:INCLUDES "<stddef.h>") (:OPCODE . "=") (:SYN-CTX . "FULLSTMT")
  )
  "\"\""
  (((:CLASS . "DECLREFEXPR") (:COUNTER . 6) (:FULL-STMT) (:INCLUDES)
    (:OPCODE) (:SYN-CTX . "GENERIC")
   )
   "\"data\"")
  "\" = \""
  (((:CLASS . "MACROEXPANSION") (:COUNTER . 7) (:FULL-STMT) (:IN-MACRO-EXPANSION . T)
    (:INCLUDES "<stddef.h>") (:OPCODE) (:SYN-CTX . "GENERIC") (:TYPES 3615142211888308905)
   )
   "\"NULL\"")
  "\"\"") . T))
    :free-variables '(("data" "*int" :-CONST :-REGISTER) ("dataCopy" "*int" :-CONST :-REGISTER))
    :includes '("<stddef.h>" "<stdlib.h>")
    :types '((CLANG-TYPE
                :HASH -2241398076656181049
                :POINTER T
                :NAME "int"
                :SIZE 8)
             (CLANG-TYPE
                :HASH 3615142211888308905
                :POINTER T
                :NAME "void"
                :SIZE 8)
             (CLANG-TYPE
                :HASH -1958391046879680490
                :POINTER NIL
                :NAME "int"
                :SIZE 4))
    :macros 'NIL
    :code "data = NULL;
    data = (int *)malloc(100*sizeof(int));
    if (data == NULL) {
        exit(-1);
    }free(data){
        dataCopy = data;
        data = dataCopy;
        /* POTENTIAL FLAW: Possibly freeing memory twice */
        free(data);
    }"))
\end{lstlisting}
\end{itemize}
\end{description}

\subsection*{Bug Template {\tt CWE426\_UNTRUSTED\_SEARCH\_PATH\_\_CHAR\_SYSTEM\_01\_BAD\_INLINE}}
\begin{description}
\item[Definition:]~\newline
\begin{lstlisting}[language=lisp]
(define-scion CWE426_Untrusted_Search_Path__char_system_01_bad_inline
  (make-instance 'clang-scion
    :name 'CWE426_Untrusted_Search_Path__char_system_01_bad_inline
    :patches (list printLine_patch CWE426_Untrusted_Search_Path__char_system_01_bad_inline_patch)))
\end{lstlisting}
\item[Patches:]~
\begin{itemize}
\item Definition for patch {\tt PRINTLINE\_PATCH}.
\begin{lstlisting}[language=lisp]
(defvar printLine_patch
  (make-instance 'clang-static-patch
    :precondition (lambda (obj location)
  (and (= location 0)
       (not (member "printLine" (asts obj)
                    :test #'string=
                    :key [#'first #'ast-declares]))))
    :free-variables 'NIL
    :includes '("<stddef.h>" "<stdio.h>")
    :types '((CLANG-TYPE
                :HASH 3615142211888308905
                :POINTER T
                :NAME "void"
                :SIZE 8)
             (CLANG-TYPE
                :HASH -1944158543856436560
                :POINTER T
                :CONST T
                :NAME "char"
                :SIZE 8))
    :macros 'NIL
    :code "void printLine (const char * line)
{
    if(line != NULL) {
        printf(\"%s\\n\", line);
    }
}"))
\end{lstlisting}
\item Definition for patch {\tt CWE426\_UNTRUSTED\_SEARCH\_PATH\_\_CHAR\_SYSTEM\_01\_BAD\_INLINE\_PATCH}.
\begin{lstlisting}[language=lisp]
(defvar CWE426_Untrusted_Search_Path__char_system_01_bad_inline_patch
  (make-instance 'clang-dynamic-patch
    :precondition NIL
    :cwe 426
    :conditional-code '()
    :free-variables '(("data" "*char" :-CONST :-REGISTER) ("dataBuffer" "[100]char" :-CONST :-REGISTER))
    :includes '("<stdlib.h>" "<string.h>")
    :types '((CLANG-TYPE
                :ARRAY "[100]"
                :HASH 6253389274476629705
                :POINTER NIL
                :NAME "char"
                :SIZE 100)
             (CLANG-TYPE
                :HASH 5790451697626571727
                :POINTER T
                :NAME "char"
                :SIZE 8))
    :macros '((CLANG-MACRO :HASH -6429760151768931699 :NAME "SYSTEM" :BODY "SYSTEM system")
              (CLANG-MACRO :HASH 3371904807624756031 :NAME "BAD_OS_COMMAND" :BODY "BAD_OS_COMMAND \"ls -la\"")
              (CLANG-MACRO :HASH -3046674180685201017 :NAME "GOOD_OS_COMMAND" :BODY "GOOD_OS_COMMAND \"/usr/bin/ls -la\""))
    :code "dataBuffer = \"\"data = dataBufferstrcpy(data, BAD_OS_COMMAND)if (SYSTEM(data) <= 0) {
        printLine(\"command execution failed!\");
        exit(1);
    }"))
\end{lstlisting}
\end{itemize}
\end{description}

\subsection*{Bug Template {\tt CWE459\_INCOMPLETE\_CLEANUP\_\_CHAR\_01\_BAD\_INLINE}}
\begin{description}
\item[Definition:]~\newline
\begin{lstlisting}[language=lisp]
(define-scion CWE459_Incomplete_Cleanup__char_01_bad_inline
  (make-instance 'clang-scion
    :name 'CWE459_Incomplete_Cleanup__char_01_bad_inline
    :patches (list CWE459_Incomplete_Cleanup__char_01_bad_inline_patch)))
\end{lstlisting}
\item[Patches:]~
\begin{itemize}
\item Definition for patch {\tt CWE459\_INCOMPLETE\_CLEANUP\_\_CHAR\_01\_BAD\_INLINE\_PATCH}.
\begin{lstlisting}[language=lisp]
(defvar CWE459_Incomplete_Cleanup__char_01_bad_inline_patch
  (make-instance 'clang-dynamic-patch
    :precondition NIL
    :cwe 459
    :conditional-code '()
    :free-variables '(("filename" "[]char" :-CONST :-REGISTER)
                      ("pFile" "*FILE" :-CONST :-REGISTER)
                      ("fileDesc" "int" :-CONST :-REGISTER))
    :includes '("<stddef.h>" "<stdio.h>" "<stdlib.h>")
    :types '((CLANG-TYPE
                :HASH 3615142211888308905
                :POINTER T
                :NAME "void"
                :SIZE 8)
             (CLANG-TYPE
                :HASH -1958391046879680490
                :POINTER NIL
                :NAME "int"
                :SIZE 4)
             (CLANG-TYPE
                :COL 1
                :DECL NIL
                :FILE "/usr/include/bits/types/FILE.h"
                :LINE 7
                :HASH 3647496794580001440
                :I-FILE "<stdio.h>"
                :POINTER T
                :NAME "FILE"
                :SIZE 8)
             (CLANG-TYPE
                :ARRAY "[]"
                :HASH 4286207319223806414
                :POINTER NIL
                :NAME "char"
                :SIZE NIL))
    :macros '((CLANG-MACRO :HASH -3470641226466452289 :NAME "FDOPEN" :BODY "FDOPEN fdopen")
              (CLANG-MACRO :HASH -1506273811393726077 :NAME "MKSTEMP" :BODY "MKSTEMP mkstemp")
              (CLANG-MACRO :HASH 4880025556042520325 :NAME "UNLINK" :BODY "UNLINK unlink"))
    :code "{
        
        
        /* Establish that this is a temporary file and that it should be deleted */
        fileDesc = MKSTEMP(filename);
        if (fileDesc != -1) {
            pFile = FDOPEN(fileDesc, \"w\");
            if (pFile != NULL) {
                fprintf(pFile, \"Temporary file\");
                fclose(pFile);
                /* FLAW: We don't unlink */
            }
        }
    }"))
\end{lstlisting}
\end{itemize}
\end{description}

\subsection*{Bug Template {\tt CWE464\_ADDITION\_OF\_DATA\_STRUCTURE\_SENTINEL\_\_BASIC\_01\_BAD\_INLINE}}
\begin{description}
\item[Definition:]~\newline
\begin{lstlisting}[language=lisp]
(define-scion CWE464_Addition_of_Data_Structure_Sentinel__basic_01_bad_inline
  (make-instance 'clang-scion
    :name 'CWE464_Addition_of_Data_Structure_Sentinel__basic_01_bad_inline
    :patches (list printLine_patch CWE464_Addition_of_Data_Structure_Sentinel__basic_01_bad_inline_patch)))
\end{lstlisting}
\item[Patches:]~
\begin{itemize}
\item Definition for patch {\tt PRINTLINE\_PATCH}.
\begin{lstlisting}[language=lisp]
(defvar printLine_patch
  (make-instance 'clang-static-patch
    :precondition (lambda (obj location)
  (and (= location 0)
       (not (member "printLine" (asts obj)
                    :test #'string=
                    :key [#'first #'ast-declares]))))
    :free-variables 'NIL
    :includes '("<stddef.h>" "<stdio.h>")
    :types '((CLANG-TYPE
                :HASH 3615142211888308905
                :POINTER T
                :NAME "void"
                :SIZE 8)
             (CLANG-TYPE
                :HASH -1944158543856436560
                :POINTER T
                :CONST T
                :NAME "char"
                :SIZE 8))
    :macros 'NIL
    :code "void printLine (const char * line)
{
    if(line != NULL) {
        printf(\"%s\\n\", line);
    }
}"))
\end{lstlisting}
\item Definition for patch {\tt CWE464\_ADDITION\_OF\_DATA\_STRUCTURE\_SENTINEL\_\_BASIC\_01\_BAD\_INLINE\_PATCH}.
\begin{lstlisting}[language=lisp]
(defvar CWE464_Addition_of_Data_Structure_Sentinel__basic_01_bad_inline_patch
  (make-instance 'clang-dynamic-patch
    :precondition NIL
    :cwe 464
    :conditional-code '()
    :free-variables '(("data" "char" :-CONST :-REGISTER)
                      ("charArraySource" "[2]char" :-CONST :-REGISTER)
                      ("charArraySink" "[4]char" :-CONST :-REGISTER))
    :includes '("<stdio.h>" "<stdlib.h>")
    :types '((CLANG-TYPE
                :ARRAY "[4]"
                :HASH -5892687046710376854
                :POINTER NIL
                :NAME "char"
                :SIZE 4)
             (CLANG-TYPE
                :HASH -2054504279541534951
                :POINTER NIL
                :NAME "char"
                :SIZE 1)
             (CLANG-TYPE
                :ARRAY "[2]"
                :HASH -3317663057540178253
                :POINTER NIL
                :NAME "char"
                :SIZE 2))
    :macros 'NIL
    :code "data = ' '{
        
        charArraySource[0] = (char)getc(stdin);
        charArraySource[1] = '\\0';
        /* FLAW: If the character entered on the command line is not an int,
         * a null value will be returned */
        data = (char)atoi(charArraySource);
    }{
        
        charArraySink[0] = 'x';
        /* POTENTIAL FLAW: If data is null, the rest of the array will not be printed */
        charArraySink[1] = data;
        charArraySink[2] = 'z';
        charArraySink[3] = '\\0';
        printLine(charArraySink);
    }"))
\end{lstlisting}
\end{itemize}
\end{description}

\subsection*{Bug Template {\tt CWE467\_USE\_OF\_SIZEOF\_ON\_POINTER\_TYPE\_\_CHAR\_01\_BAD\_INLINE}}
\begin{description}
\item[Definition:]~\newline
\begin{lstlisting}[language=lisp]
(define-scion CWE467_Use_of_sizeof_on_Pointer_Type__char_01_bad_inline
  (make-instance 'clang-scion
    :name 'CWE467_Use_of_sizeof_on_Pointer_Type__char_01_bad_inline
    :patches (list printHexCharLine_patch CWE467_Use_of_sizeof_on_Pointer_Type__char_01_bad_inline_patch)))
\end{lstlisting}
\item[Patches:]~
\begin{itemize}
\item Definition for patch {\tt PRINTHEXCHARLINE\_PATCH}.
\begin{lstlisting}[language=lisp]
(defvar printHexCharLine_patch
  (make-instance 'clang-static-patch
    :precondition (lambda (obj location)
  (and (= location 0)
       (not (member "printHexCharLine" (asts obj)
                    :test #'string=
                    :key [#'first #'ast-declares]))))
    :free-variables 'NIL
    :includes '("<stdio.h>")
    :types '((CLANG-TYPE
                :HASH -2054504279541534951
                :POINTER NIL
                :NAME "char"
                :SIZE 1))
    :macros 'NIL
    :code "void printHexCharLine (char charHex)
{
    printf(\"%02x\\n\", charHex);
}"))
\end{lstlisting}
\item Definition for patch {\tt CWE467\_USE\_OF\_SIZEOF\_ON\_POINTER\_TYPE\_\_CHAR\_01\_BAD\_INLINE\_PATCH}.
\begin{lstlisting}[language=lisp]
(defvar CWE467_Use_of_sizeof_on_Pointer_Type__char_01_bad_inline_patch
  (make-instance 'clang-dynamic-patch
    :precondition NIL
    :cwe 467
    :conditional-code '(((((:CLASS . "BINARYOPERATOR") (:COUNTER) (:FULL-STMT . T)
   (:INCLUDES "<stddef.h>") (:OPCODE . "=") (:SYN-CTX . "FULLSTMT") (:TYPES 3615142211888308905)
  )
  (((:CLASS . "IMPLICITCASTEXPR") (:COUNTER) (:EXPR-TYPE . 5790451697626571727) (:FULL-STMT)
    (:INCLUDES) (:OPCODE) (:SYN-CTX . "GENERIC")
   )
   (((:CLASS . "DECLREFEXPR") (:COUNTER) (:EXPR-TYPE . 5790451697626571727) (:FULL-STMT)
     (:INCLUDES) (:OPCODE) (:SYN-CTX . "GENERIC")
    )
    "\"badChar\""))
  "\" = \""
  (((:CLASS . "MACROEXPANSION") (:COUNTER . 6) (:FULL-STMT) (:IN-MACRO-EXPANSION . T)
    (:INCLUDES "<stddef.h>") (:OPCODE) (:SYN-CTX . "GENERIC") (:TYPES 3615142211888308905)
   )
   "\"NULL\"")) . T))
    :free-variables '(("badChar" "*char" :-CONST :-REGISTER))
    :includes '("<stddef.h>" "<stdlib.h>")
    :types '((CLANG-TYPE
                :HASH 3615142211888308905
                :POINTER T
                :NAME "void"
                :SIZE 8)
             (CLANG-TYPE
                :HASH 5790451697626571727
                :POINTER T
                :NAME "char"
                :SIZE 8))
    :macros 'NIL
    :code "{
        badChar = NULL;
        /* FLAW: Using sizeof the pointer and not the data type in malloc() */
        badChar = (char *)malloc(sizeof(badChar));
        if (badChar == NULL) {
            exit(-1);
        }
        *badChar = 'B';
        printHexCharLine(*badChar);
        free(badChar);
    }"))
\end{lstlisting}
\end{itemize}
\end{description}

\subsection*{Bug Template {\tt CWE475\_UNDEFINED\_BEHAVIOR\_FOR\_INPUT\_TO\_API\_\_CHAR\_01\_BAD\_INLINE}}
\begin{description}
\item[Definition:]~\newline
\begin{lstlisting}[language=lisp]
(define-scion CWE475_Undefined_Behavior_for_Input_to_API__char_01_bad_inline
  (make-instance 'clang-scion
    :name 'CWE475_Undefined_Behavior_for_Input_to_API__char_01_bad_inline
    :patches (list printLine_patch CWE475_Undefined_Behavior_for_Input_to_API__char_01_bad_inline_patch)))
\end{lstlisting}
\item[Patches:]~
\begin{itemize}
\item Definition for patch {\tt PRINTLINE\_PATCH}.
\begin{lstlisting}[language=lisp]
(defvar printLine_patch
  (make-instance 'clang-static-patch
    :precondition (lambda (obj location)
  (and (= location 0)
       (not (member "printLine" (asts obj)
                    :test #'string=
                    :key [#'first #'ast-declares]))))
    :free-variables 'NIL
    :includes '("<stddef.h>" "<stdio.h>")
    :types '((CLANG-TYPE
                :HASH 3615142211888308905
                :POINTER T
                :NAME "void"
                :SIZE 8)
             (CLANG-TYPE
                :HASH -1944158543856436560
                :POINTER T
                :CONST T
                :NAME "char"
                :SIZE 8))
    :macros 'NIL
    :code "void printLine (const char * line)
{
    if(line != NULL) {
        printf(\"%s\\n\", line);
    }
}"))
\end{lstlisting}
\item Definition for patch {\tt CWE475\_UNDEFINED\_BEHAVIOR\_FOR\_INPUT\_TO\_API\_\_CHAR\_01\_BAD\_INLINE\_PATCH}.
\begin{lstlisting}[language=lisp]
(defvar CWE475_Undefined_Behavior_for_Input_to_API__char_01_bad_inline_patch
  (make-instance 'clang-dynamic-patch
    :precondition NIL
    :cwe 475
    :conditional-code '()
    :free-variables '(("dataBuffer" "[100]char" :-CONST :-REGISTER) ("data" "*char" :-CONST :-REGISTER))
    :includes '("<string.h>")
    :types '((CLANG-TYPE
                :HASH -2054504279541534951
                :POINTER NIL
                :NAME "char"
                :SIZE 1)
             (CLANG-TYPE
                :HASH 5790451697626571727
                :POINTER T
                :NAME "char"
                :SIZE 8)
             (CLANG-TYPE
                :ARRAY "[100]"
                :HASH 6253389274476629705
                :POINTER NIL
                :NAME "char"
                :SIZE 100))
    :macros 'NIL
    :code "{
        dataBuffer = \"\";
        data = dataBuffer;
        strcpy(data, \"abcdefghijklmnopqrstuvwxyz\");
        /* FLAW: Copy overlapping memory regions using memcpy() for which the result is undefined */
        memcpy(data + 6, data + 4, 10*sizeof(char));
        printLine(data);
    }"))
\end{lstlisting}
\end{itemize}
\end{description}

\subsection*{Bug Template {\tt CWE476\_NULL\_POINTER\_DEREFERENCE\_\_INT\_31\_BAD\_INLINE}}
\begin{description}
\item[Definition:]~\newline
\begin{lstlisting}[language=lisp]
(define-scion CWE476_NULL_Pointer_Dereference__int_31_bad_inline
  (make-instance 'clang-scion
    :name 'CWE476_NULL_Pointer_Dereference__int_31_bad_inline
    :patches (list printIntLine_patch CWE476_NULL_Pointer_Dereference__int_31_bad_inline_patch)))
\end{lstlisting}
\item[Patches:]~
\begin{itemize}
\item Definition for patch {\tt PRINTINTLINE\_PATCH}.
\begin{lstlisting}[language=lisp]
(defvar printIntLine_patch
  (make-instance 'clang-static-patch
    :precondition (lambda (obj location)
  (and (= location 0)
       (not (member "printIntLine" (asts obj)
                    :test #'string=
                    :key [#'first #'ast-declares]))))
    :free-variables 'NIL
    :includes '("<stdio.h>")
    :types '((CLANG-TYPE
                :HASH -1958391046879680490
                :POINTER NIL
                :NAME "int"
                :SIZE 4))
    :macros 'NIL
    :code "void printIntLine (int intNumber)
{
    printf(\"%d\\n\", intNumber);
}"))
\end{lstlisting}
\item Definition for patch {\tt CWE476\_NULL\_POINTER\_DEREFERENCE\_\_INT\_31\_BAD\_INLINE\_PATCH}.
\begin{lstlisting}[language=lisp]
(defvar CWE476_NULL_Pointer_Dereference__int_31_bad_inline_patch
  (make-instance 'clang-dynamic-patch
    :precondition NIL
    :cwe 476
    :conditional-code '()
    :free-variables '(("data" "*int" :-CONST :-REGISTER) ("dataCopy" "*int" :-CONST :-REGISTER))
    :includes '("<stddef.h>")
    :types '((CLANG-TYPE
                :HASH -2241398076656181049
                :POINTER T
                :NAME "int"
                :SIZE 8)
             (CLANG-TYPE
                :HASH 3615142211888308905
                :POINTER T
                :NAME "void"
                :SIZE 8))
    :macros 'NIL
    :code "data = NULL{
        dataCopy = data;
        data = dataCopy;
        /* POTENTIAL FLAW: Attempt to use data, which may be NULL */
        printIntLine(*data);
    }"))
\end{lstlisting}
\end{itemize}
\end{description}

\subsection*{Bug Template {\tt CWE478\_MISSING\_DEFAULT\_CASE\_IN\_SWITCH\_\_BASIC\_01\_BAD\_INLINE}}
\begin{description}
\item[Definition:]~\newline
\begin{lstlisting}[language=lisp]
(define-scion CWE478_Missing_Default_Case_in_Switch__basic_01_bad_inline
  (make-instance 'clang-scion
    :name 'CWE478_Missing_Default_Case_in_Switch__basic_01_bad_inline
    :patches (list printLine_patch CWE478_Missing_Default_Case_in_Switch__basic_01_bad_inline_patch)))
\end{lstlisting}
\item[Patches:]~
\begin{itemize}
\item Definition for patch {\tt PRINTLINE\_PATCH}.
\begin{lstlisting}[language=lisp]
(defvar printLine_patch
  (make-instance 'clang-static-patch
    :precondition (lambda (obj location)
  (and (= location 0)
       (not (member "printLine" (asts obj)
                    :test #'string=
                    :key [#'first #'ast-declares]))))
    :free-variables 'NIL
    :includes '("<stddef.h>" "<stdio.h>")
    :types '((CLANG-TYPE
                :HASH 3615142211888308905
                :POINTER T
                :NAME "void"
                :SIZE 8)
             (CLANG-TYPE
                :HASH -1944158543856436560
                :POINTER T
                :CONST T
                :NAME "char"
                :SIZE 8))
    :macros 'NIL
    :code "void printLine (const char * line)
{
    if(line != NULL) {
        printf(\"%s\\n\", line);
    }
}"))
\end{lstlisting}
\item Definition for patch {\tt CWE478\_MISSING\_DEFAULT\_CASE\_IN\_SWITCH\_\_BASIC\_01\_BAD\_INLINE\_PATCH}.
\begin{lstlisting}[language=lisp]
(defvar CWE478_Missing_Default_Case_in_Switch__basic_01_bad_inline_patch
  (make-instance 'clang-dynamic-patch
    :precondition NIL
    :cwe 478
    :conditional-code '()
    :free-variables '(("charString" "*char" :+CONST :-REGISTER) ("x" "int" :-CONST :-REGISTER))
    :includes '("<stdlib.h>")
    :types '((CLANG-TYPE
                :HASH -1958391046879680490
                :POINTER NIL
                :NAME "int"
                :SIZE 4)
             (CLANG-TYPE
                :HASH -1944158543856436560
                :POINTER T
                :CONST T
                :NAME "char"
                :SIZE 8))
    :macros 'NIL
    :code "{
        charString = \"shouldn\\'t see this value\";
        
        x = (rand() % 3);
        switch (x) {
        case 0:
            charString = \"0\";
            break;
        case 1:
            charString = \"1\";
            break;
            /* FLAW: x could be 2, and there is no 'default' case for that */
        }
        printLine(charString);
    }"))
\end{lstlisting}
\end{itemize}
\end{description}

\subsection*{Bug Template {\tt CWE479\_SIGNAL\_HANDLER\_USE\_OF\_NON\_REENTRANT\_FUNCTION\_\_BASIC\_01\_BAD\_INLINE}}
\begin{description}
\item[Definition:]~\newline
\begin{lstlisting}[language=lisp]
(define-scion CWE479_Signal_Handler_Use_of_Non_Reentrant_Function__basic_01_bad_inline
  (make-instance 'clang-scion
    :name 'CWE479_Signal_Handler_Use_of_Non_Reentrant_Function__basic_01_bad_inline
    :patches (list CWE479_Signal_Handler_Use_of_Non_Reentrant_Function__basic_01_bad_inline_patch)))
\end{lstlisting}
\item[Patches:]~
\begin{itemize}
\item Definition for patch\newline{\tt CWE479\_SIGNAL\_HANDLER\_USE\_OF\_NON\_REENTRANT\_FUNCTION\_\_BASIC\_01\_BAD\_INLINE\_PATCH}.
\begin{lstlisting}[language=lisp]
(defvar CWE479_Signal_Handler_Use_of_Non_Reentrant_Function__basic_01_bad_inline_patch
  (make-instance 'clang-dynamic-patch
    :precondition NIL
    :cwe 479
    :conditional-code '()
    :free-variables 'NIL
    :includes '("<signal.h>")
    :types 'NIL
    :macros 'NIL
    :code "signal(SIGINT, helperBad)"))
\end{lstlisting}
\end{itemize}
\end{description}

\subsection*{Bug Template {\tt CWE481\_ASSIGNING\_INSTEAD\_OF\_COMPARING\_\_BASIC\_01\_BAD\_INLINE}}
\begin{description}
\item[Definition:]~\newline
\begin{lstlisting}[language=lisp]
(define-scion CWE481_Assigning_Instead_of_Comparing__basic_01_bad_inline
  (make-instance 'clang-scion
    :name 'CWE481_Assigning_Instead_of_Comparing__basic_01_bad_inline
    :patches (list printLine_patch CWE481_Assigning_Instead_of_Comparing__basic_01_bad_inline_patch)))
\end{lstlisting}
\item[Patches:]~
\begin{itemize}
\item Definition for patch {\tt PRINTLINE\_PATCH}.
\begin{lstlisting}[language=lisp]
(defvar printLine_patch
  (make-instance 'clang-static-patch
    :precondition (lambda (obj location)
  (and (= location 0)
       (not (member "printLine" (asts obj)
                    :test #'string=
                    :key [#'first #'ast-declares]))))
    :free-variables 'NIL
    :includes '("<stddef.h>" "<stdio.h>")
    :types '((CLANG-TYPE
                :HASH 3615142211888308905
                :POINTER T
                :NAME "void"
                :SIZE 8)
             (CLANG-TYPE
                :HASH -1944158543856436560
                :POINTER T
                :CONST T
                :NAME "char"
                :SIZE 8))
    :macros 'NIL
    :code "void printLine (const char * line)
{
    if(line != NULL) {
        printf(\"%s\\n\", line);
    }
}"))
\end{lstlisting}
\item Definition for patch {\tt CWE481\_ASSIGNING\_INSTEAD\_OF\_COMPARING\_\_BASIC\_01\_BAD\_INLINE\_PATCH}.
\begin{lstlisting}[language=lisp]
(defvar CWE481_Assigning_Instead_of_Comparing__basic_01_bad_inline_patch
  (make-instance 'clang-dynamic-patch
    :precondition NIL
    :cwe 481
    :conditional-code '()
    :free-variables '(("intRand" "int" :-CONST :-REGISTER))
    :includes '("<stdlib.h>")
    :types '((CLANG-TYPE
                :HASH -1958391046879680490
                :POINTER NIL
                :NAME "int"
                :SIZE 4))
    :macros 'NIL
    :code "{
        intRand = rand();
        /* FLAW: should be == and INCIDENTIAL CWE 571 Expression Is Always True */
        if(intRand = 5) {
            printLine(\"i was 5\");
        }
    }"))
\end{lstlisting}
\end{itemize}
\end{description}

\subsection*{Bug Template {\tt CWE482\_COMPARING\_INSTEAD\_OF\_ASSIGNING\_\_BASIC\_01\_BAD\_INLINE}}
\begin{description}
\item[Definition:]~\newline
\begin{lstlisting}[language=lisp]
(define-scion CWE482_Comparing_Instead_of_Assigning__basic_01_bad_inline
  (make-instance 'clang-scion
    :name 'CWE482_Comparing_Instead_of_Assigning__basic_01_bad_inline
    :patches (list printIntLine_patch CWE482_Comparing_Instead_of_Assigning__basic_01_bad_inline_patch)))
\end{lstlisting}
\item[Patches:]~
\begin{itemize}
\item Definition for patch {\tt PRINTINTLINE\_PATCH}.
\begin{lstlisting}[language=lisp]
(defvar printIntLine_patch
  (make-instance 'clang-static-patch
    :precondition (lambda (obj location)
  (and (= location 0)
       (not (member "printIntLine" (asts obj)
                    :test #'string=
                    :key [#'first #'ast-declares]))))
    :free-variables 'NIL
    :includes '("<stdio.h>")
    :types '((CLANG-TYPE
                :HASH -1958391046879680490
                :POINTER NIL
                :NAME "int"
                :SIZE 4))
    :macros 'NIL
    :code "void printIntLine (int intNumber)
{
    printf(\"%d\\n\", intNumber);
}"))
\end{lstlisting}
\item Definition for patch {\tt CWE482\_COMPARING\_INSTEAD\_OF\_ASSIGNING\_\_BASIC\_01\_BAD\_INLINE\_PATCH}.
\begin{lstlisting}[language=lisp]
(defvar CWE482_Comparing_Instead_of_Assigning__basic_01_bad_inline_patch
  (make-instance 'clang-dynamic-patch
    :precondition NIL
    :cwe 482
    :conditional-code '()
    :free-variables '(("intBadSink" "int" :-CONST :-REGISTER))
    :includes 'NIL
    :types '((CLANG-TYPE
                :HASH -1958391046879680490
                :POINTER NIL
                :NAME "int"
                :SIZE 4))
    :macros 'NIL
    :code "{
        intBadSink = 0;
        /* Print original value to avoid any unused variable incidentals */
        printIntLine(intBadSink);
        /* FLAW: meant to assign 5 to intBadSink.  Maintenance note: may generate a compiler warning, this is intentional */
        intBadSink == 5;
        printIntLine(intBadSink);
    }"))
\end{lstlisting}
\end{itemize}
\end{description}

\subsection*{Bug Template {\tt CWE483\_INCORRECT\_BLOCK\_DELIMITATION\_\_SEMICOLON\_01\_BAD\_INLINE}}
\begin{description}
\item[Definition:]~\newline
\begin{lstlisting}[language=lisp]
(define-scion CWE483_Incorrect_Block_Delimitation__semicolon_01_bad_inline
  (make-instance 'clang-scion
    :name 'CWE483_Incorrect_Block_Delimitation__semicolon_01_bad_inline
    :patches (list printLine_patch CWE483_Incorrect_Block_Delimitation__semicolon_01_bad_inline_patch)))
\end{lstlisting}
\item[Patches:]~
\begin{itemize}
\item Definition for patch {\tt PRINTLINE\_PATCH}.
\begin{lstlisting}[language=lisp]
(defvar printLine_patch
  (make-instance 'clang-static-patch
    :precondition (lambda (obj location)
  (and (= location 0)
       (not (member "printLine" (asts obj)
                    :test #'string=
                    :key [#'first #'ast-declares]))))
    :free-variables 'NIL
    :includes '("<stddef.h>" "<stdio.h>")
    :types '((CLANG-TYPE
                :HASH 3615142211888308905
                :POINTER T
                :NAME "void"
                :SIZE 8)
             (CLANG-TYPE
                :HASH -1944158543856436560
                :POINTER T
                :CONST T
                :NAME "char"
                :SIZE 8))
    :macros 'NIL
    :code "void printLine (const char * line)
{
    if(line != NULL) {
        printf(\"%s\\n\", line);
    }
}"))
\end{lstlisting}
\item Definition for patch {\tt CWE483\_INCORRECT\_BLOCK\_DELIMITATION\_\_SEMICOLON\_01\_BAD\_INLINE\_PATCH}.
\begin{lstlisting}[language=lisp]
(defvar CWE483_Incorrect_Block_Delimitation__semicolon_01_bad_inline_patch
  (make-instance 'clang-dynamic-patch
    :precondition NIL
    :cwe 483
    :conditional-code '()
    :free-variables '(("x" "int" :-CONST :-REGISTER) ("y" "int" :-CONST :-REGISTER))
    :includes '("<stdlib.h>")
    :types '((CLANG-TYPE
                :HASH -1958391046879680490
                :POINTER NIL
                :NAME "int"
                :SIZE 4))
    :macros 'NIL
    :code "{
        x = (rand() % 3);
        y = 0;
        /* FLAW: Suspicious semicolon before the if statement brace */
        if (x == 0);
        {
            printLine(\"x == 0\");
            y = 1;
        }
        if (y) {
            printLine(\"x was 0\\n\");
        }
    }"))
\end{lstlisting}
\end{itemize}
\end{description}

\subsection*{Bug Template {\tt CWE484\_OMITTED\_BREAK\_STATEMENT\_IN\_SWITCH\_\_BASIC\_01\_BAD\_INLINE}}
\begin{description}
\item[Definition:]~\newline
\begin{lstlisting}[language=lisp]
(define-scion CWE484_Omitted_Break_Statement_in_Switch__basic_01_bad_inline
  (make-instance 'clang-scion
    :name 'CWE484_Omitted_Break_Statement_in_Switch__basic_01_bad_inline
    :patches (list printLine_patch CWE484_Omitted_Break_Statement_in_Switch__basic_01_bad_inline_patch)))
\end{lstlisting}
\item[Patches:]~
\begin{itemize}
\item Definition for patch {\tt PRINTLINE\_PATCH}.
\begin{lstlisting}[language=lisp]
(defvar printLine_patch
  (make-instance 'clang-static-patch
    :precondition (lambda (obj location)
  (and (= location 0)
       (not (member "printLine" (asts obj)
                    :test #'string=
                    :key [#'first #'ast-declares]))))
    :free-variables 'NIL
    :includes '("<stddef.h>" "<stdio.h>")
    :types '((CLANG-TYPE
                :HASH 3615142211888308905
                :POINTER T
                :NAME "void"
                :SIZE 8)
             (CLANG-TYPE
                :HASH -1944158543856436560
                :POINTER T
                :CONST T
                :NAME "char"
                :SIZE 8))
    :macros 'NIL
    :code "void printLine (const char * line)
{
    if(line != NULL) {
        printf(\"%s\\n\", line);
    }
}"))
\end{lstlisting}
\item Definition for patch {\tt CWE484\_OMITTED\_BREAK\_STATEMENT\_IN\_SWITCH\_\_BASIC\_01\_BAD\_INLINE\_PATCH}.
\begin{lstlisting}[language=lisp]
(defvar CWE484_Omitted_Break_Statement_in_Switch__basic_01_bad_inline_patch
  (make-instance 'clang-dynamic-patch
    :precondition NIL
    :cwe 484
    :conditional-code '()
    :free-variables '(("x" "int" :-CONST :-REGISTER))
    :includes '("<stdlib.h>")
    :types '((CLANG-TYPE
                :HASH -1958391046879680490
                :POINTER NIL
                :NAME "int"
                :SIZE 4))
    :macros 'NIL
    :code "{
        x = (rand() % 3);
        /* FLAW: Missing break in first case */
        switch (x) {
        case 0:
            printLine(\"0\");
        case 1:
            printLine(\"1\");
            break;
        case 2:
            printLine(\"2\");
            break;
        default:
            printLine(\"Invalid Number\");
            break;
        }
    }"))
\end{lstlisting}
\end{itemize}
\end{description}

\subsection*{Bug Template {\tt CWE511\_LOGIC\_TIME\_BOMB\_\_RAND\_01\_BAD\_INLINE}}
\begin{description}
\item[Definition:]~\newline
\begin{lstlisting}[language=lisp]
(define-scion CWE511_Logic_Time_Bomb__rand_01_bad_inline
  (make-instance 'clang-scion
    :name 'CWE511_Logic_Time_Bomb__rand_01_bad_inline
    :patches (list CWE511_Logic_Time_Bomb__rand_01_bad_inline_patch)))
\end{lstlisting}
\item[Patches:]~
\begin{itemize}
\item Definition for patch {\tt CWE511\_LOGIC\_TIME\_BOMB\_\_RAND\_01\_BAD\_INLINE\_PATCH}.
\begin{lstlisting}[language=lisp]
(defvar CWE511_Logic_Time_Bomb__rand_01_bad_inline_patch
  (make-instance 'clang-dynamic-patch
    :precondition NIL
    :cwe 511
    :conditional-code '()
    :free-variables 'NIL
    :includes '("<stddef.h>" "<stdlib.h>" "<time.h>" "<unistd.h>")
    :types '((CLANG-TYPE
                :HASH 3615142211888308905
                :POINTER T
                :NAME "void"
                :SIZE 8)
             (CLANG-TYPE
                :HASH -760642589583846522
                :POINTER NIL
                :NAME "unsigned int"
                :SIZE 4))
    :macros '((CLANG-MACRO :HASH 4880025556042520325 :NAME "UNLINK" :BODY "UNLINK unlink")
              (CLANG-MACRO :HASH -2866508520563029221 :NAME "NUM_CHECK" :BODY "NUM_CHECK 20000"))
    :code "srand((unsigned)time(NULL))if (rand() == NUM_CHECK) {
        UNLINK(\"important_file.txt\");
    }"))
\end{lstlisting}
\end{itemize}
\end{description}

\subsection*{Bug Template {\tt CWE526\_INFO\_EXPOSURE\_ENVIRONMENT\_VARIABLES\_\_BASIC\_01\_BAD\_INLINE}}
\begin{description}
\item[Definition:]~\newline
\begin{lstlisting}[language=lisp]
(define-scion CWE526_Info_Exposure_Environment_Variables__basic_01_bad_inline
  (make-instance 'clang-scion
    :name 'CWE526_Info_Exposure_Environment_Variables__basic_01_bad_inline
    :patches (list printLine_patch CWE526_Info_Exposure_Environment_Variables__basic_01_bad_inline_patch)))
\end{lstlisting}
\item[Patches:]~
\begin{itemize}
\item Definition for patch {\tt PRINTLINE\_PATCH}.
\begin{lstlisting}[language=lisp]
(defvar printLine_patch
  (make-instance 'clang-static-patch
    :precondition (lambda (obj location)
  (and (= location 0)
       (not (member "printLine" (asts obj)
                    :test #'string=
                    :key [#'first #'ast-declares]))))
    :free-variables 'NIL
    :includes '("<stddef.h>" "<stdio.h>")
    :types '((CLANG-TYPE
                :HASH 3615142211888308905
                :POINTER T
                :NAME "void"
                :SIZE 8)
             (CLANG-TYPE
                :HASH -1944158543856436560
                :POINTER T
                :CONST T
                :NAME "char"
                :SIZE 8))
    :macros 'NIL
    :code "void printLine (const char * line)
{
    if(line != NULL) {
        printf(\"%s\\n\", line);
    }
}"))
\end{lstlisting}
\item Definition for patch {\tt CWE526\_INFO\_EXPOSURE\_ENVIRONMENT\_VARIABLES\_\_BASIC\_01\_BAD\_INLINE\_PATCH}.
\begin{lstlisting}[language=lisp]
(defvar CWE526_Info_Exposure_Environment_Variables__basic_01_bad_inline_patch
  (make-instance 'clang-dynamic-patch
    :precondition NIL
    :cwe 526
    :conditional-code '()
    :free-variables 'NIL
    :includes '("<stdlib.h>")
    :types 'NIL
    :macros 'NIL
    :code "printLine(getenv(\"PATH\"))"))
\end{lstlisting}
\end{itemize}
\end{description}

\subsection*{Bug Template {\tt CWE546\_SUSPICIOUS\_COMMENT\_\_BUG\_08\_BAD\_INLINE}}
\begin{description}
\item[Definition:]~\newline
\begin{lstlisting}[language=lisp]
(define-scion CWE546_Suspicious_Comment__BUG_08_bad_inline
  (make-instance 'clang-scion
    :name 'CWE546_Suspicious_Comment__BUG_08_bad_inline
    :patches (list printLine_patch staticReturnsTrue_patch CWE546_Suspicious_Comment__BUG_08_bad_inline_patch)))
\end{lstlisting}
\item[Patches:]~
\begin{itemize}
\item Definition for patch {\tt PRINTLINE\_PATCH}.
\begin{lstlisting}[language=lisp]
(defvar printLine_patch
  (make-instance 'clang-static-patch
    :precondition (lambda (obj location)
  (and (= location 0)
       (not (member "printLine" (asts obj)
                    :test #'string=
                    :key [#'first #'ast-declares]))))
    :free-variables 'NIL
    :includes '("<stddef.h>" "<stdio.h>")
    :types '((CLANG-TYPE
                :HASH 3615142211888308905
                :POINTER T
                :NAME "void"
                :SIZE 8)
             (CLANG-TYPE
                :HASH -1944158543856436560
                :POINTER T
                :CONST T
                :NAME "char"
                :SIZE 8))
    :macros 'NIL
    :code "void printLine (const char * line)
{
    if(line != NULL) {
        printf(\"%s\\n\", line);
    }
}"))
\end{lstlisting}
\item Definition for patch {\tt STATICRETURNSTRUE\_PATCH}.
\begin{lstlisting}[language=lisp]
(defvar staticReturnsTrue_patch
  (make-instance 'clang-static-patch
    :precondition (lambda (obj location)
  (and (= location 0)
       (not (member "staticReturnsTrue" (asts obj)
                    :test #'string=
                    :key [#'first #'ast-declares]))))
    :free-variables 'NIL
    :includes 'NIL
    :types 'NIL
    :macros 'NIL
    :code "static int staticReturnsTrue()
{
    return 1;
}"))
\end{lstlisting}
\item Definition for patch {\tt CWE546\_SUSPICIOUS\_COMMENT\_\_BUG\_08\_BAD\_INLINE\_PATCH}.
\begin{lstlisting}[language=lisp]
(defvar CWE546_Suspicious_Comment__BUG_08_bad_inline_patch
  (make-instance 'clang-dynamic-patch
    :precondition NIL
    :cwe 546
    :conditional-code '()
    :free-variables 'NIL
    :includes 'NIL
    :types 'NIL
    :macros 'NIL
    :code "if(staticReturnsTrue()) {
        /* FLAW: The following comment has the letters 'BUG' in it*/
        /* BUG: This comment has the letters 'BUG' in it, which is certainly
         * suspicious, because it could indicate this code has a BUG in it.
         */
        printLine(\"Hello\");
    }"))
\end{lstlisting}
\end{itemize}
\end{description}

\subsection*{Bug Template {\tt CWE570\_EXPRESSION\_ALWAYS\_FALSE\_\_N\_LESS\_INT\_MIN\_01\_BAD\_INLINE}}
\begin{description}
\item[Definition:]~\newline
\begin{lstlisting}[language=lisp]
(define-scion CWE570_Expression_Always_False__n_less_int_min_01_bad_inline
  (make-instance 'clang-scion
    :name 'CWE570_Expression_Always_False__n_less_int_min_01_bad_inline
    :patches (list printLine_patch CWE570_Expression_Always_False__n_less_int_min_01_bad_inline_patch)))
\end{lstlisting}
\item[Patches:]~
\begin{itemize}
\item Definition for patch {\tt PRINTLINE\_PATCH}.
\begin{lstlisting}[language=lisp]
(defvar printLine_patch
  (make-instance 'clang-static-patch
    :precondition (lambda (obj location)
  (and (= location 0)
       (not (member "printLine" (asts obj)
                    :test #'string=
                    :key [#'first #'ast-declares]))))
    :free-variables 'NIL
    :includes '("<stddef.h>" "<stdio.h>")
    :types '((CLANG-TYPE
                :HASH 3615142211888308905
                :POINTER T
                :NAME "void"
                :SIZE 8)
             (CLANG-TYPE
                :HASH -1944158543856436560
                :POINTER T
                :CONST T
                :NAME "char"
                :SIZE 8))
    :macros 'NIL
    :code "void printLine (const char * line)
{
    if(line != NULL) {
        printf(\"%s\\n\", line);
    }
}"))
\end{lstlisting}
\item Definition for patch {\tt CWE570\_EXPRESSION\_ALWAYS\_FALSE\_\_N\_LESS\_INT\_MIN\_01\_BAD\_INLINE\_PATCH}.
\begin{lstlisting}[language=lisp]
(defvar CWE570_Expression_Always_False__n_less_int_min_01_bad_inline_patch
  (make-instance 'clang-dynamic-patch
    :precondition NIL
    :cwe 570
    :conditional-code '()
    :free-variables '(("intRand" "int" :-CONST :-REGISTER))
    :includes '("<limits.h>" "<stdlib.h>")
    :types '((CLANG-TYPE
                :HASH -1958391046879680490
                :POINTER NIL
                :NAME "int"
                :SIZE 4))
    :macros 'NIL
    :code "intRand = rand()if (intRand < INT_MIN) {
        printLine(\"Never prints\");
    }"))
\end{lstlisting}
\end{itemize}
\end{description}

\subsection*{Bug Template {\tt CWE571\_EXPRESSION\_ALWAYS\_TRUE\_\_N\_LESS\_INT\_MAX\_01\_BAD\_INLINE}}
\begin{description}
\item[Definition:]~\newline
\begin{lstlisting}[language=lisp]
(define-scion CWE571_Expression_Always_True__n_less_int_max_01_bad_inline
  (make-instance 'clang-scion
    :name 'CWE571_Expression_Always_True__n_less_int_max_01_bad_inline
    :patches (list printLine_patch CWE571_Expression_Always_True__n_less_int_max_01_bad_inline_patch)))
\end{lstlisting}
\item[Patches:]~
\begin{itemize}
\item Definition for patch {\tt PRINTLINE\_PATCH}.
\begin{lstlisting}[language=lisp]
(defvar printLine_patch
  (make-instance 'clang-static-patch
    :precondition (lambda (obj location)
  (and (= location 0)
       (not (member "printLine" (asts obj)
                    :test #'string=
                    :key [#'first #'ast-declares]))))
    :free-variables 'NIL
    :includes '("<stddef.h>" "<stdio.h>")
    :types '((CLANG-TYPE
                :HASH 3615142211888308905
                :POINTER T
                :NAME "void"
                :SIZE 8)
             (CLANG-TYPE
                :HASH -1944158543856436560
                :POINTER T
                :CONST T
                :NAME "char"
                :SIZE 8))
    :macros 'NIL
    :code "void printLine (const char * line)
{
    if(line != NULL) {
        printf(\"%s\\n\", line);
    }
}"))
\end{lstlisting}
\item Definition for patch {\tt CWE571\_EXPRESSION\_ALWAYS\_TRUE\_\_N\_LESS\_INT\_MAX\_01\_BAD\_INLINE\_PATCH}.
\begin{lstlisting}[language=lisp]
(defvar CWE571_Expression_Always_True__n_less_int_max_01_bad_inline_patch
  (make-instance 'clang-dynamic-patch
    :precondition NIL
    :cwe 571
    :conditional-code '()
    :free-variables '(("intRand" "int" :-CONST :-REGISTER))
    :includes '("<limits.h>" "<stdlib.h>")
    :types '((CLANG-TYPE
                :HASH -1958391046879680490
                :POINTER NIL
                :NAME "int"
                :SIZE 4))
    :macros 'NIL
    :code "intRand = rand()if (intRand <= INT_MAX) {
        printLine(\"Always prints\");
    }"))
\end{lstlisting}
\end{itemize}
\end{description}

\subsection*{Bug Template {\tt CWE587\_ASSIGNMENT\_OF\_FIXED\_ADDRESS\_TO\_POINTER\_\_BASIC\_01\_BAD\_INLINE}}
\begin{description}
\item[Definition:]~\newline
\begin{lstlisting}[language=lisp]
(define-scion CWE587_Assignment_of_Fixed_Address_to_Pointer__basic_01_bad_inline
  (make-instance 'clang-scion
    :name 'CWE587_Assignment_of_Fixed_Address_to_Pointer__basic_01_bad_inline
    :patches (list printHexCharLine_patch CWE587_Assignment_of_Fixed_Address_to_Pointer__basic_01_bad_inline_patch)))
\end{lstlisting}
\item[Patches:]~
\begin{itemize}
\item Definition for patch {\tt PRINTHEXCHARLINE\_PATCH}.
\begin{lstlisting}[language=lisp]
(defvar printHexCharLine_patch
  (make-instance 'clang-static-patch
    :precondition (lambda (obj location)
  (and (= location 0)
       (not (member "printHexCharLine" (asts obj)
                    :test #'string=
                    :key [#'first #'ast-declares]))))
    :free-variables 'NIL
    :includes '("<stdio.h>")
    :types '((CLANG-TYPE
                :HASH -2054504279541534951
                :POINTER NIL
                :NAME "char"
                :SIZE 1))
    :macros 'NIL
    :code "void printHexCharLine (char charHex)
{
    printf(\"%02x\\n\", charHex);
}"))
\end{lstlisting}
\item Definition for patch {\tt CWE587\_ASSIGNMENT\_OF\_FIXED\_ADDRESS\_TO\_POINTER\_\_BASIC\_01\_BAD\_INLINE\_PATCH}.
\begin{lstlisting}[language=lisp]
(defvar CWE587_Assignment_of_Fixed_Address_to_Pointer__basic_01_bad_inline_patch
  (make-instance 'clang-dynamic-patch
    :precondition NIL
    :cwe 587
    :conditional-code '()
    :free-variables '(("charPointer" "*char" :-CONST :-REGISTER))
    :includes 'NIL
    :types '((CLANG-TYPE
                :HASH 5790451697626571727
                :POINTER T
                :NAME "char"
                :SIZE 8))
    :macros 'NIL
    :code "{
        /* FLAW: Assigning fixed address to pointer */
        charPointer = (char*)0x400000;
        printHexCharLine(*charPointer);
    }"))
\end{lstlisting}
\end{itemize}
\end{description}

\subsection*{Bug Template {\tt CWE590\_FREE\_MEMORY\_NOT\_ON\_HEAP\_\_FREE\_CHAR\_ALLOCA\_31\_BAD\_INLINE}}
\begin{description}
\item[Definition:]~\newline
\begin{lstlisting}[language=lisp]
(define-scion CWE590_Free_Memory_Not_on_Heap__free_char_alloca_31_bad_inline
  (make-instance 'clang-scion
    :name 'CWE590_Free_Memory_Not_on_Heap__free_char_alloca_31_bad_inline
    :patches (list printLine_patch CWE590_Free_Memory_Not_on_Heap__free_char_alloca_31_bad_inline_patch)))
\end{lstlisting}
\item[Patches:]~
\begin{itemize}
\item Definition for patch {\tt PRINTLINE\_PATCH}.
\begin{lstlisting}[language=lisp]
(defvar printLine_patch
  (make-instance 'clang-static-patch
    :precondition (lambda (obj location)
  (and (= location 0)
       (not (member "printLine" (asts obj)
                    :test #'string=
                    :key [#'first #'ast-declares]))))
    :free-variables 'NIL
    :includes '("<stddef.h>" "<stdio.h>")
    :types '((CLANG-TYPE
                :HASH 3615142211888308905
                :POINTER T
                :NAME "void"
                :SIZE 8)
             (CLANG-TYPE
                :HASH -1944158543856436560
                :POINTER T
                :CONST T
                :NAME "char"
                :SIZE 8))
    :macros 'NIL
    :code "void printLine (const char * line)
{
    if(line != NULL) {
        printf(\"%s\\n\", line);
    }
}"))
\end{lstlisting}
\item Definition for patch {\tt CWE590\_FREE\_MEMORY\_NOT\_ON\_HEAP\_\_FREE\_CHAR\_ALLOCA\_31\_BAD\_INLINE\_PATCH}.
\begin{lstlisting}[language=lisp]
(defvar CWE590_Free_Memory_Not_on_Heap__free_char_alloca_31_bad_inline_patch
  (make-instance 'clang-dynamic-patch
    :precondition NIL
    :cwe 590
    :conditional-code '()
    :free-variables '(("data" "*char" :-CONST :-REGISTER)
                      ("dataBuffer" "*char" :-CONST :-REGISTER)
                      ("dataCopy" "*char" :-CONST :-REGISTER))
    :includes '("<alloca.h>" "<stddef.h>" "<stdlib.h>" "<string.h>")
    :types '((CLANG-TYPE
                :HASH 5790451697626571727
                :POINTER T
                :NAME "char"
                :SIZE 8)
             (CLANG-TYPE
                :HASH -2054504279541534951
                :POINTER NIL
                :NAME "char"
                :SIZE 1)
             (CLANG-TYPE
                :HASH 3615142211888308905
                :POINTER T
                :NAME "void"
                :SIZE 8))
    :macros '((CLANG-MACRO :HASH -342517378131665086 :NAME "ALLOCA" :BODY "ALLOCA alloca"))
    :code "data = NULL{
        /* FLAW: data is allocated on the stack and deallocated in the BadSink */
        dataBuffer = (char *)ALLOCA(100*sizeof(char));
        memset(dataBuffer, 'A', 100-1); /* fill with 'A's */
        dataBuffer[100-1] = '\\0'; /* null terminate */
        data = dataBuffer;
    }{
        dataCopy = data;
        data = dataCopy;
        printLine(data);
        /* POTENTIAL FLAW: Possibly deallocating memory allocated on the stack */
        free(data);
    }"))
\end{lstlisting}
\end{itemize}
\end{description}

\subsection*{Bug Template {\tt CWE617\_REACHABLE\_ASSERTION\_\_RAND\_01\_BAD\_INLINE}}
\begin{description}
\item[Definition:]~\newline
\begin{lstlisting}[language=lisp]
(define-scion CWE617_Reachable_Assertion__rand_01_bad_inline
  (make-instance 'clang-scion
    :name 'CWE617_Reachable_Assertion__rand_01_bad_inline
    :patches (list CWE617_Reachable_Assertion__rand_01_bad_inline_patch)))
\end{lstlisting}
\item[Patches:]~
\begin{itemize}
\item Definition for patch {\tt CWE617\_REACHABLE\_ASSERTION\_\_RAND\_01\_BAD\_INLINE\_PATCH}.
\begin{lstlisting}[language=lisp]
(defvar CWE617_Reachable_Assertion__rand_01_bad_inline_patch
  (make-instance 'clang-dynamic-patch
    :precondition NIL
    :cwe 617
    :conditional-code '(((((:CLASS . "BINARYOPERATOR") (:COUNTER . 5) (:FULL-STMT . T) (:INCLUDES)
   (:OPCODE . "=") (:SYN-CTX . "FULLSTMT")
  )
  "\"\""
  (((:CLASS . "DECLREFEXPR") (:COUNTER . 6) (:FULL-STMT) (:INCLUDES)
    (:OPCODE) (:SYN-CTX . "GENERIC")
   )
   "\"data\"")
  "\" = \""
  (((:CLASS . "UNARYOPERATOR") (:COUNTER . 7) (:FULL-STMT) (:INCLUDES)
    (:OPCODE . "-") (:SYN-CTX . "GENERIC")
   )
   "\"-\""
   (((:CLASS . "INTEGERLITERAL") (:COUNTER . 8) (:FULL-STMT) (:INCLUDES)
     (:OPCODE) (:SYN-CTX . "GENERIC")
    )
    "\"1\"")
   "\"\"")
  "\"\"") . T))
    :free-variables '(("data" "int" :-CONST :-REGISTER))
    :includes '("<assert.h>" "<stdlib.h>")
    :types '((CLANG-TYPE
                :HASH 2826451665740210303
                :POINTER NIL
                :NAME "void"
                :SIZE NIL)
             (CLANG-TYPE
                :HASH -760642589583846522
                :POINTER NIL
                :NAME "unsigned int"
                :SIZE 4)
             (CLANG-TYPE
                :HASH -1958391046879680490
                :POINTER NIL
                :NAME "int"
                :SIZE 4))
    :macros '((CLANG-MACRO :HASH 2308996158549424241 :NAME "URAND31"
                           :BODY "URAND31() (((unsigned)rand()<<30) ^ ((unsigned)rand()<<15) ^ rand())")
              (CLANG-MACRO :HASH 1124813122759813294 :NAME "RAND32"
                           :BODY "RAND32() ((int)(rand() & 1 ? URAND31() : -URAND31() - 1))")
              (CLANG-MACRO :HASH 560588087248213234 :NAME "ASSERT_VALUE" :BODY "ASSERT_VALUE 5"))
    :code "data = -1;
    data = RAND32();
    assert(data > ASSERT_VALUE);"))
\end{lstlisting}
\end{itemize}
\end{description}

\subsection*{Bug Template {\tt CWE665\_IMPROPER\_INITIALIZATION\_\_CHAR\_CAT\_31\_BAD\_INLINE}}
\begin{description}
\item[Definition:]~\newline
\begin{lstlisting}[language=lisp]
(define-scion CWE665_Improper_Initialization__char_cat_31_bad_inline
  (make-instance 'clang-scion
    :name 'CWE665_Improper_Initialization__char_cat_31_bad_inline
    :patches (list printLine_patch CWE665_Improper_Initialization__char_cat_31_bad_inline_patch)))
\end{lstlisting}
\item[Patches:]~
\begin{itemize}
\item Definition for patch {\tt PRINTLINE\_PATCH}.
\begin{lstlisting}[language=lisp]
(defvar printLine_patch
  (make-instance 'clang-static-patch
    :precondition (lambda (obj location)
  (and (= location 0)
       (not (member "printLine" (asts obj)
                    :test #'string=
                    :key [#'first #'ast-declares]))))
    :free-variables 'NIL
    :includes '("<stddef.h>" "<stdio.h>")
    :types '((CLANG-TYPE
                :HASH 3615142211888308905
                :POINTER T
                :NAME "void"
                :SIZE 8)
             (CLANG-TYPE
                :HASH -1944158543856436560
                :POINTER T
                :CONST T
                :NAME "char"
                :SIZE 8))
    :macros 'NIL
    :code "void printLine (const char * line)
{
    if(line != NULL) {
        printf(\"%s\\n\", line);
    }
}"))
\end{lstlisting}
\item Definition for patch {\tt CWE665\_IMPROPER\_INITIALIZATION\_\_CHAR\_CAT\_31\_BAD\_INLINE\_PATCH}.
\begin{lstlisting}[language=lisp]
(defvar CWE665_Improper_Initialization__char_cat_31_bad_inline_patch
  (make-instance 'clang-dynamic-patch
    :precondition NIL
    :cwe 665
    :conditional-code '()
    :free-variables '(("data" "*char" :-CONST :-REGISTER)
                      ("dataBuffer" "[100]char" :-CONST :-REGISTER)
                      ("dataCopy" "*char" :-CONST :-REGISTER)
                      ("source" "[100]char" :-CONST :-REGISTER))
    :includes '("<string.h>")
    :types '((CLANG-TYPE
                :ARRAY "[100]"
                :HASH 6253389274476629705
                :POINTER NIL
                :NAME "char"
                :SIZE 100)
             (CLANG-TYPE
                :HASH 5790451697626571727
                :POINTER T
                :NAME "char"
                :SIZE 8))
    :macros 'NIL
    :code "data = dataBuffer;{
        dataCopy = data;
        data = dataCopy;
        {
            
            memset(source, 'C', 100-1); /* fill with 'C's */
            source[100-1] = '\\0'; /* null terminate */
            /* POTENTIAL FLAW: If data is not initialized properly, strcat() may not function correctly */
            strcat(data, source);
            printLine(data);
        }
    }"))
\end{lstlisting}
\end{itemize}
\end{description}

\subsection*{Bug Template {\tt CWE674\_UNCONTROLLED\_RECURSION\_\_INFINITE\_RECURSIVE\_CALL\_01\_BAD\_INLINE}}
\begin{description}
\item[Definition:]~\newline
\begin{lstlisting}[language=lisp]
(define-scion CWE674_Uncontrolled_Recursion__infinite_recursive_call_01_bad_inline
  (make-instance 'clang-scion
    :name 'CWE674_Uncontrolled_Recursion__infinite_recursive_call_01_bad_inline
    :patches (list helperBad_inline_patch)))
\end{lstlisting}
\item[Patches:]~
\begin{itemize}
\item Definition for patch {\tt HELPERBAD\_INLINE\_PATCH}.
\begin{lstlisting}[language=lisp]
(defvar helperBad_inline_patch
  (make-instance 'clang-dynamic-patch
    :precondition NIL
    :cwe NIL
    :conditional-code '()
    :free-variables 'NIL
    :includes 'NIL
    :types 'NIL
    :macros 'NIL
    :code "helperBad()"))
\end{lstlisting}
\end{itemize}
\end{description}

\subsection*{Bug Template {\tt CWE675\_DUPLICATE\_OPERATIONS\_ON\_RESOURCE\_\_FOPEN\_31\_BAD\_INLINE}}
\begin{description}
\item[Definition:]~\newline
\begin{lstlisting}[language=lisp]
(define-scion CWE675_Duplicate_Operations_on_Resource__fopen_31_bad_inline
  (make-instance 'clang-scion
    :name 'CWE675_Duplicate_Operations_on_Resource__fopen_31_bad_inline
    :patches (list CWE675_Duplicate_Operations_on_Resource__fopen_31_bad_inline_patch)))
\end{lstlisting}
\item[Patches:]~
\begin{itemize}
\item Definition for patch {\tt CWE675\_DUPLICATE\_OPERATIONS\_ON\_RESOURCE\_\_FOPEN\_31\_BAD\_INLINE\_PATCH}.
\begin{lstlisting}[language=lisp]
(defvar CWE675_Duplicate_Operations_on_Resource__fopen_31_bad_inline_patch
  (make-instance 'clang-dynamic-patch
    :precondition NIL
    :cwe 675
    :conditional-code '(((((:CLASS . "BINARYOPERATOR") (:COUNTER . 5) (:FULL-STMT . T)
   (:INCLUDES "<stddef.h>") (:OPCODE . "=") (:SYN-CTX . "FULLSTMT")
  )
  "\"\""
  (((:CLASS . "DECLREFEXPR") (:COUNTER . 6) (:FULL-STMT) (:INCLUDES)
    (:OPCODE) (:SYN-CTX . "GENERIC")
   )
   "\"data\"")
  "\" = \""
  (((:CLASS . "MACROEXPANSION") (:COUNTER . 7) (:FULL-STMT) (:IN-MACRO-EXPANSION . T)
    (:INCLUDES "<stddef.h>") (:OPCODE) (:SYN-CTX . "GENERIC") (:TYPES 3615142211888308905)
   )
   "\"NULL\"")
  "\"\"") . T))
    :free-variables '(("data" "*FILE" :-CONST :-REGISTER) ("dataCopy" "*FILE" :-CONST :-REGISTER))
    :includes '("<stddef.h>" "<stdio.h>")
    :types '((CLANG-TYPE
                :COL 1
                :DECL NIL
                :FILE "/usr/include/bits/types/FILE.h"
                :LINE 7
                :HASH 3647496794580001440
                :I-FILE "<stdio.h>"
                :POINTER T
                :NAME "FILE"
                :SIZE 8)
             (CLANG-TYPE
                :HASH 3615142211888308905
                :POINTER T
                :NAME "void"
                :SIZE 8))
    :macros 'NIL
    :code "data = NULL;
    data = fopen(\"BadSource_fopen.txt\", \"w+\");
    fclose(data);
   {
        dataCopy = data;
        data = dataCopy;
        /* POTENTIAL FLAW: Close the file in the sink (it may have been closed in the Source) */
        fclose(data);
    }"))
\end{lstlisting}
\end{itemize}
\end{description}

\subsection*{Bug Template {\tt CWE680\_INTEGER\_OVERFLOW\_TO\_BUFFER\_OVERFLOW\_\_MALLOC\_RAND\_01\_BAD\_INLINE}}
\begin{description}
\item[Definition:]~\newline
\begin{lstlisting}[language=lisp]
(define-scion CWE680_Integer_Overflow_to_Buffer_Overflow__malloc_rand_01_bad_inline
  (make-instance 'clang-scion
    :name 'CWE680_Integer_Overflow_to_Buffer_Overflow__malloc_rand_01_bad_inline
    :patches (list printIntLine_patch CWE680_Integer_Overflow_to_Buffer_Overflow__malloc_rand_01_bad_inline_patch)))
\end{lstlisting}
\item[Patches:]~
\begin{itemize}
\item Definition for patch {\tt PRINTINTLINE\_PATCH}.
\begin{lstlisting}[language=lisp]
(defvar printIntLine_patch
  (make-instance 'clang-static-patch
    :precondition (lambda (obj location)
  (and (= location 0)
       (not (member "printIntLine" (asts obj)
                    :test #'string=
                    :key [#'first #'ast-declares]))))
    :free-variables 'NIL
    :includes '("<stdio.h>")
    :types '((CLANG-TYPE
                :HASH -1958391046879680490
                :POINTER NIL
                :NAME "int"
                :SIZE 4))
    :macros 'NIL
    :code "void printIntLine (int intNumber)
{
    printf(\"%d\\n\", intNumber);
}"))
\end{lstlisting}
\item Definition for patch\newline{\tt CWE680\_INTEGER\_OVERFLOW\_TO\_BUFFER\_OVERFLOW\_\_MALLOC\_RAND\_01\_BAD\_INLINE\_PATCH}.
\begin{lstlisting}[language=lisp]
(defvar CWE680_Integer_Overflow_to_Buffer_Overflow__malloc_rand_01_bad_inline_patch
  (make-instance 'clang-dynamic-patch
    :precondition NIL
    :cwe 680
    :conditional-code '(((((:CLASS . "BINARYOPERATOR") (:COUNTER . 5) (:FULL-STMT . T) (:INCLUDES)
   (:OPCODE . "=") (:SYN-CTX . "FULLSTMT")
  )
  "\"\""
  (((:CLASS . "DECLREFEXPR") (:COUNTER . 6) (:FULL-STMT) (:INCLUDES)
    (:OPCODE) (:SYN-CTX . "GENERIC")
   )
   "\"data\"")
  "\" = \""
  (((:CLASS . "UNARYOPERATOR") (:COUNTER . 7) (:FULL-STMT) (:INCLUDES)
    (:OPCODE . "-") (:SYN-CTX . "GENERIC")
   )
   "\"-\""
   (((:CLASS . "INTEGERLITERAL") (:COUNTER . 8) (:FULL-STMT) (:INCLUDES)
     (:OPCODE) (:SYN-CTX . "GENERIC")
    )
    "\"1\"")
   "\"\"")
  "\"\"") . T))
    :free-variables '(("data" "int" :-CONST :-REGISTER)
                      ("i" "size_t" :-CONST :-REGISTER)
                      ("intPointer" "*int" :-CONST :-REGISTER))
    :includes '("<stddef.h>" "<stdlib.h>")
    :types '((CLANG-TYPE
                :COL 1
                :DECL NIL
                :FILE "/usr/bin/../lib/clang/6.0.1/include/stddef.h"
                :LINE 62
                :HASH 764611252874068922
                :I-FILE "<stddef.h>"
                :POINTER NIL
                :NAME "size_t"
                :SIZE 8)
             (CLANG-TYPE
                :HASH 3615142211888308905
                :POINTER T
                :NAME "void"
                :SIZE 8)
             (CLANG-TYPE
                :HASH -1958391046879680490
                :POINTER NIL
                :NAME "int"
                :SIZE 4)
             (CLANG-TYPE
                :HASH -2241398076656181049
                :POINTER T
                :NAME "int"
                :SIZE 8)
             (CLANG-TYPE
                :HASH -760642589583846522
                :POINTER NIL
                :NAME "unsigned int"
                :SIZE 4))
    :macros '((CLANG-MACRO :HASH 2308996158549424241 :NAME "URAND31"
                           :BODY "URAND31() (((unsigned)rand()<<30) ^ ((unsigned)rand()<<15) ^ rand())")
              (CLANG-MACRO :HASH 1124813122759813294 :NAME "RAND32"
                           :BODY "RAND32() ((int)(rand() & 1 ? URAND31() : -URAND31() - 1))"))
    :code "data = -1;
    data = RAND32();
    {
        
        
        /* POTENTIAL FLAW: if data * sizeof(int) > SIZE_MAX, overflows to a small value
         * so that the for loop doing the initialization causes a buffer overflow */
        intPointer = (int*)malloc(data * sizeof(int));
        if (intPointer == NULL) {
            exit(-1);
        }
        for (i = 0; i < (size_t)data; i++) {
            intPointer[i] = 0; /* Potentially writes beyond the boundary of intPointer */
        }
        printIntLine(intPointer[0]);
        free(intPointer);
    }"))
\end{lstlisting}
\end{itemize}
\end{description}

\subsection*{Bug Template {\tt CWE685\_FUNCTION\_CALL\_WITH\_INCORRECT\_NUMBER\_OF\_ARGUMENTS\_\_BASIC\_01\_BAD\_INLINE}}
\begin{description}
\item[Definition:]~\newline
\begin{lstlisting}[language=lisp]
(define-scion CWE685_Function_Call_With_Incorrect_Number_of_Arguments__basic_01_bad_inline
  (make-instance 'clang-scion
    :name 'CWE685_Function_Call_With_Incorrect_Number_of_Arguments__basic_01_bad_inline
    :patches (list printLine_patch CWE685_Function_Call_With_Incorrect_Number_of_Arguments__basic_01_bad_inline_patch)))
\end{lstlisting}
\item[Patches:]~
\begin{itemize}
\item Definition for patch {\tt PRINTLINE\_PATCH}.
\begin{lstlisting}[language=lisp]
(defvar printLine_patch
  (make-instance 'clang-static-patch
    :precondition (lambda (obj location)
  (and (= location 0)
       (not (member "printLine" (asts obj)
                    :test #'string=
                    :key [#'first #'ast-declares]))))
    :free-variables 'NIL
    :includes '("<stddef.h>" "<stdio.h>")
    :types '((CLANG-TYPE
                :HASH 3615142211888308905
                :POINTER T
                :NAME "void"
                :SIZE 8)
             (CLANG-TYPE
                :HASH -1944158543856436560
                :POINTER T
                :CONST T
                :NAME "char"
                :SIZE 8))
    :macros 'NIL
    :code "void printLine (const char * line)
{
    if(line != NULL) {
        printf(\"%s\\n\", line);
    }
}"))
\end{lstlisting}
\item Definition for patch\newline{\tt CWE685\_FUNCTION\_CALL\_WITH\_INCORRECT\_NUMBER\_OF\_ARGUMENTS\_\_BASIC\_01\_BAD\_INLINE\_PATCH}.
\begin{lstlisting}[language=lisp]
(defvar CWE685_Function_Call_With_Incorrect_Number_of_Arguments__basic_01_bad_inline_patch
  (make-instance 'clang-dynamic-patch
    :precondition NIL
    :cwe 685
    :conditional-code '()
    :free-variables '(("dest" "[100]char" :-CONST :-REGISTER))
    :includes '("<stdio.h>")
    :types '((CLANG-TYPE
                :ARRAY "[100]"
                :HASH 6253389274476629705
                :POINTER NIL
                :NAME "char"
                :SIZE 100))
    :macros '((CLANG-MACRO :HASH -6999316518217383118 :NAME "SOURCE_STRING" :BODY "SOURCE_STRING \"AAA\"")
              (CLANG-MACRO :HASH 1185787598850764903 :NAME "DEST_SIZE" :BODY "DEST_SIZE 100 "))
    :code "{
        
        /* FLAW: Incorrect number of arguments */
        sprintf(dest, \"%s %s\", SOURCE_STRING);
        printLine(dest);
    }"))
\end{lstlisting}
\end{itemize}
\end{description}

\subsection*{Bug Template {\small {\tt CWE688\_FUNCTION\_CALL\_WITH\_INCORRECT\_VARIABLE\_OR\_REFERENCE\_AS\_ARGUMENT\_\_BASIC\_01\_BAD\_INLINE}}}
\begin{description}
\item[Definition:]~\newline
\begin{lstlisting}[language=lisp]
(define-scion CWE688_Function_Call_With_Incorrect_Variable_or_Reference_as_Argument__basic_01_bad_inline
  (make-instance 'clang-scion
    :name 'CWE688_Function_Call_With_Incorrect_Variable_or_Reference_as_Argument__basic_01_bad_inline
    :patches (list printLine_patch
                   CWE688_Function_Call_With_Incorrect_Variable_or_Reference_as_Argument__basic_01_bad_inline_patch)))
\end{lstlisting}
\item[Patches:]~
\begin{itemize}
\item Definition for patch {\tt PRINTLINE\_PATCH}.
\begin{lstlisting}[language=lisp]
(defvar printLine_patch
  (make-instance 'clang-static-patch
    :precondition (lambda (obj location)
  (and (= location 0)
       (not (member "printLine" (asts obj)
                    :test #'string=
                    :key [#'first #'ast-declares]))))
    :free-variables 'NIL
    :includes '("<stddef.h>" "<stdio.h>")
    :types '((CLANG-TYPE
                :HASH 3615142211888308905
                :POINTER T
                :NAME "void"
                :SIZE 8)
             (CLANG-TYPE
                :HASH -1944158543856436560
                :POINTER T
                :CONST T
                :NAME "char"
                :SIZE 8))
    :macros 'NIL
    :code "void printLine (const char * line)
{
    if(line != NULL) {
        printf(\"%s\\n\", line);
    }
}"))
\end{lstlisting}
\item Definition for patch\newline{\small {\tt CWE688\_FUNCTION\_CALL\_WITH\_INCORRECT\_VARIABLE\_OR\_REFERENCE\_AS\_ARGUMENT\_\_BASIC\_01\_BAD\_INLINE\_PATCH}}.
\begin{lstlisting}[language=lisp]
(defvar CWE688_Function_Call_With_Incorrect_Variable_or_Reference_as_Argument__basic_01_bad_inline_patch
  (make-instance 'clang-dynamic-patch
    :precondition NIL
    :cwe 688
    :conditional-code '()
    :free-variables '(("dest" "[100]char" :-CONST :-REGISTER) ("intFive" "int" :-CONST :-REGISTER))
    :includes '("<stdio.h>")
    :types '((CLANG-TYPE
                :HASH -1958391046879680490
                :POINTER NIL
                :NAME "int"
                :SIZE 4)
             (CLANG-TYPE
                :ARRAY "[100]"
                :HASH 6253389274476629705
                :POINTER NIL
                :NAME "char"
                :SIZE 100))
    :macros '((CLANG-MACRO :HASH -1390543107768948573 :NAME "DEST_SIZE" :BODY "DEST_SIZE 100"))
    :code "{
        
        intFive = 5;
        /* FLAW: int argument passed, expecting string argument */
        sprintf(dest, \"%s\", intFive);
        printLine(dest);
    }"))
\end{lstlisting}
\end{itemize}
\end{description}

\subsection*{Bug Template {\tt CWE690\_NULL\_DEREF\_FROM\_RETURN\_\_CHAR\_MALLOC\_01\_BAD\_INLINE}}
\begin{description}
\item[Definition:]~\newline
\begin{lstlisting}[language=lisp]
(define-scion CWE690_NULL_Deref_From_Return__char_malloc_01_bad_inline
  (make-instance 'clang-scion
    :name 'CWE690_NULL_Deref_From_Return__char_malloc_01_bad_inline
    :patches (list printLine_patch CWE690_NULL_Deref_From_Return__char_malloc_01_bad_inline_patch)))
\end{lstlisting}
\item[Patches:]~
\begin{itemize}
\item Definition for patch {\tt PRINTLINE\_PATCH}.
\begin{lstlisting}[language=lisp]
(defvar printLine_patch
  (make-instance 'clang-static-patch
    :precondition (lambda (obj location)
  (and (= location 0)
       (not (member "printLine" (asts obj)
                    :test #'string=
                    :key [#'first #'ast-declares]))))
    :free-variables 'NIL
    :includes '("<stddef.h>" "<stdio.h>")
    :types '((CLANG-TYPE
                :HASH 3615142211888308905
                :POINTER T
                :NAME "void"
                :SIZE 8)
             (CLANG-TYPE
                :HASH -1944158543856436560
                :POINTER T
                :CONST T
                :NAME "char"
                :SIZE 8))
    :macros 'NIL
    :code "void printLine (const char * line)
{
    if(line != NULL) {
        printf(\"%s\\n\", line);
    }
}"))
\end{lstlisting}
\item Definition for patch {\tt CWE690\_NULL\_DEREF\_FROM\_RETURN\_\_CHAR\_MALLOC\_01\_BAD\_INLINE\_PATCH}.
\begin{lstlisting}[language=lisp]
(defvar CWE690_NULL_Deref_From_Return__char_malloc_01_bad_inline_patch
  (make-instance 'clang-dynamic-patch
    :precondition NIL
    :cwe 690
    :conditional-code '(((((:CLASS . "BINARYOPERATOR") (:COUNTER . 5) (:FULL-STMT . T)
   (:INCLUDES "<stddef.h>") (:OPCODE . "=") (:SYN-CTX . "FULLSTMT")
  )
  "\"\""
  (((:CLASS . "DECLREFEXPR") (:COUNTER . 6) (:FULL-STMT) (:INCLUDES)
    (:OPCODE) (:SYN-CTX . "GENERIC")
   )
   "\"data\"")
  "\" = \""
  (((:CLASS . "MACROEXPANSION") (:COUNTER . 7) (:FULL-STMT) (:IN-MACRO-EXPANSION . T)
    (:INCLUDES "<stddef.h>") (:OPCODE) (:SYN-CTX . "GENERIC") (:TYPES 3615142211888308905)
   )
   "\"NULL\"")
  "\"\"") . T))
    :free-variables '(("data" "*char" :-CONST :-REGISTER))
    :includes '("<stddef.h>" "<stdlib.h>" "<string.h>")
    :types '((CLANG-TYPE
                :HASH -2054504279541534951
                :POINTER NIL
                :NAME "char"
                :SIZE 1)
             (CLANG-TYPE
                :HASH 5790451697626571727
                :POINTER T
                :NAME "char"
                :SIZE 8)
             (CLANG-TYPE
                :HASH 3615142211888308905
                :POINTER T
                :NAME "void"
                :SIZE 8))
    :macros 'NIL
    :code "data = NULL;
    data = (char *)malloc(20*sizeof(char));
    strcpy(data, \"Initialize\")printLine(data)free(data)"))
\end{lstlisting}
\end{itemize}
\end{description}

\subsection*{Bug Template {\tt CWE758\_UNDEFINED\_BEHAVIOR\_\_CHAR\_ALLOCA\_USE\_01\_BAD\_INLINE}}
\begin{description}
\item[Definition:]~\newline
\begin{lstlisting}[language=lisp]
(define-scion CWE758_Undefined_Behavior__char_alloca_use_01_bad_inline
  (make-instance 'clang-scion
    :name 'CWE758_Undefined_Behavior__char_alloca_use_01_bad_inline
    :patches (list printHexCharLine_patch CWE758_Undefined_Behavior__char_alloca_use_01_bad_inline_patch)))
\end{lstlisting}
\item[Patches:]~
\begin{itemize}
\item Definition for patch {\tt PRINTHEXCHARLINE\_PATCH}.
\begin{lstlisting}[language=lisp]
(defvar printHexCharLine_patch
  (make-instance 'clang-static-patch
    :precondition (lambda (obj location)
  (and (= location 0)
       (not (member "printHexCharLine" (asts obj)
                    :test #'string=
                    :key [#'first #'ast-declares]))))
    :free-variables 'NIL
    :includes '("<stdio.h>")
    :types '((CLANG-TYPE
                :HASH -2054504279541534951
                :POINTER NIL
                :NAME "char"
                :SIZE 1))
    :macros 'NIL
    :code "void printHexCharLine (char charHex)
{
    printf(\"%02x\\n\", charHex);
}"))
\end{lstlisting}
\item Definition for patch {\tt CWE758\_UNDEFINED\_BEHAVIOR\_\_CHAR\_ALLOCA\_USE\_01\_BAD\_INLINE\_PATCH}.
\begin{lstlisting}[language=lisp]
(defvar CWE758_Undefined_Behavior__char_alloca_use_01_bad_inline_patch
  (make-instance 'clang-dynamic-patch
    :precondition NIL
    :cwe 758
    :conditional-code '()
    :free-variables '(("pointer" "*char" :-CONST :-REGISTER) ("data" "char" :-CONST :-REGISTER))
    :includes '("<alloca.h>")
    :types '((CLANG-TYPE
                :HASH -2054504279541534951
                :POINTER NIL
                :NAME "char"
                :SIZE 1)
             (CLANG-TYPE
                :HASH 5790451697626571727
                :POINTER T
                :NAME "char"
                :SIZE 8))
    :macros '((CLANG-MACRO :HASH -342517378131665086 :NAME "ALLOCA" :BODY "ALLOCA alloca"))
    :code "{
        pointer = (char *)ALLOCA(sizeof(char));
        data = *pointer; /* FLAW: the value pointed to by pointer is undefined */
        printHexCharLine(data);
    }"))
\end{lstlisting}
\end{itemize}
\end{description}

\subsection*{Bug Template {\tt CWE761\_FREE\_POINTER\_NOT\_AT\_START\_OF\_BUFFER\_\_CHAR\_ENVIRONMENT\_01\_BAD\_INLINE}}
\begin{description}
\item[Definition:]~\newline
\begin{lstlisting}[language=lisp]
(define-scion CWE761_Free_Pointer_Not_at_Start_of_Buffer__char_environment_01_bad_inline
  (make-instance 'clang-scion
    :name 'CWE761_Free_Pointer_Not_at_Start_of_Buffer__char_environment_01_bad_inline
    :patches (list printLine_patch CWE761_Free_Pointer_Not_at_Start_of_Buffer__char_environment_01_bad_inline_patch)))
\end{lstlisting}
\item[Patches:]~
\begin{itemize}
\item Definition for patch {\tt PRINTLINE\_PATCH}.
\begin{lstlisting}[language=lisp]
(defvar printLine_patch
  (make-instance 'clang-static-patch
    :precondition (lambda (obj location)
  (and (= location 0)
       (not (member "printLine" (asts obj)
                    :test #'string=
                    :key [#'first #'ast-declares]))))
    :free-variables 'NIL
    :includes '("<stddef.h>" "<stdio.h>")
    :types '((CLANG-TYPE
                :HASH 3615142211888308905
                :POINTER T
                :NAME "void"
                :SIZE 8)
             (CLANG-TYPE
                :HASH -1944158543856436560
                :POINTER T
                :CONST T
                :NAME "char"
                :SIZE 8))
    :macros 'NIL
    :code "void printLine (const char * line)
{
    if(line != NULL) {
        printf(\"%s\\n\", line);
    }
}"))
\end{lstlisting}
\item Definition for patch\newline{\tt CWE761\_FREE\_POINTER\_NOT\_AT\_START\_OF\_BUFFER\_\_CHAR\_ENVIRONMENT\_01\_BAD\_INLINE\_PATCH}.
\begin{lstlisting}[language=lisp]
(defvar CWE761_Free_Pointer_Not_at_Start_of_Buffer__char_environment_01_bad_inline_patch
  (make-instance 'clang-dynamic-patch
    :precondition NIL
    :cwe 761
    :conditional-code '()
    :free-variables '(("data" "*char" :-CONST :-REGISTER)
                      ("dataLen" "size_t" :-CONST :-REGISTER)
                      ("environment" "*char" :-CONST :-REGISTER))
    :includes '("<stddef.h>" "<stdlib.h>" "<string.h>")
    :types '((CLANG-TYPE
                :HASH 3615142211888308905
                :POINTER T
                :NAME "void"
                :SIZE 8)
             (CLANG-TYPE
                :HASH 5790451697626571727
                :POINTER T
                :NAME "char"
                :SIZE 8)
             (CLANG-TYPE
                :COL 1
                :DECL NIL
                :FILE "/usr/bin/../lib/clang/6.0.1/include/stddef.h"
                :LINE 62
                :HASH 764611252874068922
                :I-FILE "<stddef.h>"
                :POINTER NIL
                :NAME "size_t"
                :SIZE 8)
             (CLANG-TYPE
                :HASH -2054504279541534951
                :POINTER NIL
                :NAME "char"
                :SIZE 1))
    :macros '((CLANG-MACRO :HASH -8515871080290371086 :NAME "SEARCH_CHAR" :BODY "SEARCH_CHAR 'S'")
              (CLANG-MACRO :HASH -4912265186542351092 :NAME "ENV_VARIABLE" :BODY "ENV_VARIABLE \"ADD\"")
              (CLANG-MACRO :HASH 2645724798783031398 :NAME "GETENV" :BODY "GETENV getenv"))
    :code "data = (char *)malloc(100*sizeof(char))if (data == NULL) {
        exit(-1);
    }data[0] = '\\0'{
        /* Append input from an environment variable to data */
        dataLen = strlen(data);
        environment = GETENV(ENV_VARIABLE);
        /* If there is data in the environment variable */
        if (environment != NULL) {
            /* POTENTIAL FLAW: Read data from an environment variable */
            strncat(data+dataLen, environment, 100-dataLen-1);
        }
    }for (; *data != '\\0'; data++) {
        if (*data == SEARCH_CHAR) {
            printLine(\"We have a match!\");
            break;
        }
    }free(data)"))
\end{lstlisting}
\end{itemize}
\end{description}

\subsection*{Bug Template {\tt CWE773\_MISSING\_REFERENCE\_TO\_ACTIVE\_FILE\_DESCRIPTOR\_OR\_HANDLE\_\_FOPEN\_31\_BAD\_INLINE}}
\begin{description}
\item[Definition:]~\newline
\begin{lstlisting}[language=lisp]
(define-scion CWE773_Missing_Reference_to_Active_File_Descriptor_or_Handle__fopen_31_bad_inline
  (make-instance 'clang-scion
    :name 'CWE773_Missing_Reference_to_Active_File_Descriptor_or_Handle__fopen_31_bad_inline
    :patches (list CWE773_Missing_Reference_to_Active_File_Descriptor_or_Handle__fopen_31_bad_inline_patch)))
\end{lstlisting}
\item[Patches:]~
\begin{itemize}
\item Definition for patch\newline{\tt CWE773\_MISSING\_REFERENCE\_TO\_ACTIVE\_FILE\_DESCRIPTOR\_OR\_HANDLE\_\_FOPEN\_31\_BAD\_INLINE\_PATCH}.
\begin{lstlisting}[language=lisp]
(defvar CWE773_Missing_Reference_to_Active_File_Descriptor_or_Handle__fopen_31_bad_inline_patch
  (make-instance 'clang-dynamic-patch
    :precondition NIL
    :cwe 773
    :conditional-code '(((((:CLASS . "BINARYOPERATOR") (:COUNTER . 5) (:FULL-STMT . T)
   (:INCLUDES "<stddef.h>") (:OPCODE . "=") (:SYN-CTX . "FULLSTMT")
  )
  "\"\""
  (((:CLASS . "DECLREFEXPR") (:COUNTER . 6) (:FULL-STMT) (:INCLUDES)
    (:OPCODE) (:SYN-CTX . "GENERIC")
   )
   "\"data\"")
  "\" = \""
  (((:CLASS . "MACROEXPANSION") (:COUNTER . 7) (:FULL-STMT) (:IN-MACRO-EXPANSION . T)
    (:INCLUDES "<stddef.h>") (:OPCODE) (:SYN-CTX . "GENERIC") (:TYPES 3615142211888308905)
   )
   "\"NULL\"")
  "\"\"") . T)((((:CLASS . "BINARYOPERATOR") (:COUNTER) (:FULL-STMT . T) (:INCLUDES)
   (:OPCODE . "=") (:SYN-CTX . "FULLSTMT")
  )
  (((:CLASS . "IMPLICITCASTEXPR") (:COUNTER) (:EXPR-TYPE . 3647496794580001440) (:FULL-STMT)
    (:INCLUDES) (:OPCODE) (:SYN-CTX . "GENERIC")
   )
   (((:CLASS . "DECLREFEXPR") (:COUNTER) (:EXPR-TYPE . 3647496794580001440) (:FULL-STMT)
     (:INCLUDES) (:OPCODE) (:SYN-CTX . "GENERIC")
    )
    "\"data\""))
  "\" = \""
  (((:CLASS . "IMPLICITCASTEXPR") (:COUNTER . 29) (:FULL-STMT) (:INCLUDES)
    (:OPCODE) (:SYN-CTX . "GENERIC")
   )
   "\"\""
   (((:CLASS . "DECLREFEXPR") (:COUNTER . 30) (:FULL-STMT) (:INCLUDES)
     (:OPCODE) (:SYN-CTX . "GENERIC")
    )
    "\"dataCopy\"")
   "\"\"")) . T))
    :free-variables '(("data" "*FILE" :-CONST :-REGISTER) ("dataCopy" "*FILE" :-CONST :-REGISTER))
    :includes '("<stddef.h>" "<stdio.h>")
    :types '((CLANG-TYPE
                :HASH 3615142211888308905
                :POINTER T
                :NAME "void"
                :SIZE 8)
             (CLANG-TYPE
                :COL 1
                :DECL NIL
                :FILE "/usr/include/bits/types/FILE.h"
                :LINE 7
                :HASH 3647496794580001440
                :I-FILE "<stdio.h>"
                :POINTER T
                :NAME "FILE"
                :SIZE 8))
    :macros 'NIL
    :code "data = NULL;
    data = fopen(\"BadSource_fopen.txt\", \"w+\");
    {
        dataCopy = data;
        data = dataCopy;
        /* FLAW: Point data to another file handle without closing the handle from the source */
        data = fopen(\"BadSink_fopen.txt\", \"w+\");
        /* avoid incidental for not closing the file handle */
        if (data != NULL) {
            fclose(data);
        }
    }"))
\end{lstlisting}
\end{itemize}
\end{description}

\subsection*{Bug Template {\tt CWE775\_MISSING\_RELEASE\_OF\_FILE\_DESCRIPTOR\_OR\_HANDLE\_\_OPEN\_NO\_CLOSE\_31\_BAD\_INLINE}}
\begin{description}
\item[Definition:]~\newline
\begin{lstlisting}[language=lisp]
(define-scion CWE775_Missing_Release_of_File_Descriptor_or_Handle__open_no_close_31_bad_inline
  (make-instance 'clang-scion
    :name 'CWE775_Missing_Release_of_File_Descriptor_or_Handle__open_no_close_31_bad_inline
    :patches (list CWE775_Missing_Release_of_File_Descriptor_or_Handle__open_no_close_31_bad_inline_patch)))
\end{lstlisting}
\item[Patches:]~
\begin{itemize}
\item Definition for patch\newline{\tt CWE775\_MISSING\_RELEASE\_OF\_FILE\_DESCRIPTOR\_OR\_HANDLE\_\_OPEN\_NO\_CLOSE\_31\_BAD\_INLINE\_PATCH}.
\begin{lstlisting}[language=lisp]
(defvar CWE775_Missing_Release_of_File_Descriptor_or_Handle__open_no_close_31_bad_inline_patch
  (make-instance 'clang-dynamic-patch
    :precondition NIL
    :cwe 775
    :conditional-code '(((((:CLASS . "BINARYOPERATOR") (:COUNTER . 5) (:FULL-STMT . T) (:INCLUDES)
   (:OPCODE . "=") (:SYN-CTX . "FULLSTMT")
  )
  "\"\""
  (((:CLASS . "DECLREFEXPR") (:COUNTER . 6) (:FULL-STMT) (:INCLUDES)
    (:OPCODE) (:SYN-CTX . "GENERIC")
   )
   "\"data\"")
  "\" = \""
  (((:CLASS . "UNARYOPERATOR") (:COUNTER . 7) (:FULL-STMT) (:INCLUDES)
    (:OPCODE . "-") (:SYN-CTX . "GENERIC")
   )
   "\"-\""
   (((:CLASS . "INTEGERLITERAL") (:COUNTER . 8) (:FULL-STMT) (:INCLUDES)
     (:OPCODE) (:SYN-CTX . "GENERIC")
    )
    "\"1\"")
   "\"\"")
  "\"\"") . T))
    :free-variables '(("data" "int" :-CONST :-REGISTER) ("dataCopy" "int" :-CONST :-REGISTER))
    :includes '("<fcntl.h>" "<sys/stat.h>")
    :types '((CLANG-TYPE
                :HASH -1958391046879680490
                :POINTER NIL
                :NAME "int"
                :SIZE 4))
    :macros '((CLANG-MACRO :HASH 1558538643793173296 :NAME "OPEN" :BODY "OPEN open")
              (CLANG-MACRO :HASH -7379358396012845812 :NAME "CLOSE" :BODY "CLOSE close"))
    :code "data = -1;
    data = OPEN(\"BadSource_open.txt\", O_RDWR|O_CREAT, S_IREAD|S_IWRITE);
    {
        dataCopy = data;
        data = dataCopy;
        /* FLAW: No attempt to close the file */
        ; /* empty statement needed for some flow variants */
    }"))
\end{lstlisting}
\end{itemize}
\end{description}

\subsection*{Bug Template {\tt CWE789\_UNCONTROLLED\_MEM\_ALLOC\_\_MALLOC\_CHAR\_RAND\_01\_BAD\_INLINE}}
\begin{description}
\item[Definition:]~\newline
\begin{lstlisting}[language=lisp]
(define-scion CWE789_Uncontrolled_Mem_Alloc__malloc_char_rand_01_bad_inline
  (make-instance 'clang-scion
    :name 'CWE789_Uncontrolled_Mem_Alloc__malloc_char_rand_01_bad_inline
    :patches (list printLine_patch CWE789_Uncontrolled_Mem_Alloc__malloc_char_rand_01_bad_inline_patch)))
\end{lstlisting}
\item[Patches:]~
\begin{itemize}
\item Definition for patch {\tt PRINTLINE\_PATCH}.
\begin{lstlisting}[language=lisp]
(defvar printLine_patch
  (make-instance 'clang-static-patch
    :precondition (lambda (obj location)
  (and (= location 0)
       (not (member "printLine" (asts obj)
                    :test #'string=
                    :key [#'first #'ast-declares]))))
    :free-variables 'NIL
    :includes '("<stddef.h>" "<stdio.h>")
    :types '((CLANG-TYPE
                :HASH 3615142211888308905
                :POINTER T
                :NAME "void"
                :SIZE 8)
             (CLANG-TYPE
                :HASH -1944158543856436560
                :POINTER T
                :CONST T
                :NAME "char"
                :SIZE 8))
    :macros 'NIL
    :code "void printLine (const char * line)
{
    if(line != NULL) {
        printf(\"%s\\n\", line);
    }
}"))
\end{lstlisting}
\item Definition for patch {\tt CWE789\_UNCONTROLLED\_MEM\_ALLOC\_\_MALLOC\_CHAR\_RAND\_01\_BAD\_INLINE\_PATCH}.
\begin{lstlisting}[language=lisp]
(defvar CWE789_Uncontrolled_Mem_Alloc__malloc_char_rand_01_bad_inline_patch
  (make-instance 'clang-dynamic-patch
    :precondition NIL
    :cwe 789
    :conditional-code '(((((:CLASS . "BINARYOPERATOR") (:COUNTER . 5) (:FULL-STMT . T) (:INCLUDES)
   (:OPCODE . "=") (:SYN-CTX . "FULLSTMT")
  )
  "\"\""
  (((:CLASS . "DECLREFEXPR") (:COUNTER . 6) (:FULL-STMT) (:INCLUDES)
    (:OPCODE) (:SYN-CTX . "GENERIC")
   )
   "\"data\"")
  "\" = \""
  (((:CLASS . "IMPLICITCASTEXPR") (:COUNTER . 7) (:FULL-STMT) (:INCLUDES)
    (:OPCODE) (:SYN-CTX . "GENERIC")
   )
   "\"\""
   (((:CLASS . "INTEGERLITERAL") (:COUNTER . 8) (:FULL-STMT) (:INCLUDES)
     (:OPCODE) (:SYN-CTX . "GENERIC")
    )
    "\"0\"")
   "\"\"")
  "\"\"") . T))
    :free-variables '(("data" "size_t" :-CONST :-REGISTER) ("myString" "*char" :-CONST :-REGISTER))
    :includes '("<stddef.h>" "<stdlib.h>" "<string.h>")
    :types '((CLANG-TYPE
                :HASH 3615142211888308905
                :POINTER T
                :NAME "void"
                :SIZE 8)
             (CLANG-TYPE
                :HASH -2054504279541534951
                :POINTER NIL
                :NAME "char"
                :SIZE 1)
             (CLANG-TYPE
                :HASH 5790451697626571727
                :POINTER T
                :NAME "char"
                :SIZE 8)
             (CLANG-TYPE
                :COL 1
                :DECL NIL
                :FILE "/usr/bin/../lib/clang/6.0.1/include/stddef.h"
                :LINE 62
                :HASH 764611252874068922
                :I-FILE "<stddef.h>"
                :POINTER NIL
                :NAME "size_t"
                :SIZE 8))
    :macros '((CLANG-MACRO :HASH 1808983277519718612 :NAME "HELLO_STRING" :BODY "HELLO_STRING \"hello\""))
    :code "data = 0;
    data = rand();
    {
        
        /* POTENTIAL FLAW: No MAXIMUM limitation for memory allocation, but ensure data is large enough
         * for the strcpy() function to not cause a buffer overflow */
        /* INCIDENTAL FLAW: The source could cause a type overrun in data or in the memory allocation */
        if (data > strlen(HELLO_STRING)) {
            myString = (char *)malloc(data*sizeof(char));
            if (myString == NULL) {
                exit(-1);
            }
            /* Copy a small string into myString */
            strcpy(myString, HELLO_STRING);
            printLine(myString);
            free(myString);
        } else {
            printLine(\"Input is less than the length of the source string\");
        }
    }"))
\end{lstlisting}
\end{itemize}
\end{description}

\subsection*{Bug Template {\tt CWE78\_OS\_COMMAND\_INJECTION\_\_CHAR\_ENVIRONMENT\_EXECL\_01\_BAD\_INLINE}}
\begin{description}
\item[Definition:]~\newline
\begin{lstlisting}[language=lisp]
(define-scion CWE78_OS_Command_Injection__char_environment_execl_01_bad_inline
  (make-instance 'clang-scion
    :name 'CWE78_OS_Command_Injection__char_environment_execl_01_bad_inline
    :patches (list CWE78_OS_Command_Injection__char_environment_execl_01_bad_inline_patch)))
\end{lstlisting}
\item[Patches:]~
\begin{itemize}
\item Definition for patch {\tt CWE78\_OS\_COMMAND\_INJECTION\_\_CHAR\_ENVIRONMENT\_EXECL\_01\_BAD\_INLINE\_PATCH}.
\begin{lstlisting}[language=lisp]
(defvar CWE78_OS_Command_Injection__char_environment_execl_01_bad_inline_patch
  (make-instance 'clang-dynamic-patch
    :precondition NIL
    :cwe 78
    :conditional-code '()
    :free-variables '(("data" "*char" :-CONST :-REGISTER)
                      ("dataBuffer" "[100]char" :-CONST :-REGISTER)
                      ("dataLen" "size_t" :-CONST :-REGISTER)
                      ("environment" "*char" :-CONST :-REGISTER))
    :includes '("<stddef.h>" "<stdlib.h>" "<string.h>" "<unistd.h>")
    :types '((CLANG-TYPE
                :HASH 3615142211888308905
                :POINTER T
                :NAME "void"
                :SIZE 8)
             (CLANG-TYPE
                :HASH 5790451697626571727
                :POINTER T
                :NAME "char"
                :SIZE 8)
             (CLANG-TYPE
                :COL 1
                :DECL NIL
                :FILE "/usr/bin/../lib/clang/6.0.1/include/stddef.h"
                :LINE 62
                :HASH 764611252874068922
                :I-FILE "<stddef.h>"
                :POINTER NIL
                :NAME "size_t"
                :SIZE 8)
             (CLANG-TYPE
                :ARRAY "[100]"
                :HASH 6253389274476629705
                :POINTER NIL
                :NAME "char"
                :SIZE 100))
    :macros '((CLANG-MACRO :HASH 9084927035900116674 :NAME "COMMAND_ARG3" :BODY "COMMAND_ARG3 data")
              (CLANG-MACRO :HASH 4633345150827363949 :NAME "COMMAND_ARG1" :BODY "COMMAND_ARG1 \"-c\"")
              (CLANG-MACRO :HASH -2565974004529164926 :NAME "COMMAND_INT_PATH" :BODY "COMMAND_INT_PATH \"/bin/sh\"")
              (CLANG-MACRO :HASH -2425351531048995248 :NAME "EXECL" :BODY "EXECL execl")
              (CLANG-MACRO :HASH -4912265186542351092 :NAME "ENV_VARIABLE" :BODY "ENV_VARIABLE \"ADD\"")
              (CLANG-MACRO :HASH 2645724798783031398 :NAME "GETENV" :BODY "GETENV getenv")
              (CLANG-MACRO :HASH 1512811662678344236 :NAME "COMMAND_ARG2" :BODY "COMMAND_ARG2 \"ls \"")
              (CLANG-MACRO :HASH -2047303224589684749 :NAME "COMMAND_INT" :BODY "COMMAND_INT \"sh\""))
    :code "dataBuffer = COMMAND_ARG2data = dataBuffer{
        /* Append input from an environment variable to data */
        dataLen = strlen(data);
        environment = GETENV(ENV_VARIABLE);
        /* If there is data in the environment variable */
        if (environment != NULL) {
            /* POTENTIAL FLAW: Read data from an environment variable */
            strncat(data+dataLen, environment, 100-dataLen-1);
        }
    }EXECL(COMMAND_INT_PATH, COMMAND_INT_PATH, COMMAND_ARG1, COMMAND_ARG3, NULL)"))
\end{lstlisting}
\end{itemize}
\end{description}

\subsection*{Bug Template {\tt CWE835\_INFINITE\_LOOP\_\_DO\_01\_BAD\_INLINE}}
\begin{description}
\item[Definition:]~\newline
\begin{lstlisting}[language=lisp]
(define-scion CWE835_Infinite_Loop__do_01_bad_inline
  (make-instance 'clang-scion
    :name 'CWE835_Infinite_Loop__do_01_bad_inline
    :patches (list printIntLine_patch CWE835_Infinite_Loop__do_01_bad_inline_patch)))
\end{lstlisting}
\item[Patches:]~
\begin{itemize}
\item Definition for patch {\tt PRINTINTLINE\_PATCH}.
\begin{lstlisting}[language=lisp]
(defvar printIntLine_patch
  (make-instance 'clang-static-patch
    :precondition (lambda (obj location)
  (and (= location 0)
       (not (member "printIntLine" (asts obj)
                    :test #'string=
                    :key [#'first #'ast-declares]))))
    :free-variables 'NIL
    :includes '("<stdio.h>")
    :types '((CLANG-TYPE
                :HASH -1958391046879680490
                :POINTER NIL
                :NAME "int"
                :SIZE 4))
    :macros 'NIL
    :code "void printIntLine (int intNumber)
{
    printf(\"%d\\n\", intNumber);
}"))
\end{lstlisting}
\item Definition for patch {\tt CWE835\_INFINITE\_LOOP\_\_DO\_01\_BAD\_INLINE\_PATCH}.
\begin{lstlisting}[language=lisp]
(defvar CWE835_Infinite_Loop__do_01_bad_inline_patch
  (make-instance 'clang-dynamic-patch
    :precondition NIL
    :cwe 835
    :conditional-code '()
    :free-variables '(("i" "int" :-CONST :-REGISTER))
    :includes 'NIL
    :types '((CLANG-TYPE
                :HASH -1958391046879680490
                :POINTER NIL
                :NAME "int"
                :SIZE 4))
    :macros 'NIL
    :code "i = 0do {
        printIntLine(i);
        i = (i + 1) % 256;
    } while(i >= 0)"))
\end{lstlisting}
\end{itemize}
\end{description}

\subsection*{Bug Template {\tt CWE843\_TYPE\_CONFUSION\_\_CHAR\_01\_BAD\_INLINE}}
\begin{description}
\item[Definition:]~\newline
\begin{lstlisting}[language=lisp]
(define-scion CWE843_Type_Confusion__char_01_bad_inline
  (make-instance 'clang-scion
    :name 'CWE843_Type_Confusion__char_01_bad_inline
    :patches (list printIntLine_patch CWE843_Type_Confusion__char_01_bad_inline_patch)))
\end{lstlisting}
\item[Patches:]~
\begin{itemize}
\item Definition for patch {\tt PRINTINTLINE\_PATCH}.
\begin{lstlisting}[language=lisp]
(defvar printIntLine_patch
  (make-instance 'clang-static-patch
    :precondition (lambda (obj location)
  (and (= location 0)
       (not (member "printIntLine" (asts obj)
                    :test #'string=
                    :key [#'first #'ast-declares]))))
    :free-variables 'NIL
    :includes '("<stdio.h>")
    :types '((CLANG-TYPE
                :HASH -1958391046879680490
                :POINTER NIL
                :NAME "int"
                :SIZE 4))
    :macros 'NIL
    :code "void printIntLine (int intNumber)
{
    printf(\"%d\\n\", intNumber);
}"))
\end{lstlisting}
\item Definition for patch {\tt CWE843\_TYPE\_CONFUSION\_\_CHAR\_01\_BAD\_INLINE\_PATCH}.
\begin{lstlisting}[language=lisp]
(defvar CWE843_Type_Confusion__char_01_bad_inline_patch
  (make-instance 'clang-dynamic-patch
    :precondition NIL
    :cwe 843
    :conditional-code '()
    :free-variables '(("data" "*void" :-CONST :-REGISTER) ("charBuffer" "char" :-CONST :-REGISTER))
    :includes '("<stddef.h>")
    :types '((CLANG-TYPE
                :HASH -2241398076656181049
                :POINTER T
                :NAME "int"
                :SIZE 8)
             (CLANG-TYPE
                :HASH -2054504279541534951
                :POINTER NIL
                :NAME "char"
                :SIZE 1)
             (CLANG-TYPE
                :HASH 3615142211888308905
                :POINTER T
                :NAME "void"
                :SIZE 8))
    :macros 'NIL
    :code "data = NULL{
        /* FLAW: Point data to a char */
        charBuffer = 'a';
        data = &charBuffer;
    }printIntLine(*((int*)data))"))
\end{lstlisting}
\end{itemize}
\end{description}
